# Supplementary material for: Adding Circumscription to Decidable Fragments of First-Order Logic: A Complexity Rollercoaster
Source: arXiv:2407.20822 source file (2024-07-30)
Supplement: Supplementary file 1 [file appendix.tex]

\section{Proofs for Section~\ref{subsect:fundamental}}

To complete the proof of Proposition~\ref{prop:nonom}, it suffices
to show the following.
\begin{lemma}
  $\Circ(\Kmc) \models q(\bar a)$ iff 
  $\mn{Circ}_{\mn{CP}'}(\Kmc') \models q'(\bar a)$ for all 
  $\bar a \in \mn{ind}(\Amc)$. 
\end{lemma}
\begin{proof}
  First assume that $\Circ(\Kmc) \not\models q(\bar a)$. Then there is
  a model \Imc of $\Circ(\Kmc)$ such that $\Imc\not\models q(\bar a)$.
  Let $\Imc'$ be defined like \Imc except that
  $A_a^{\Imc'}=B_a^{\Imc'}= \{a \}$ and $D_a^{\Imc'}=\emptyset$ for
  all $a \in N$. It is readily checked that $\Imc'$ is a model of
    $\mn{Circ}_{\mn{CP}'}(\Kmc')$ and that $\Imc' \not \models q'(\bar
    a)$.

    Now assume that
    $\mn{Circ}_{\mn{CP}'}(\Kmc')\not\models q'(\bar a)$. Then there is
    a model $\Imc'$ of $\mn{Circ}_{\mn{CP}'}(\Kmc')$ with
    $\Imc' \not\models q'(\bar a)$. Since $\Imc'$ is a model of
    $\Amc'$, we have $a \in B_a^{\Imc'}$ for all $a \in N$. Moreover,
    if $\{a\} \subsetneq B_a^{\Imc'}$, then we can find a model
    $\Jmc'$ of $\mn{Circ}_{\mn{CP}'}(\Kmc')$ with
    $\Jmc' <_{\CP'} \Imc'$ by setting $B_a^{\Jmc'}=\{a\}$ and
    $D_a^{\Jmc'}=A_a^{\Imc'} \setminus \{ a \}$. This contradicts the
    minimality of $\Imc'$, and, consequently, we must have
    $B_a^{\Imc'} = \{a\}$. But then also $A_a^{\Imc'} = \{ a \}$ since
    $A(a) \in \Amc'$, $A_a \sqcap \neg B_a \sqsubseteq D_a \in \Tmc'$,
    and the disjunct $\exists y \, D_a(y)$ is not satisfied in
    $\Imc'$. It can be verified that, consequently, $\Imc'$ is also a
    model of $\Circ(\Kmc)$, and we are done.
\end{proof}

\lemnormalform*
We omit a proof of the above lemma, which is entirely standard. The same normal form was used for \ALCHI, e.g., in \cite{maniere:thesis}.

\lemmafive*
\begin{proof}
	Assume to the contrary that \Jmc is not a model of $\Circ(\Kmc)$.
	As \Jmc is a model of \Kmc by prerequisite, there is thus a model $\Jmc'$ of \Kmc with $\Jmc' <_\CP \Jmc$.	
	To derive a contradiction, we construct a model $\Imc'$ of \Kmc with $\Delta^{\Imc'} = \Delta^{\Imc}$ and show that $\Imc' <_\CP \Imc$.
	For each type $t \in \mn{TP}_{\overline{\mn{core}}}(\Imc)$,	let
	$$
	\begin{array}{rcl}
		D_t & = & \{ d \in \Delta^\Imc \setminus \mn{ind}(\Amc) \mid \mn{tp}_\Imc(d)=t
		\}   \\[1mm]
		S_t & = & \{ \mn{tp}_{\Jmc'}(d) \mid d \in \Delta^\Jmc: \mn{tp}_\Jmc(d)=t \}.
	\end{array}
	$$
        We have
        \begin{itemize}
        \item $|D_t| \geq |\mn{TP}(\Tmc)|$ by definition of
          $\noncoretypesof{\I}$ and
        \item  $|S_t| \leq |\mn{TP}(\Tmc)|$, by definition of $S_t$.
        \end{itemize}
	Moreover, the `$\supseteq$'	direction of Point~2 implies $S_t \neq \emptyset$.
	We can thus	find a surjective function $\pi_t: D_t \rightarrow S_t$.
	
	Let $\pi$ be the function that is obtained as the union of 
        the (domain disjoint) functions $\pi_t$, for all $t \in
        \mn{TP}_{\overline{\mn{core}}}(\Imc)$.
	By definition of $\pi$ and of $\Delta^\Imc_\mn{core}$, the domain of $\pi$ is 
        $$\Delta^\Imc \setminus 
	\big (\Delta^\Imc_\mn{core} \cup \mn{ind}(\Amc) \big ).$$
        Now consider the range of $\pi$.
        By Point~1 and the `$\subseteq$' direction of Point~2,
        $\mn{tp}_\Jmc(d) \in  \mn{TP}_{\overline{\mn{core}}}(\Imc)$
        iff
        $d \notin \Delta^\Imc_\mn{core}$. By definition, the range
        of $\pi$ is thus 
	$$\{ \mn{tp}_{\Jmc'}(d) \mid d \in \Delta^\Jmc
        \setminus \Delta^\Imc_\mn{core}\}.$$
        %
        % and all elements from this set are actually hit, that is, $\pi$ is
        % surjective.

	Extend $\pi$ to domain $\Delta^\Imc$ by setting $\pi(d)=\mn{tp}_{\Jmc'}(d)$ for all
	$d \in \Delta^\Imc_\mn{core} \cup \mn{ind}(\Amc)$.
	It is easy to see that now, $\pi$ is a surjective function from $\Delta^\Imc$ to $\mn{TP}(\Jmc')$.
	We construct an interpretation $\Imc'$ as follows:
	\begin{align*}
		\Delta^{\Imc'} & =	\Delta^\Imc                                                                               \\
%		\istyle{a}^{\Imc'}      & =	\istyle{a} \\
		\cstyle{A}^{\Imc'}      & =	\{ d \in
		\Delta^{\Imc'}\mid \cstyle{A} \in
		\pi(d) \}
%		\cup \{ a \in
%		\mn{ind}(\Amc) \mid A(a)
%		\in \Amc \}                                                                                                 
		\\
		\rstyle{r}^{\Imc'}      & =	\{ (d,e) \in \Delta^{\Imc'}\times \Delta^{\Imc'} \mid \pi(d) \rightsquigarrow_\rstyle{r} \pi(e) \} 
	\end{align*}
        for all concept names $A$ and role names $r$.  Notice that
        $\typeinof{\I'}{d} = \pi(d)$, hence
        $\types(\I') \subseteq \types(\Jmc')$.  We first show that
        $\Imc'$ is a model of \Kmc by considering each possible shape
        of assertions and inclusion (recall that $\tbox$ is {in}
        normal form):
	\begin{itemize}
		
		\item{$\conceptassertion{A}{a}$.}
		Since $\Jmc'$ is a model of $\kb$, we have $\istyle{a} \in \cstyle{A}^{\Jmc'}$, hence $\cstyle{A} \in \typeinof{\Jmc'}{\istyle{a}}$.
		By definition of $\pi$, we have $\pi(\istyle{a}) = \typeinof{\Jmc'}{\istyle{a}}$, hence $\cstyle{A} \in \pi(\istyle{a})$.
		The definition of $\cstyle{A}^{\I'}$ yields $\istyle{a} \in \cstyle{A}^{\I'}$.
		
		\item{$\roleassertion{r}{a}{b}$.}
		Since $\Jmc'$ is a model of $\kb$, we have $(\istyle{a}, \istyle{b}) \in \rstyle{r}^{\Jmc'}$, hence $\typeinof{\Jmc'}{\istyle{a}} \legitsucc_\rstyle{r} \typeinof{\Jmc'}{\istyle{b}}$.
		By definition of $\pi$, we have $\pi(\istyle{a}) = \typeinof{\Jmc'}{\istyle{a}}$ and $\pi(\istyle{b}) = \typeinof{\Jmc'}{\istyle{b}}$.
		The definition of $\rstyle{r}^{\I'}$ yields $(\istyle{a}, \istyle{b}) \in \rstyle{r}^{\I'}$.
		
		\item
		Satisfaction of CIs of shape $\axtop$, $\axand$,
                $\axnotright$ and $\axnotleft$ immediately follows
                from $\types(\I') \subseteq \types(\Jmc')$ and $\Jmc'$
                being a model of \Tmc.
		
		\item{$\axexistsright$.}
		Let $d \in \cstyle{A}^{\I'}$.
		Then $\cstyle{A} \in \pi(d)$. 
		Since $\pi(d) \in \types(\Jmc')$, there exists $d' \in \domain{\Jmc'}$ such that $\typeinof{\Jmc'}{d'} = \pi(d)$.
		Since $\Jmc'$ is a model of $\tbox$, there exists $e' \in \cstyle{B}^{\Jmc'}$ such that $(d', e') \in \rstyle{R}^{\Jmc'}$.
		In particular, $\cstyle{B} \in \typeinof{\Jmc'}{e'}$ and $\typeinof{\Jmc'}{d'} \legitsucc_\rstyle{R} \typeinof{\Jmc'}{e'}$.
		It follows from $\pi$ being surjective that there exists $e \in \domain{\I'}$ with $\pi(e) = \typeinof{\Jmc'}{e'}$.
		Then $e \in \cstyle{B}^{\I'}$ and $(d, e) \in
                \rstyle{R}^{\I'}$ by definition of $\I'$, hence $d \in (\exists\rstyle{R}.\cstyle{B})^{\I'}$. 
		
		\item{$\axexistsleft$.}
		Let $d \in (\exists\rstyle{R}.\cstyle{B})^{\I'}$. 
		Then there exists $e \in \cstyle{B}^{\I'}$ such that $(d, e) \in \rstyle{R}^{\I'}$.
		By definition of $\rstyle{R}^{\I'}$, we have $\pi(d) \legitsucc_\rstyle{R} \pi(e)$.
		Since $\cstyle{B} \in \typeinof{\I'}{e} = \pi(e)$ and $\axexistsleft$, the definition of $\legitsucc_\rstyle{R}$ yields $\cstyle{A} \in \pi(d) = \typeinof{\I'}{d}$.
		Thus $d \in \cstyle{A}^{\I'}$.

		\item{$r \sqsubseteq s$.}
		Let $(d, e) \in \rstyle{r}^{\I'}$. Then $\pi(d) \legitsucc_\rstyle{r} \pi(e)$.
		Since $\tbox \models r \sqsubseteq s$, it is immediate that $\pi(d) \legitsucc_\rstyle{s} \pi(e)$.
		Therefore the definition of $\rstyle{s}^{\I'}$ yields $(d, e) \in \rstyle{s}^{\I'}$.
		
	\end{itemize}
	It remains to show that $\Imc' <_\CP \Imc$.
	We make use of the following claim.
	\begin{claim}
		$A^{\Imc'} \odot A^\Imc$ iff $A^{\Jmc'} \odot A^\Jmc$,
                for each concept name $A$ and $\odot \in \{\subseteq, \supseteq\}$.
	\end{claim}
	
		Let $A$ be a concept name.
		We prove the claim for $\odot =\; \subseteq$ only; for $\odot =\; \supseteq$, the arguments are similar.

                \smallskip
		``$\Rightarrow$''.
		Let $A^{\Imc'} \subseteq A^\Imc$ and $d \in
                A^{\Jmc'}$; we need to show that $d \in A^{\Jmc}$.
                First assume that $d \in \Delta_\mn{core}^\Imc$. Then
                $\mn{tp}_\Imc(d)=\mn{tp}_\Jmc(d)$ and
                $\mn{tp}_{\Imc'}(d) = \mn{tp}_{\Jmc'}(d)$. So
                $A^{\Imc'} \subseteq A^\Imc$ clearly implies
                $d \in A^\Jmc$, as required. Now assume that
                $d \notin \Delta_\mn{core}^\Imc$. Let
                $t=\mn{tp}_\Jmc(d)$. Then $\mn{tp}_{\Jmc'}(d) \in S_t$
                and consequently we find a $d' \in D_t$ with
                $\pi(d')=\mn{tp}_{\Jmc'}(d)$. This implies
                $\mn{tp}_{\Imc'}(d')=\mn{tp}_{\Jmc'}(d)$.  Since
                $d' \in D_t$, we have
                $\mn{tp}_\Imc(d)=t=\mn{tp}_\Jmc(d)$.
                So again,  $A^{\Imc'} \subseteq A^\Imc$ implies
                $d \in A^\Jmc$, as required.

                \smallskip
		``$\Leftarrow$''.
		Let $A^{\Jmc'} \subseteq A^\Jmc$ and $d \in
                A^{\Imc'}$; we need to show $d \in A^{\Imc}$.
                First assume that $d \in \Delta_\mn{core}^\Imc$. Then
                $\mn{tp}_\Imc(d)=\mn{tp}_\Jmc(d)$ and
                $\mn{tp}_{\Imc'}(d) = \mn{tp}_{\Jmc'}(d)$. So
                $A^{\Jmc'} \subseteq A^\Jmc$ clearly implies
                $d \in A^\Imc$, as required. Now assume that
                $d \notin \Delta_\mn{core}^\Imc$ and let
                $t'=\mn{tp}_{\Imc'}(d)$. By definition of $\Imc'$, we
                have $t'=\pi(d)$. By definition of $\pi$, there is a
                $t \in \mn{TP}_{\overline{\mn{core}}}(\Imc)$ such that
                $t'=\pi_t(d)$. Then $d \in D_t$ and $t' \in S_t$. The
                former yields $\mn{tp}_\Imc(d)=t$ and due to the
                latter, there is a $d'$ such that
                $\mn{tp}_\Jmc(d)=t=\mn{tp}_\Imc(d)$ and
                $\mn{tp}_{\Jmc'}(d)=t'=\mn{tp}_{\Imc'}(d)$.
                So again,  $A^{\Jmc'} \subseteq A^\Jmc$ implies
                $d \in A^\Imc$, as required.

                \medskip

        It is easy to see that since
	$\Imc' <_\CP \Imc$, the claim implies $\Jmc'<_\CP \Jmc$.
	We have derived a contradiction and conclude that $\Jmc$ is a
        model of $\Circ(\Kmc)$, as desired.
\end{proof}

\leminterlacingiscountermodel*
\begin{proof}
  Let $\I$ be a countermodel against $\circkb \models q(\bar a)$. It
  is clear that $\Imc' \not\models q[\bar a]$ since any homomorphism
  $g$ from $q$ to $\Imc'$ with $g(\bar x)=\bar a$ could be composed
  with the homomorphism $h$ from $\Imc'$ to \Imc to show that
  $\Imc \models q[\bar a]$. It is also straightforward to verify that
  \begin{itemize}
  \item[($*$)] 
    $\mn{tp}_{\Imc'}(d)=\mn{tp}_\Imc(h(d))$ for all $d \in \Delta^{\Imc'}$.
  \end{itemize}
  Using this and the
  definition of role extensions in $\Imc'$, it can be verified that
  $\Imc'$ is a model of \Kmc. % {\color{blue}do we need details?}
  Let us consider each possible shape of assertions and axioms in our normal form:
  \begin{itemize}
  	
  	\item
  	Assertions from $\abox$ are clearly satisfied as $\I$ is a model of $\abox $ and $\I'$ preserves $\I|_{\basedomainof{\I}}$ (recall $\indsof{\abox} \subseteq \basedomainof{\I}$).
  	
  	\item
  	Satisfaction of CIs with shape $\axtop$, $\axand$,
  	$\axnotright$ and $\axnotleft$ follows from remark ($*$) on types.
  	
  	\item{$\axexistsright$.}
  	Let $d \in \cstyle{A}^{\I'}$.
  	Thus $h(d) \in \cstyle{A}^\I$, and since $\I$ models $\kb$, $d' = f(h(d), r.B)$ is defined.
  	If $d' \in \coredomainof{\I}$, then definition of $\I'$ yields $(d, d') \in r^{\I'}$ and $d' \in B^{\I'}$.
  	Otherwise, $d r.B$ is a path through $\I$, and, by definition of $\I'$, we have in this case $(d, d r.B) \in r^{\I'}$ and $d r.B \in B^{\I'}$.
  	In both cases, $d \in (\exists r.B)^{\I'}$.
  	
  	\item{$\axexistsleft$.}
  	Let $d \in (\exists\rstyle{R}.\cstyle{B})^{\I'}$.
  	That is, there exists $e \in \cstyle{B}^{\I'}$ such that $(d, e) \in \rstyle{R}^{\I'}$.
  	Therefore $h(e) \in \cstyle{B}^{\I}$ and $(h(d), h(e)) \in \rstyle{R}^{\I}$, ie $h(d) \in (\exists\rstyle{R}.\cstyle{B})^{\I}$.
  	From $\I$ being a model of $\kb$, it follows $h(d) \in A^\I$, thus $d \in A^{\I'}$.

  	\item Axioms with shape $r \sqsubseteq s$ are clearly satisfied from the definition of $s^{\I'}$.
  	
  \end{itemize}

  It remains to prove that $\interlacing$ is minimal w.r.t.\ $<_\CP$.
  We use Lemma~\ref{lem-lemma5} with \Imc as the reference model, and it
  suffices to show that the preconditions of that lemma are
  satisfied. Clearly,
  $\coredomainof{\I} \subseteq \domain{\interlacing}$. Moreover, $(*)$
  and the fact that $h(d)=d$ for all $d \in \coredomainof{\I}$ implies
  that Condition~1 of Lemma~\ref{lem-lemma5} is satisfied.  We next
  verify that Condition~2 is also satisfied. First, let
  $d \in \Delta^\Jmc \setminus \coredomainof{\I}$. We have to show
  that $\mn{tp}_\Jmc(d) \in \noncoretypesof{\I}$. If
  $d \in \basedomainof{\I}$, then $h(d)=d$. From
  $d \notin \coredomainof{\I}$, we get
  $\mn{tp}_\Imc(d) \in \noncoretypesof{\I}$ and it remains to apply
  ($*$).  If $d \notin \basedomainof{\I}$, then
  $h(d) \notin \coredomainof{\I}$ and again we may use ($*$).
  Conversely, let $t \in \noncoretypesof{\I}$. We have to show that
  there is a $d \in \Delta^\Jmc \setminus \coredomainof{\I}$ with
  $\mn{tp}_\Jmc(d)=t$. But that $d$ is $e_t$ since $h(e_t)=e_t$ and by
  ($*$).
\end{proof}

\lemfinitemodelpropertywrtcore*
\begin{proof}
	Let $\Kmc=(\Tmc,\Amc)$ and let $\I$ be a model of $\circkb$.
	% We construct the desired model $\Jmc$ by starting from
        % $\I_{\mid \abox \cup \coredomainof{\I}}$ and adding exactly $m = \sizeof{\types(\tbox)}$ instances of each type from $\noncoretypesof{\I}$.
	Assume that $t_i \notin \Delta^\I$, for every $t \in
        \noncoretypesof{\I}$ and $1 \leq i \leq m$. Define $\Jmc$ by setting
	\[
	\begin{array}{r@{~}c@{~}l}
		\domain{\Jmc} & = & \indsof{\abox} \cup \coredomainof{\I} \cup \{ t_i \mid t \in \noncoretypesof{\I}, 1 \leq i \leq m \}
		\medskip \\
		\cstyle{A}^{\Jmc} & = & (\cstyle{A}^{\I} \cap \domain{\Jmc}) \cup \{ t_i \mid \cstyle{A} \in t, 1 \leq i \leq m \}
		\medskip \\
		\rstyle{r}^{\Jmc} & = & (\rstyle{r}^{\I} \cap (\domain{\Jmc} \times \domain{\Jmc}))  \hfill \text{(i)}
		\smallskip \\ & &
		\cup \, \{ (e, t_i) \mid 
		e \in \domain{\I}, \typeinof{\I}{e}
                                  \legitsucc_{\rstyle{r}} t, 1 \leq i
                                  \leq m \}  \hfill \text{(ii)}
		\smallskip \\ & &
		\cup \, \{ (t_i, e) \mid 
		e \in \domain{\I}, t \legitsucc_{\rstyle{r}}
                                  \typeinof{\I}{e}, 1 \leq i \leq m \}  \hfill \text{(iii)}
		\smallskip \\ & &
		\cup \, \{ (t_i, t'_j) \mid 
		t \legitsucc_{\rstyle{r}} t', 1 \leq i,j \leq m \} \hfill \text{(iv)}
	\end{array}
      \]
      for all concept names $A$ and role names $r$. It is easy to see
      that       $\typeinof{\Jmc}{e} = \typeinof{\I}{e}$
      for all $e \in \domain{\Imc} \cap \domain{\Jmc}$ and
      $\typeinof{\Jmc}{t_i} = t$ for all $t \in \types(\Tmc)$ and $1
      \leq i \leq m$.  This implies that
      $\I_{\mid \coredomainof{\I}} = \Jmc_{\mid \coredomainof{\Jmc}}$
      and $\noncoretypesof{\I} = \noncoretypesof{\Jmc}$ as desired.
      It also implies that Conditions 1 and 2 from Lemma~\ref{lem-lemma5} are satisfied.
      To show that \Jmc is a model of $\circkb$, it thus suffices to
      show
      that \Jmc is a model of $\kb$. It is clear by construction that
      \Jmc is a model of \Amc. For \Tmc, we consider all different
      forms of axioms:
	\begin{itemize}
		
		% \item{\bf$\conceptassertion{A}{a}$.}
		% Since $\I$ is a model of $\kb$, we have $\istyle{a} \in \cstyle{A}^{\I}$.
		% Furthermore, $\istyle{a} \in \domain{\Jmc}$ hence by definition of $\cstyle{A}^{\Jmc}$ we obtain $\istyle{a} \in \cstyle{A}^{\Jmc}$.
		
		% \item{\bf $\roleassertion{P}{a}{b}$.}
		% Since $\I$ is a model of $\kb$, we have $\istyle{a}, \istyle{b} \in \rstyle{P}^{\I}$.
		% Furthermore, $\istyle{a}, \istyle{b} \in \domain{\Jmc}$ hence by definition of $\rstyle{P}^{\Jmc}$ we obtain $(\istyle{a}, \istyle{b} \in \rstyle{P}^{\Jmc}$.
		
		\item
		Satisfaction of CIs of the form$\axtop$, $\axand$,
                $\axnotright$ and $\axnotleft$  immediately follows
                from $\types(\Jmc) \subseteq \types(\I)$ and $\I$
                being a model of \Tmc. We distinguish two cases:
		
		\item{$\axexistsright$.}
		Let $d \in \cstyle{A}^{\Jmc}$. 
		\begin{itemize}
		\item If $d \in \domain{\I}$, then we have $d \in \cstyle{A}^{\I}$.
		Since $\I$ is a model of $\Tmc$, there exists $e \in
                \cstyle{B}^{\I}$ such that $(d, e) \in \rstyle{R}^{\I}$.
		If $e \in \domain{\I}$, then $(d, e) \in
                \rstyle{R}^{\Jmc}$ due to Case~(i) in the definition
                of~$r^\Jmc$.
		Otherwise $t := \typeinof{\I}{e} \in \noncoretypesof{\I}$.
		In particular, $\cstyle{B} \in t$ and $\typeinof{\I}{d} \legitsucc_\rstyle{R} t$.
		Therefore $t_1 \in \cstyle{B}^\Jmc$ and $(d, t_1) \in
                \rstyle{R}^\Jmc$ due to Case~(ii), proving $d \in (\exists\rstyle{R}.\cstyle{B})^{\Jmc}$.
		\item If $d \notin \domain{\I}$, then $d = t_i$ for some $t \in \noncoretypesof{\I}$ and $1 \leq i \leq m$.
		By definition of $\noncoretypesof{\I}$, there exists $d' \in \domain{\I}$ s.t. $\typeinof{\I}{d'} = t = \typeinof{\Jmc}{d}$.
		From $d \in \cstyle{A}^{\Jmc}$, we get $A \in t$.
		Therefore $d' \in \cstyle{A}^{\I}$, and since $\I$ is
                a model of $\tbox$, there exists $e \in
                \cstyle{B}^{\I}$ such that $(d', e) \in \rstyle{R}^{\I}$.
		In particular, $\cstyle{B} \in \typeinof{\I}{e}$ %,
                % hence $e \in \cstyle{B}^\Jmc$,
                and $t \legitsucc_\rstyle{R} \typeinof{\I}{e}$.
		If $e \in \domain{\Jmc}$, then $e \in B^\Jmc$ and
                Case~(iii) in the definition of $\rstyle{R}^{\Jmc}$
                ensures $(d, e) \in \rstyle{R}^\Jmc$, which gives $d
                \in (\exists\rstyle{R}.\cstyle{B})^{\Jmc}$.
                If $e \notin \domain{\Jmc}$, then $t'=\typeinof{\I}{e} \in
                \noncoretypesof{\I}$. Let $e'= t'_j$ for some $j$ with
                $1 \leq j \leq m$.
		Case~(iv) in the definition of $\rstyle{R}^{\Jmc}$ yields $(d, e') \in \rstyle{R}^\Jmc$, which again gives $d \in (\exists\rstyle{R}.\cstyle{B})^{\Jmc}$.
		\end{itemize}
		
		\item{$\axexistsleft$.}
		Let $d \in (\exists\rstyle{R}.\cstyle{B})^{\Jmc}$.
		Then there exists $e \in \cstyle{B}^{\Jmc}$ such that $(d, e) \in \rstyle{R}^{\Jmc}$.
		From each case in definition of $\rstyle{R}^{\Jmc}$, we easily get $\typeinof{\Jmc}{d} \legitsucc_\rstyle{R} \typeinof{\Jmc}{e}$.
		Since $e \in \cstyle{B}^{\Jmc}$ we have in particular $\cstyle{B} \in \typeinof{\Jmc}{e}$.
		Combined with $\tbox \models \axexistsleft$ and the definition of $\typeinof{\Jmc}{d} \legitsucc_\rstyle{R} \typeinof{\Jmc}{e}$, we obtain $\cstyle{A} \in \typeinof{\Jmc}{d}$, that is $d \in \cstyle{A}^{\Jmc}$.

		\item{$r \sqsubseteq s$.}
		Let $(d, e) \in \rstyle{r}^{\Jmc}$.
		If this is due to Case~(i) in the definition of
                $\rstyle{r}^{\Jmc}$, then
                $(d, e) \in \rstyle{s}^{\Jmc}$ since $\I$ is a model of~$\Tmc$.
		For all other three cases, it suffices to note that,
                due to $r \sqsubseteq s \in \tbox$, $t_1
                \legitsucc_\rstyle{r} t_2$ implies $t_1
                \legitsucc_\rstyle{s} t_2$ for all types $t_1, t_2$.
		
	\end{itemize}
	Finally, we remark that the size of $\domain{\Jmc}$ is bounded by $\sizeof{\indsof{\abox}} + \sizeof{\coredomainof{\I}} + m \cdot \sizeof{\noncoretypesof{\I}}$.
	From $\sizeof{\coredomainof{\I}} \leq m \cdot
        \sizeof{\coretypesof{\I}}$ and $\sizeof{\coretypesof{\I}} +
        \sizeof{\noncoretypesof{\I}} = \sizeof{\types(\I)} \leq m$ we obtain
	$\sizeof{\domain{\Jmc}} \leq \sizeof{\abox} + m^2$. 
	Recalling $m = \sizeof{\types(\tbox)} \leq 2^\sizeof{\tbox}$,
        we obtain $|\Delta^\Jmc| \leq\sizeof{\abox} +
        2^{2\sizeof{\tbox}}$ as required.
\end{proof}

\section{Proofs for Section~\ref{subsection-alchi-combined}}

\lemmamosaic*

\input{soundness}%
\input{completeness}

\thmcombinedlowerel*

\input{thm-combined-lower-el}

\section{Proofs for Section~\ref{subsection-alchi-data}}

In the main part of the paper, we have defined neighborhoods only for
the unraveling $\Imc'$ of the interpretation \Imc. In the proofs, we
also consider neighborhods in the quotient
$\J = \interleavingof{\I}/{\sim_{\maxradius}}$. We thus start with
a more general definition of neighborhoods.

Let \Imc be an interpretation and $\Delta \subseteq \Delta^{\Imc}$.
For $n \geq 0$ and $d \in \Delta^\Imc \setminus \Delta$, we use
$\Nmc_n^{{\Imc},\Delta}(d)$ to denote the \emph{$n$-neighborhood of
  $d$ in {\Imc} up to} $\Delta$, that is, the set of all elements
$e \in \Delta^{\Imc} \setminus \Delta$ such that the undirected
graph $G_{\Imc}$ associated with \Imc contains a path
$d_0,\dots,d_k$ with $0 \leq k \leq n$, $d_0=d$,
$d_0,\dots,d_{k-1} \notin \Delta$, and $d_k=e$.

So the neighborhoods $\Nmc_n(d)$ defined in the main body of
the paper are now called $\Nmc_n^{{\Imc'}, \basedomainof{\I}}(d)$.

\lemquotient*

\input{quotient}

\thmdataupperalchi*
\begin{proof}
  Assume that we are given a circumscribed $\ALCHI$ KB $\Circ(\Kmc)$ with
  $\Kmc=(\Tmc,\Amc)$ and a UCQ $q$.  We describe a $\Sigma^p_2$ procedure to decide whether $\Circ(\Kmc) \not\models
  q(\bar a)$.
  
  We first guess an interpretation \Imc with $|\Delta^\Imc| \leq |\Amc|+(2^{|\Tmc|+2}+1)^{3|q|}$.
  We next check in polynomial time that \Imc is a model of \Kmc
  and that \Imc is minimal w.r.t.\ $<_{\mn{CP}}$ by co-guessing a
  model \Jmc of \Kmc with $\Jmc <_{\mn{CP}} \Imc$. If one of the
  checks fails, we reject. Otherwise, for each CQ $p$ in $q$, we verify whether there is a homomorphism from $p$ to \Imc. This is done brute-force, in time $O(|\Delta^{\Imc}|^{|q|})$.
  We accept if there is no such homomorphism and reject otherwise.
  This procedure is correct due to Lemma~\ref{lem-quotient}.
\end{proof}

\thmdatalowerel*
\input{thm-data-lower-el}

\section{Proofs for Section~\ref{subsection-dllite-combined}}

\thmcombinedlowerdlliter*
\begin{proof}
  % , which is why we skip most
  % explanations.
	%
  We reduce from (Boolean) UCQ evaluation on \dlliter KBs with
  closed concept names, which is defined in the expected way
   and known to be \TwoExpTime-hard
   \cite{Ngo2016}.
   Let $\Kmc_\Sigma$ be a \dlliter KB with closed concept names,
   $\Kmc = (\Tmc,\Amc)$, and let $q$ be a Boolean UCQ.  We construct a
   circumscribed \dlliter KB $\mn{Circ}_\CP(\Kmc')$, with
   $\Kmc'=(\Tmc',\Amc')$, and a CQ $q'$ such that
   $\Kmc_\Sigma \models q$ iff $\mn{Circ}_\CP(\Kmc') \models q'$.

   As
   in the proof of \cref{thm:combined-lower-el}, we minimize only a
   single concept name $M$ and include \Amc in $\Amc'$. To construct
   $\Tmc'$, we start from \Tmc and extend with additional concept
   inclusions. For $q'$, we start from $q$ and extend with
   additional disjuncts. We will actually use individuals
   $a \in \mn{Ind}(\Amc)$ as constants in~$q'$. These can be
   eliminated by introducing a fresh concept name $A_a$, extending
   \Amc with $A_a(a)$, and replacing in each CQ in $q'$ the constant
   $a$ with a fresh variable $x_a$ and adding the atom $A_a(x_a)$.

   As in the proof of \cref{thm:combined-lower-el}, we include in
   $\Tmc'$ the CI
   \begin{align}
		A \sqsubseteq \M & \quad \text{for all } A \in \Sigma
   \end{align}
   and then have to rule out non-asserted instances of closed concept
   names. To rule out non-asserted instances inside of $\Ind(\Amc)$,
   we add to $q'$ the disjunct $A(a)$ for all $A \in \Sigma$ and
   $a \in \Ind(\Amc)$ with $A(a) \notin \Amc$.

   To rule out instances of closed concept names outside of
   $\Ind(\Amc)$, add
	\begin{align}
		\M(\tc)
	\end{align}
	% s#
	where $\tc$ is a fresh individual. As in the proof of
        \cref{thm:combined-lower-el}, this guarantees that models with
        instances of closed concept names outside of $\Ind(\Amc)$ are
        not minimal. To ensure that no closed concept names are made
        true at \tc, we extend $q'$ with the disjunct $r(x,t)$ for every
        role name $r$ used in \Tmc.
                \\[2mm]
        {\bf Claim.} 
                $\Kmc_\Sigma \models q$ iff $\Circ(\Kmc') \models q'$.
\\[2mm]
        The proof is rather straightforward; we omit the details.
%                 \smallskip
%
% 	\noindent The proof is very similar to that of \cref{lem:K_Sigma_q_Circ_CP_K_q}, but some arguments differ.
% 	%
% 	Generally, replace every occurrence of $\Aqt$ with $\{\tc\}$.
% 	%
% 	In the ``$\Leftarrow$''-direction, to derive $\Jmc \not \models q'$, we need, due to $q' = q \cup \exists x.L$, the additional argument that $\mn{L}^\Jmc = \emptyset$ by construction, but can drop the arguments about $h(x) \in \X^\Jmc$ for each $x \in V$.
%
% 	For the ``$\Rightarrow$''-direction, replace the argument that the extension of $\mn{L}$ not being empty causes the identity function to be a homomorphism from $\Dmc_{q'}$ to {\Imc'} via \cref{eq:bar_X,eq:X_Bar_X,eq:copy_query_links,eq:propagate_L_copy} with any instance of $\mn{L}$ being an answer to $q'$.
% 	%
% 	That $\Jmc = \Imc |_{\X^\Imc}$ is a model of $\Tmc$ does not follow from the replaced \cref{eq:T_Axioms_X}, but by the facts that $\Tmc \subseteq \Tmc'$ and that, ensured by \cref{eq:r_X_X}, \tc is not used as a successor for any existential restriction.
% 	%
% 	That $\Jmc \not \models q$ follows directly from the construction of $q'$ and $\Imc \not \models q$.
% 	%
% 	Proving that \Jmc respects $\Sigma$ is much simpler:
% 	%
% 	In the case of $\hat x \notin \Ind(\Amc)$, we do not need to account for the copy of $\Dmc_q$ (i.e., to interpret it ``maximally'').
% 	%
% 	\cref{claim:V_type} can be ignored as well.
% 	%
% 	Finally, not needing to consider $C_\X$ turns the inductions for \cref{claim:t_type} into simple observations.
\end{proof}

We now work towards a proof of
Theorem~\ref{thm-combined-upper-dllitebool}, first establishing the
following.
\lemmaboolcountermodel*

\newcommand{\pathsbool}{\Pmc_{\mathsf{bool}}}
\newcommand{\boolunrav}{\I'_\mathsf{bool}}
Refining the unraveling begins by noticing the set $\Omega$ now only contains elements with shape $r\top$ as $\dllitebool$ TBoxes are considered.
We drop the $\top$ concept for simplicity.
Recall that we assume chosen a representative $e_t \in \domain{\I}$ for each non-core type $t \in \noncoretypesof{\I}$.
We define the set $\pathsbool$ of {$\mathsf{bool}$-paths through \Imc} along with
a mapping $h$ that assigns to each $p \in \pathsbool$ an element of~$\Delta^\Imc$:
\begin{itemize}
	
	\item each element $d$ of the set
	$$\basedomainof{\I} := \indsof{\abox} \cup \coredomainof{\I} \cup \{
	e_t \mid t \in \noncoretypesof{\I} \}.$$
	is a path in $\pathsbool$ and
	$h(d)=d$;
	
	\item if $p \in \pathsbool$ with $h(p)=d$ and $r \in \Omega$ such that:
	\begin{enumerate}
		\item[(a)] $f(d,r)$ is defined and not from $\Delta^\Imc_{\mn{core}}$ and
		\item[(b)] $p$ does not end by $r^-$, which we denote $\mn{tail}(p) \neq r^-$.
	\end{enumerate} 
	then
	$p'=p r$ is a path in $\pathsbool$ and $h(p')=f(d,r)$.
	
\end{itemize}

For every role $r$, define
$$
\begin{array}{@{}r@{\;}c@{\;}l}
	R_r &=& \{ (a,b) \mid a,b \in \Ind(\Amc), \Kmc \models r(a,b)
	\} \, \cup \\[1mm]
	&& \{ (d,e) \mid d,e \in  \coredomainof{\I}, (d,e) \in r^\Imc \} \,
	\cup \\[1mm]
	&& \{ (p,p') \mid p'=pr %, \Tmc
	% \models s \sqsubseteq r
	\} \, \cup\\[1mm]
	%          && \{ (p',p) \mid p'=pr^-A \in \Pmc %,
	%          % \Tmc \models s \sqsubseteq r
	%             \} \,
	% \cup \\[1mm]
	&& \{ (p,e) \mid %p=p'rA \in \Pmc,
	e=f(h(p),r) \in \Delta^\Imc_{\mn{core}}, \mn{tail}(p) \neq r^- %, \Tmc
	% \models s \sqsubseteq r
	\}. %  \,
	%  \cup \\[1mm]
	% && \{ (e,p) \mid p=p'r^-A \in \Pmc,
	%                 e=f(h(p),rA) \in \Delta^\Imc_{\mn{core}} %, \Tmc
	%                 % \models s \sqsubseteq r
	%    \}
\end{array}
$$
Now the $\mathsf{bool}$-{unraveling} of \Imc is defined by setting
$$
\begin{array}{r@{\;}c@{\;}l}
	\Delta^{\Imc'} &=& \pathsbool \\[1mm]
	A^{\Imc'} &=& \{ p \in \pathsbool \mid h(p) \in A^\Imc \} \\[1mm]
	r^{\Imc'} &=& \displaystyle R_r \cup \{ (e,d) \mid (d,e) \in R_{r^-} \}
\end{array}
$$
for all concept names $A$ and role names $r$. It is easy to verify
that $h$ is a homomorphism from $\Imc'$ to \Imc.
%The $\mathsf{bool}$-unraveling $\boolunrav$ is then define as in Section~\ref{subsection-alchi-interlacing} replacing $\Pmc$ by $\pathsbool$ (and $h$ by its corresponding version).
It is a technicality to verify that $\boolunrav$ satisfies the same properties as the previous unraveling $\interlacingof{\I}$, that is: if $\I$ is a countermodel for $\query$ over $\circkb$, then so is $\boolunrav$. The key additional property satisfied by $\boolunrav$ is the following:

\begin{lemma}
	\label{lemma-unique-succ}
	For any $\rolestyle{r} \in \rnames$ and $d_1 \in \domain{\boolunrav} \setminus \basedomainof{\I}$, there is at most one element $d_2 \in \domain{\boolunrav}$ such that $(d_1, d_2) \in \rolestyle{R}^{\boolunrav}$.
\end{lemma}
\begin{proof}
	Unfolding the definition of $\rolestyle{R}^{\boolunrav}$ and recalling $d_1 \notin \basedomainof{\I}$, we obtain that if $d_1 \in \domain{\boolunrav} \setminus \basedomainof{\I}$ and $(d_1, d_2) \in \rolestyle{R}^{\boolunrav}$, then either:
	\begin{itemize}
		\item $(d_1, d_2) \in R_r$ and either $d_2 = d_1 r$ (Case~1) or $d_2 = f(h(d_1), r) \in \basedomainof{\I}$ and $\mn{tail}(d_1) \neq r^-$ (Case~2).
		
		\item $(d_2, d_1) \in R_{r^-}$ and we have $d_1 = d_2 r^-$ (Case~3).
	\end{itemize}
	To verify uniqueness, let us assume there exist $d_2$ and $d_2'$ s.t.\ $(d_1, d_2'), (d_1, d_2') \in \rolestyle{R}^{\boolunrav}$.
	We want to prove $d_2 = d_2'$.
	From the small analysis above, there are $3 \times 3$ cases to consider:
	\begin{enumerate}
		\item if $d_2 = d_1 r$, then:
		\begin{enumerate}
			\item[1.] if $d_2' = d_1 r$, we obtain directly $d_2' = d_2$.
			\item[2.] if $d_2' = f(h(d_1), r) \in \basedomainof{\I}$ and $\mn{tail}(d_1) \neq r^-$, then it contradicts $d_1 r \in \pathsbool$ (Condition~(a)).
			\item[3.] if $d_1 = d_2' r^-$, then $d_2 = d_2' r^- r$, which contradicts $d_2 \in \pathsbool$ (Condition~(b)).
		\end{enumerate}
		\item if $d_2 = f(h(d_1), r) \in \basedomainof{\I}$ and $\mn{tail}(d_1) \neq r^-$, then:
		\begin{enumerate}
			\item[1.] if $d_2' = d_1 r$, then same argument as 1.2. 
			\item[2.] if $d_2' = f(h(d_1), r) \in \basedomainof{\I}$ and $\mn{tail}(d_1) \neq r^-$, then $d_2' = d_2$ from $h$ and $f$ being functions.
			\item[3.] if $d_1 = d_2' r^-$, then it contradicts $\mn{tail}(d_1) \neq r^-$.
		\end{enumerate}
			\item if $d_1 = d_2 r^-$, then:
		\begin{enumerate}
			\item[1.] if $d_2' = d_1 r$, then same argument as 1.3. 
			\item[2.] if $d_2' = f(h(d_1), r) \in \basedomainof{\I}$ and $\mn{tail}(d_1) \neq r^-$, then same argument as 2.3.
			\item[3.] if $d_1 = d_2' r^-$, we obtain directly $d_2' = d_2$.
		\end{enumerate}
	\end{enumerate}
\end{proof}

Repeated applications of Lemma~\ref{lemma-unique-succ} ensure that each partial homomorphism of a CQ $p \in q$ in the non-$\basedomainof{\I}$ part of the bool-unraveling can be completed uniquely in a maximal such partial homomorphism (see further Lemma~\ref{lemma-poly-neighborhoods}).
This motivates a refined notion of the neighborhood of an element $d$, restricting the (usual) neighborhood to those elements $e$ that can be reached by a homomorphism of some connected subquery involving both $d$ and $e$.
Formally, for $n \geq 0$ and
$\Delta \subseteq \Delta^\Imc$, we use $\coreneighof{n}{d}{\I}{\domain{}}$
to denote the \emph{$n$-bool-neighborhood of $d$ in \Imc up to}
$\Delta$, that is, the set of all elements $e \in \neighof{n}{d}{\I}{\domain{}}$
such that there exists a connected subquery $p' \subseteq p$ for some $p \in q$ and a homomorphism $\pi : p' \rightarrow \neighof{n}{d}{\I}{\domain{}}$ s.t.\ $d, e \in \pi(\variablesof{p'})$.

%\begin{definition}
%	\label{def-bool-neighborhoods}
%	Consider an interpretation $\I$ and an element $c \in \domain{\I}$. 
%	Its $n$-$\mathsf{bool}$-neighbourhood $\coreneighof{n}{c}{\I}{\domain{}}$ w.r.t. a subdomain $\domain{} \subseteq \domain{\I}$ is defined as:
%	\[
%	\begin{array}{rcl}
%		\coreneighof{0}{c}{\I}{\domain{}} & := & \{ c \}
%		\\ 
%		\coreneighof{n+1}{c}{\I}{\domain{}} & := &
%		\left\{ e ~ \middle|
%		\begin{array}{l}
%			\exists p \subseteq q_k \in q \text{ connected}
%			\\
%			\, \exists \match : p \rightarrow \I_{\mid (\coreneighof{n}{c}{\I}{\domain{}} \,\setminus\, \domain{}) \,\cup\, \{ e \}} \text{ match}
%			\\
%			c, e \in \match(\termsof{p})
%		\end{array}
%		\hspace{-.3em}
%		\right\}
%	\end{array}
%	\]
%\end{definition}

%\begin{remark}
%	By contrast with ``usual'' neighborhoods, bool-neighborhoods are query dependent.
%%	Furthermore, since the subquery $p$ must be connected, the inclusion $\coreneighof{n}{c}{\I}{\domain{}} \subseteq \neighof{n}{c}{\I}{\domain{}}$ is straightforward.
%\end{remark}

The following polynomial bound on their size in the bool-unraveling is the central property allowing bool-neighborhoods to improve our construction.

%Indeed, Lemma~\ref{canmodunique} applied on core-neighbourhoods proves that the core-neighbourhood of an element $c \in \domain{\interlacingof{\I}} \setminus \deltastar$ has size at most polynomial.

\begin{lemma}
	\label{lemma-poly-neighborhoods}
	Let $\I$ be a model of $\kb$ and $\boolunrav$ its bool-unraveling.
	Consider $d \in \domain{\boolunrav} \setminus \basedomainof{\I}$, then $\sizeof{\coreneighof{n}{d}{\boolunrav}{\basedomainof{\I}}} \leq \sizeof{q}^2 ( \sizeof{\tbox} + 1)$.
\end{lemma}
\begin{proof}
	\newcommand{\termsof}[1]{\variablesof{#1}}
	Let $c \in \domain{\boolunrav} \setminus \domain{\basecandidate}$
	in a first step, we prove the number of elements in $\coreneighof{n}{c}{\boolunrav}{\domain{\basecandidate}} \setminus \domain{\basecandidate}$ is at most $\sizeof{q}^2$.
	In a second step, we notice each element $e \in \coreneighof{n}{c}{\boolunrav}{\domain{\basecandidate}} \cap \domain{\basecandidate}$ must be connected to an element $d \in \coreneighof{n}{c}{\boolunrav}{\domain{\basecandidate}} \setminus \domain{\basecandidate}$ by construction of (usual) neighborhoods.
	However, from Lemma~\ref{lemma-unique-succ}, each such element $d$ is connected to at most $\sizeof{\tbox}$ elements.
	From the first step it follows there are at most $\sizeof{q}^2 \cdot \sizeof{\tbox}$ elements in $e \in \coreneighof{n}{c}{\boolunrav}{\domain{\basecandidate}} \cap \domain{\basecandidate}$, hence the claimed bound.
	
	It remains to prove the first step.
	We start by proving that if the connected subquery $p' \subseteq p$ for some $p \in q$ and the variable $v_0$ that shall map on $c$ are fixed, then all homomorphisms $p' \rightarrow { (\coreneighof{n}{c}{\boolunrav}{\basedomainof{\I}} \,\setminus\, \basedomainof{\I})}$ mapping $v_0$ on $c$ are equal.
	Consider two such homomorphisms $\match_1$ and $\match_2$.
	We proceed by induction on the variables $v$ of $p'$ being connected.
	For $v = v_0$, we have $\match_1(v_0) = \match_2(v_0)$ by definition.
	For a further term $v$, we use the induction hypothesis, that is, the existence of an atom $\rolestyle{R}(v', v) \in p'$ (or the other way around) such that $\match_1(v') = \match_2(v')$.
	Recall $\match_1$ and $\match_2$ are homomorphisms of $p'$ in $\coreneighof{n}{c}{\boolunrav}{\basedomainof{\I}} \,\setminus\, \basedomainof{\I}$, in particular $\match_1(v'), \match_2(v') \notin \basedomainof{\I}$, hence we can apply Lemma~\ref{lemma-unique-succ}, yielding $\match_1(v) = \match_2(v)$.
	
	This proves that, for a fixed $v_0 \in \termsof{p}$, each connected subquery $p' \subseteq p$ admitting a homomorphism in $\coreneighof{n}{c}{\boolunrav}{\basedomainof{\I}} \,\setminus\, \basedomainof{\I}$ defines at most $\sizeof{p}$ new neighbors, but also that if $p' \subseteq p'' \subseteq p$ are two such subqueries, then the neighbors defined by $p'$ are subsumed by those defined by $p''$ (the restriction to the variables of $p'$ of {the} unique homomorphism of $p''$ mapping $v_0$ on $c$ must coincide with {the} unique homomorphism of $p'$ mapping $v_0$ on $c$).
	Still, for a fixed $v_0$, consider now two connected subqueries $p_1, p_2 \subseteq p$, each admitting a (unique) homomorphism $\match_1$ resp. $\match_2$, to $\coreneighof{n}{c}{\boolunrav}{\basedomainof{\I}} \,\setminus\, \basedomainof{\I}$ mapping $v_0$ to $c$, and each maximal, w.r.t. the inclusion, for this property.
	By the previous property, we know $\match_1$ and $\match_2$ coincide on $\termsof{p_1} \cap \termsof{p_2}$.
	Therefore, $p_1 \cup p_2$ admits a homomorphism to $\coreneighof{n}{c}{\boolunrav}{\basedomainof{\I}} \,\setminus\, \basedomainof{\I}$ mapping $v_0$ to $c$, being $\match_1 \cup \match_2$.
	However, since $p_1$ and $p_2$ are assumed maximal for this property, we must have $p_1 = p_2$.
	
	Therefore, for a fixed $v_0 \in \termsof{p}$, there is a unique maximal connected subquery $p_{\textsf{max}} \subseteq p$ admitting a homomorphism in $\coreneighof{n}{c}{\boolunrav}{\basedomainof{\I}} \,\setminus\, \basedomainof{\I}$ and mapping $v_0$ to $c$.
	As previously seen, the neighbors defined by $p_\textsf{max}$ subsume those defined by other subqueries of $p$, and since the homomorphism for $p_{\textsf{max}}$ is unique, it defines at most $\sizeof{p}$ neighbors.
	This holds for each possible choices of term $v_0$, hence a total number of possible neighbors issued by $p$ bounded by $\sizeof{p}^2$.
	Iterating over each $p \in q$, we hence obtain the claimed bound of at most $\sizeof{q}^2$ elements in $\coreneighof{n}{c}{\boolunrav}{\basedomainof{\I}} \,\setminus\, \basedomainof{\I}$.
\end{proof}

Using bool-neighborhoods in the quotient construction presented in
Section~\ref{subsection-alchi-data}, the number of equivalence classes
drops, which yieldings Lemma~\ref{lemma-bool-countermodel}.

\begin{restatable}{lemma}{lemmaportionaremodels}
	\label{lemma-portion-are-models}
	For all $\Pmc \subseteq \domain{\I}$, $\I_\Pmc$ is a model of $\kb$.
\end{restatable}
%\lemmaportionaremodels*
%
\begin{proof}
	Let $\Pmc\subseteq \domain{\I}$, we have:
	\begin{itemize}
		\item $\I_\Pmc$ models $\abox$ as it inherits interpretations of concepts and roles on $\indsof{\abox}$ from $\I$, which is a model of $\abox$.
		\item Axioms in $\tbox$ with shape $\axtop$, $\axand$, $\axnotright$ or $\axnotleft$ are satisfied since $\I_\Pmc$ inherits interpretations of concept names from $\I$, which is a model of $\tbox$.
		\item Axioms in $\tbox$ with shape $A \incl \exists r$ are witnessed with an $r$-edge pointing to $w_r$.
		\item Axioms in $\tbox$ with shape $\exists r \incl A$ are satisfied since every element in $\I_\Pmc$ having some $r$-edge already has one in $\I$ (and interpretations of concept names are preserved).
		\item Role inclusions $r \incl s$ are satisfied on $\indsof{\abox} \times \indsof{\abox}$ from $\I$ being a model of $\tbox$ in the first place, otherwise directly from the definition of $s^{\Imc_\Pmc}$.
	\end{itemize}
	This proves $\I_\Pmc \models \kb$ as desired.
\end{proof}

\lemmacriteriacombined*
To piece together the $\J_{e}$ and reconstruct an eventual $\J$, we first prove the following property:

\begin{lemma}
	\label{lemma-portions-union}
	%Let $\I$ be a model of a $\dllitebool^{\Hmc^-}$ KB $\kb$ and $\CP$ a circumscription pattern.
	Let $\Pmc_1, \Pmc_2 \subseteq \domain{\I}$ and $\J_1$, $\J_2$ two models of $\kb$ s.t.\ $\J_1 <_\CP \I_{\Pmc_1}$ and $\J_2 <_\CP \I_{\Pmc_2}$.
	If $\J_1 |_{\domain{\J_2}} = \J_2 |_{\domain{\J_1}}$, then $\J_1 \cup \J_2 <_\CP \I_{\Pmc_1 \cup \Pmc_2}$.
\end{lemma}

\begin{proof}
	Assume $\J_1 |_{\domain{\J_2}} = \J_2 |_{\domain{\J_1}}$.
	It is easily verified that $\J_1 \cup \J_2$ is also a model of $\kb$ since $\J_1$ and $\J_2$ agree on their shared domain.
	We now check that all four conditions from the definition of $<_\CP$ are satisfied:
	\begin{enumerate}
		\item 
		From $\J_1 <_\CP \I_{\Pmc_1}$ we have $\domain{\J_1} = \domain{\I_{\Pmc_1}}$ and similarly for $\J_2$ we have $\domain{\J_2} = \domain{\I_{\Pmc_2}}$.
		It follows from its definition that $\domain{\I_{\Pmc_1 \cup \Pmc_2}} = \domain{\I_{\Pmc_1}} \cup \domain{\I_{\Pmc_2}}$.
		Therefore we have as desired $\domain{\J_1 \cup \J_2} = \domain{\I_{\Pmc_1 \cup \Pmc_2}}$.
		\item 
		Let $A \in \Fsf$.
		From $\J_1 <_\CP \I_{\Pmc_1}$ we have $A^{\J_1} = A^{\I_{\Pmc_1}}$ and similarly for $\J_2$ we have $A^{\J_2} = A^{\I_{\Pmc_2}}$.
		It follows from its definition that $A^{\I_{\Pmc_1 \cup \Pmc_2}} = A^{\I_{\Pmc_1}} \cup A^{\I_{\Pmc_2}}$.
		Therefore we have as desired $A^{\J_1 \cup \J_2} = A^{\I_{\Pmc_1 \cup \Pmc_2}}$.
		\item 
		Let $A \in \Msf$ such that $A^{\J_1 \cup \J_2} \not\subseteq A^{\I_{\Pmc_1 \cup \Pmc_2}}$.
		We may assume w.l.o.g.\ that $A$ is minimal w.r.t.\ $\prec$ for this property.
		We thus have $e \in A^{\J_1 \cup \J_2} \setminus A^{\I_{\Pmc_1 \cup \Pmc_2}}$.
		We either have $e \in \domain{\J_1}$ or $e \in \domain{\J_2}$.
		We treat the case $e \in \domain{\J_1}$, the arguments for $e \in \domain{\J_2}$ are similar.
		From $\J_1 <_\CP \I_{\Pmc_1}$, there exists a concept $B_1 \prec A$ s.t.\ $B_1^{\J_1} \subsetneq B_1^{\I_{\Pmc_1}}$.
		We chose such a $B_1$ that is minimal for this property, that is s.t.\ for all $B \prec B_1$, we have $B^{\J_1} = B^{\I_{\Pmc_1}}$ (recall $A$ is minimal for its property so that such a $B$ must verify $B^{\J_1 \cup \J_2} \subseteq B^{\I_{\Pmc_1 \cup \Pmc_2}}$ hence $B^{\J_1} \subseteq B^{\I_{\Pmc_1}}$).
		If $B_1^{\J_2} \subseteq B_1^{\I_{\Pmc_2}}$, then we are done as we obtain $B_1^{\J_1 \cup \J_2} \subsetneq B_1^{\I_{\Pmc_1 \cup \Pmc_2}}$.
		Otherwise, we have $B_1^{\J_2} \not\subseteq B_1^{\I_{\Pmc_2}}$ and from $\J_2 <_\CP \I_{\Pmc_2}$, there exists a concept $B_2 \prec B_1$ s.t.\ $B_2^{\J_2} \subsetneq B_2^{\I_{\Pmc_2}}$.
		Since $B_1$ has been chosen minimal, we have in particular $B_2^{\J_1} = B_2^{\I_{\Pmc_1}}$, which yields $B_2^{\J_1 \cup \J_2} \subsetneq B_2^{\I_{\Pmc_1 \cup \Pmc_2}}$.
		\item
		From $\J_1 <_\CP \I_{\Pmc_1}$, there exists a concept $A_1 \in \Msf$ s.t.\ $A_1^{\J_1} \subsetneq A_1^{\I_{\Pmc_1}}$ and for all $B \prec A_1$, we have $B^{\J_1} = B^{\I_{\Pmc_1}}$.
		If $A_1^{\J_2} \subsetneq A_2^{\Pmc_2}$ and for all $B \prec A_1$, $B^{\J_2} = B^{\Pmc_2}$, then we obtain directly $A_1^{\J_1 \cup \J_2} \subsetneq A_1^{\I_{\Pmc_1 \cup \Pmc_2}}$ and for all $B \prec A_1$, $B^{\J_1 \cup \J_2} = B^{\I_{\Pmc_1 \cup \Pmc_2}}$ and we are done.
		Otherwise:
		\begin{itemize}
			\item If $A_1^{\J_2} \not\subseteq A_1^{\I_{\Pmc_2}}$, then from $\J_2 <_\CP \I_{\Pmc_2}$, there exists a concept $A_2 \prec A_1$ s.t.\ $A_2^{\J_2} \subsetneq A_2^{\I_{\Pmc_2}}$.
			Consider a minimal such $A_2$, that is s.t.\ for all $A \prec A_2$, we have $A^{\J_2} = A^{\I_{\Pmc_2}}$ or $A^{\J_2} \not\subseteq A^{\I_{\Pmc_2}}$. 
			Notice the second option cannot happen otherwise from $\J_2 <_\CP \I_{\Pmc_2}$ we could obtain $A_3 \prec A_2$ s.t.\ $A_2^{\J_2} \subsetneq A_2^{\I_{\Pmc_2}}$, contradicting the minimality of $A_2$.
			Therefore $A_2$ being minimal yields that for all $A \prec A_2$, we have $A^{\J_2} = A^{\I_{\Pmc_2}}$.
			Now, from the minimality of $A_1$, we extend this to $\J_1 \cup \J_2$ and obtain $A_2^{\J_1 \cup \J_2} \subsetneq A_2^{\I_{\Pmc_1 \cup \Pmc_2}}$ and for all $B \prec A_2$, $B^{\J_1 \cup \J_2} = B^{\I_{\Pmc_1 \cup \Pmc_2}}$.
			\item If there exists $A_2 \prec A_1$ s.t.\ $A_2^{\J_2} \neq A_2^{\I_{\Pmc_2}}$.
			Consider a minimal such $A_2$, that is s.t.\ for all $A \prec A_2$, we have $A^{\J_2} = A^{\I_{\Pmc_2}}$.
			Notice we must have $A_2^{\J_2} \subseteq A_2^{\I_{\Pmc_2}}$, otherwise from $\J_2 <_\CP \I_{\Pmc_2}$ we could obtain $A_3 \prec A_2$ s.t.\ $A_2^{\J_2} \subsetneq A_2^{\I_{\Pmc_2}}$, contradicting that for all $A \prec A_2$, we have $A^{\J_2} = A^{\I_{\Pmc_2}}$.
			Therefore, since $A_2^{\J_2} \neq A_2^{\I_{\Pmc_2}}$, it must be that $A_2^{\J_2} \subsetneq A_2^{\I_{\Pmc_2}}$.
			Now, from the minimality of $A_1$, we extend this to $\J_1 \cup \J_2$ and obtain $A_2^{\J_1 \cup \J_2} \subsetneq A_2^{\I_{\Pmc_1 \cup \Pmc_2}}$ and for all $B \prec A_2$, $B^{\J_1 \cup \J_2} = B^{\I_{\Pmc_1 \cup \Pmc_2}}$.
			%\item Otherwise we have $A_1^{\J_1 \cup \J_2} \subsetneq A_1^{\I_{\Pmc_1 \cup \Pmc_2}}$ and for all $B \prec A_1$, $B^{\J_1 \cup \J_2} = B^{\I_{\Pmc_1 \cup \Pmc_2}}$ and we are done.
		\end{itemize}
	\end{enumerate}
	Overall, this proves $\J_1 \cup \J_2 <_\CP \I_{\Pmc_1 \cup \Pmc_2}$ as desired.
\end{proof}

We are now ready to properly prove Lemma~\ref{lemma-criteria-combined}.

\begin{proof}[Proof of Lemma~\ref{lemma-criteria-combined}]
	``$1 \Rightarrow 2$''. 
	Assume there exists $\J \models \kb$ s.t.\ $\J <_\CP \I$.
	Based on $\J$, we build a subset $\Pmc \subseteq \domain{\J}$ containing:
	\begin{itemize}
		\item for each role $r$ s.t.\ $r^\J \neq \emptyset$, an element $w_r' \in (\exists r^-)^\J$;
		\item for each $A \in \Msf$ s.t.\ $A^\J \not\subseteq A^\I$, an element $e_A \in B^\J \setminus B^\I$ for some $B \prec A$ (Condition~3 in the definition of $\J <_\CP \I$ ensures existence of such $B$ and $e_A$);
		\item an element $e_\Msf \in A^\J \setminus A^\I$ for some $A \in \Msf$ s.t.\ $A^\J \subsetneq A^\I$ and for all $B \prec A$, $B^\J = B^\I$
		(Condition~4 in the definition of $\J <_\CP \I$ ensures existence of such $A$ and $e_\Msf$).
	\end{itemize}
	Notice $\Pmc$ has size at most $2\sizeof{\tbox} +1$.
	We now build $\J_e$ as:
	\begin{align*}
		\domain{\J_e} = \; & \domain{\I_{\Pmc \cup \{ e\}}}
		\\
		\cstyle{A}^{\J_e} = \; & \cstyle{A}^{\J} \cap \domain{\J_e}
		\\
		\rstyle{r}^{\J_e} = \; & \rstyle{r}^{\J} \cap (\indsof{\abox} \times \indsof{\abox}) 
		\\
		& \cup \{ (e, w_s') \mid e \in (\exists s)^\J, \tbox \models s \incl r \}
		\\
		& \cup \{ (w_s', e) \mid e \in (\exists s)^\J, \tbox \models s \incl r^- \}
	\end{align*}
	It is easily verified that $\J_e$ is a model of $\kb$, and we now prove $\J_e <_\CP \I_{\Pmc \cup \{ e\}}$.
	We check that all four conditions from the definition of $<_\CP$ are satisfied:
	\begin{enumerate}
		\item 
		By definition, we have $\domain{\J_e} = \domain{\I_{\Pmc \cup \{ e \}}}$.
		\item 
		Let $A \in \Fsf$. 
		Definitions of $\I_{\Pmc \cup \{ e \}}$ and $\J_e$ ensure $A^\I \cap {\domain{\I_{\Pmc \cup \{ e \}}}} = A^{\I_{\Pmc \cup \{ e \}}}$ and $A^\J \cap {\domain{\I_{\Pmc \cup \{ e \}}}} = A^{\J_e}$.
		From $\J <_\CP \I$, we get $A^{\I} = A^{\J}$, which thus yields $A^{\I_{\Pmc \cup \{ e \}}} = A^{\J_e}$.
		\item 
		Let $A \in \Msf$ such that $A^{\J_e} \not\subseteq A^{\I_{\Pmc \cup \{ e \}}}$.
		Therefore $A^{\J} \not\subseteq A^{\I}$, and recall we kept in $\Pmc$ an element $e_A \in B^\J \setminus B^\I$ for some $B \prec A$ to belong to $\Pmc$.
		Joint with $B^{\J_e} \subseteq B^{\I_{\Pmc \cup \{ e \}}}$ being trivial, $e_A$ additionally witnesses that $B^{\J_e} \subsetneq B^{\I_{\Pmc \cup \{ e \}}}$.
		\item
		Recall we kept in $\Pmc$ an element $e_\Msf \in A^\J \setminus A^\I$ for some $A \in \Msf$ s.t.\ $A^\J \subsetneq A^\I$ and for all $B \prec A$, $B^\J = B^\I$.
		It gives immediately that $A^{\J_e} \subsetneq A^{\I_{\Pmc \cup \{ e \}}}$ and for all $B \prec A$, $B^{\J_e} = B^{\I_{\Pmc \cup \{ e \}}}$.
	\end{enumerate}
	This proves $\J_e <_\CP \I_{\Pmc \cup \{ e \}}$.
%	It remains to prove that for all $e \in \domain{\I} \setminus \domain{\I_\Pmc}$, there exists $\J_{\Pmc, e} \models \kb$ with $\J_{\Pmc, e} <_\CP \I_{\Pmc \cup \{ e\} }$ and $\J_{\Pmc, e}|_{\domain{\J_\Pmc}} = \J_\Pmc$.
%	This is achieved by constructing $\J_{\Pmc, e}$ as $\J_\Pmc$ above, but from $\Pmc \cup \{ e \}$ instead of $\Pmc$.
	It is straightforward from the definition of each $\J_e$ that for all $e, e'$ in $\domain{\I}$, we have $\J_{e}|_{\domain{\I_\Pmc}} = \J_{e'}|_{\domain{\I_\Pmc}}$, concluding the proof of ``$1 \Rightarrow 2$''. 
	
	``$2 \Rightarrow 1$''. 
	Assume there exist $\Pmc \subseteq \domain{\I}$
	with $\sizeof{\Pmc} \leq 2\sizeof{\tbox} + 1$ and a
	family
	$(\Jmc_{e})_{e \in \domain{\I}}$ of models of \Kmc such that
	$\J_{ e} <_\CP \I_{\Pmc \cup \{ e\} }$ and
	$\J_{e}|_{\domain{\I_\Pmc}} =
	\J_{e'}|_{\domain{\I_\Pmc}}$ for all $e,e' \in \domain{\I}$.
	Consider such a $\Pmc \subseteq \domain{\I}$, and family of models $\J_{e}$ for each $e \in \domain{\I}$.
	We build:
	\[
	\J = \bigcup_{e \in \domain{\I}} \J_{e}
	\]
	It is clear $\domain{\J} = \domain{\I}$ and since all $\J_{e}$ agree on the shared domain $\domain{\I_\Pmc}$, we apply Lemma~\ref{lemma-portions-union} to obtain $\J <_\CP \I$.
\end{proof}

\thmcombinedupperdllitebool*
\begin{proof}
	We exhibit a $\NExpTime$ procedure to decide the complement of our problem, that is, existence of a countermodel for UCQ $q$ over $\dllitebool$ cKB $\circkb$.
	Our procedure starts by guessing an interpretation $\I$ whose domain has size at most $\abox + 2^{\sizeof{\tbox} \sizeof{q}}$.
	This can be done in exponentially many non-deterministic steps.
	It further checks whether $\I$ is a model of $\kb$ that does not entail $q$ and rejects otherwise.
	This can essentially be done naively in $\sizeof{\domain{\I}}^{\sizeof{\tbox}\sizeof{q}}$ deterministic steps, that is still simply exponential w.r.t.\ our input.
	The procedure finally checks whether $\I$ complies with $\CP$ by
	iterating over each $\Pmc$ with $\sizeof{\Pmc} \leq 2 \sizeof{\tbox} + 1$ and over each model $\J_\Pmc$ of $\kb$ s.t.\ $\J_\Pmc < \I_\Pmc$.
	If, for a choice of $\Pmc$ and $\J_\Pmc$, we can find a $\J_{\Pmc, e}$ for each $e \in \domain{\I} \setminus \domain{\I_\Pmc}$ s.t.\ $\J_{\Pmc, e} \models \kb$ with $\J_{\Pmc, e} <_\CP \I_{\Pmc \cup \{ e\} }$ and $\J_{\Pmc, e}|_{\domain{\J_\Pmc}} = \J_\Pmc$, then our procedure rejects.
	Otherwise, that is all choices of $\Pmc$ and $\J_\Pmc$ led to the existence of a $e \in \domain{\I} \setminus \domain{\I_\Pmc}$ without a fitting $\J_{\Pmc, e}$, then it accepts.
	Notice that: iterating over such $\Pmc$ can be done in $\sizeof{\domain{\I}}^{2 \sizeof{\tbox} + 1}$ iterations since we require $\sizeof{\Pmc} \leq 2 \sizeof{\tbox} + 1$.
	Computing $\I_\Pmc$ follows directly from the choice of $\Pmc$.
	Since each $\I_\Pmc$ has polynomial size, iterating over each $\J_\Pmc$ can be done naively with exponentially many steps.
	Further iterating over each $e \in \domain{\I} \setminus \domain{\I_\Pmc}$ can be done in $\sizeof{\domain{\I}}$ steps, which is at most exponential by construction.
	Since each $\I_{\Pmc \cup \{ e\} }$ has polynomial size, deciding the existence of $\J_{\Pmc, e}$ can be done naively in exponentially many steps.
	Overall, the procedure uses an exponential number of non-deterministic steps at the beginning and further performs several checks using exponentially many more deterministic steps.
	
	It remains to prove an accepting run exists iff there is a countermodel for $q$ over $\circkb$.
	If there exists an accepting run, then the corresponding guessed interpretation $\I$ is a model of $\kb$ that does not entail $q$, and it must also comply with $\CP$. Otherwise, the ``$1 \Rightarrow 2$'' direction from Lemma~\ref{lemma-criteria-combined} ensures the procedure would have rejected it.
	Conversely, if a countermodel exists, Lemma~\ref{lemma-bool-countermodel} ensures the existence of a countermodel $\I$ whose domain has exponential size.
	This $\I$ can be guessed by the procedure that checks whether it is indeed a model of $\kb$ not entailing $q$; hence, do not reject it at first.
	The ``$2 \Rightarrow 1$'' direction from Lemma~\ref{lemma-criteria-combined} further ensures $\I$ also passes the remaining check performed by the procedure; otherwise, it would contradict $\I$ being a model of $\circkb$.
\end{proof}

\thmcombinedlowerdllitepos*
\begin{proof}
	
	The proof proceeds by reduction from the complement of the $\NExpTime$-complete \succinct\tcol\ problem. %, known to be $\NEXP$-complete due to \cite{papadimitriou-succinct}.
	An instance of \succinct\tcol\ consists of a Boolean circuit $C$ with $2n$ input gates.
	The graph $G_C$ encoded by $C$ has $2^n$ vertices, identified by binary encodings on $n$ bits.
	Two vertices $u$ and $v$, with respective binary encodings $u_1 \dots u_n$ and $v_1 \dots v_n$, are adjacent in $G_C$ iff $C$ returns True when given as input $u_1 \dots u_n$ on its first $n$ gates and  $v_1 \dots v_n$ on the second half.
	The problem of deciding if $G_C$ is 3-colorable has been proven to be $\NExpTime$-complete in \cite{Papadimitriou1986}.
	
	Let $C$ be a Boolean circuit with $2n$ input gates.
%	To prove this result, we provide a polynomial time reduction from the complement of Succinct3COL, which is known to be \NExpTime-complete \cite{Papadimitriou1986}.
	Let $G = (V,E)$ be the corresponding graph with $V = \{v_1, v_2, \cdots, v_{2^n}\}$.
	We denote $\bar i$ the binary encoding on $n$ bits of vertex $v_i$.
	We also identify $\mn{t}$ (True) and $\mn{f}$ (False) with their usual binary valuation $1$ and $0$, respectively.
%	%
%	\textcolor{red}{Robin: Quentin said that I can assume $G$ to contain exactly $2^n$ vertices, although the sources allow for less vertices. As I have no references, I am not entirely convinced that this restriction is sound, but without it, the proof does not go through.}
%	%
%	A \emph{succinct representation} of $G$ is a circuit $C_G$ that computes the following function:
%	%
%	\[
%		C_G(\bar i, \bar j) =
%		\begin{cases}
%			\mn{t} & \text{if } (v_i,v_j) \in E               \\
%			\mn{f} & \text{if, otherwise, }(v_i,v_j) \notin E
%		\end{cases}
%	\]
%
%	\noindent The problem Succinct3COL is, given the succinct representation $C_G$ of a graph $G$, to decide whether $G$ is 3-colorable.
	We construct a circumscribed \dllitecore KB $\Circ(\Kmc)$ with $\Kmc = (\Tmc,\Amc)$ and a UCQ $q$ that encode a given problem instance.
	With the aim to restrict colors and truth values to those defined in the ABox (see axioms (\ref{ax:min_value_col})), we minimize exactly the concept name $\mn{Min}$ and let others vary freely.
	Our reduction starts by representing the colors (\ref{ax:colors_def}) and truth values (\ref{ax:values_def}) in the ABox.
	The role name $\mn{neq}$ makes the inequality relations within them explicit; see axioms (\ref{ax:neq_colors}) and (\ref{ax:neq_values}).
	\begin{align}
		\mn{Col}(c)                      & \text{ for all } c \in \{\mn{r},\mn{g},\mn{b}\}         \label{ax:colors_def}                             \\
		\mn{neq}(c,c')                & \text{ for all } c,c' \in \{\mn{r},\mn{g},\mn{b}\}  \text{ with } c \neq c'  \label{ax:neq_colors}                            \\
		\mn{Val}_b(\mn{val}_b)           & \text{ for all } b \in \{\mn{f},\mn{t}\}      \label{ax:values_def}                        \\
		\mn{neq}(\mn{val}_b, \mn{val}_{b'}) & \text{ for all } b,b' \in \{\mn{f},\mn{t}\} \text{ with } b \neq b'    \label{ax:neq_values} \\
		\mn{Min}(x)                      & \text{ for all } x \in \{\mn{r},\mn{g},\mn{b},\mn{val}_\mn{t},\mn{val}_\mn{f}\} \label{ax:min_value_col}
	\end{align}

	We aim countermodels to contain $2^{2n}$ elements that each encode a pair $(v_k,v_l) \in V^2$.
	Towards this goal, we lay the foundation to branch a binary tree of depth $n$ from a root $a_\mn{tree}$, which will be later enforced via the constructed UCQ further down.
	The concept names $(\mn{Index}_i)_{i = 1,\cdots,2n}$ encode the tree levels, which fork via the role names $\mn{next}_{i,\mn{t}}$ and $\mn{next}_{i,\mn{f}}$, encoding whether the $i$-th bit in $\bar k \cdot \bar l$ should be set to $\mn{t}$ or $\mn{f}$, respectively.
	The desired elements will therefore be (a subset of) the extension $\mn{Index}_{2n}$.  
	A role name $(\mn{hBit}_j)_{j = 1, \cdots, 2n}$ will later set the actual bit values.
	Note that axioms (\ref{ax:index_hBit}) require any $i$-th tree level to set the bits $1$ to $i$ so that the UCQ can later ensure the truth values to coincide with the choice via $\mn{next}$.
	Formally:
	\begin{align}
		\mathclap{\mn{Index}_0(a_\mn{tree})} \label{ax:tree_root}                                                                                                                                         \\
		\mn{Index}_{i-1}            & \sqsubseteq \exists \mn{next}_{i,b}               \label{ax:tree_branch}                                                                                                \\
		\exists \mn{next}^-_{i,b} & \sqsubseteq  \mn{Index}_{i}                                                 \label{ax:next_index}                                                                     \\
		\mn{Index}_i            & \sqsubseteq \exists \mn{hBit}_{j}                                                                   &  & \text{ for all } j \in \{1, \cdots, i\}  \label{ax:index_hBit} \\
		\exists \mn{hBit}_j^-   & \sqsubseteq \mn{Min}                                                                                &  & \text{ for all } j \in \{1, \cdots, 2n\} \label{ax:hBit_min}
	\end{align}
	for all $i \in \{1, \cdots, 2n\}$ and $b \in \{\mn{t}, \mn{f}\}$.

	We encode the color assignments of $(v_k,v_l)$ only at the $2n$-th level via the role name $\mn{hCol}$ for $v_k$ and $\mn{hCol}'$ for $v_l$:
	\begin{align}
		\mn{Index}_{2n}     & \sqsubseteq \exists \mn{hCol} & \mn{Index}_{2n}        & \sqsubseteq \exists \mn{hCol}' \label{ax:hCol_index} \\
		\exists \mn{hCol}^- & \sqsubseteq \mn{Min}          & \exists {\mn{hCol}'}^- & \sqsubseteq \mn{Min} \label{ax:hCol_min}
	\end{align}

	Finally, the computation of a gate $g$ in $C$ is enforced for each pair by an outgoing edge $\mn{gate}_g$ at the $2n$-th level.
	Add:
	\begin{align}
		\mn{Index}_{2n}     & \sqsubseteq \exists \mn{gate}_g \label{ax:index_gate}\\
		\exists \mn{gate}_g & \sqsubseteq \mn{Min} \label{ax:gate_min}
	\end{align}
	for all gates $g$ in $C$.

	Let the constructed UCQ $q$ be the disjunction over all subsequent queries.
	We first make sure that no color is used as a truth value (CQs (\ref{cq:hasBit_not_to_color}) and (\ref{cq:gate_not_to_color})) or vice-versa (CQs (\ref{cq:hasCol_not_to_val}) and (\ref{cq:hasCol2_not_to_val})):
	\begin{align}
		\exists x,y \, \mn{hBit}_j(x,y) \wedge \mn{Col}(y)  & \text{ for all } j \in \{1, \cdots, 2n\}     \label{cq:hasBit_not_to_color} \\
		\exists x,y \, \mn{gate}_g(x,y) \wedge \mn{Col}(y)  & \text{ for all gates } g \text{ in } G'   \label{cq:gate_not_to_color}      \\
		\exists x,y \, \mn{hCol}(x,y) \wedge \mn{Val}_b(y)  & \text{ for all } b \in \{\mn{t}, \mn{f}\} \label{cq:hasCol_not_to_val}      \\
		\exists x,y \, \mn{hCol}'(x,y) \wedge \mn{Val}_b(y) & \text{ for all } b \in \{\mn{t}, \mn{f}\} \label{cq:hasCol2_not_to_val}
	\end{align}

	We next simultaneously enforce that a) the structure constructed by axioms (\ref{ax:tree_root})--(\ref{ax:next_index}) really is a tree, and b) that the valuation required by axioms (\ref{ax:index_hBit}) and (\ref{ax:hBit_min}) is consistent with the branching of the tree.
	We achieve this via CQs (\ref{cq:next_correct_additional_bit}), which makes countermodels assign the bits by $\mn{hBit}$ as dictated by $\mn{next}$, and via CQs (\ref{cq:next_same_bits}), which makes countermodels propagate the bit assignment of a node downwards the tree to all successors:
	\begin{align}
		\begin{split}
			\exists x,y,z_1,z_2 \, & \mn{next}_{i-1,b}(x,y) \wedge \mn{hBit}_j(y,z_1) \\
			& \wedge \mn{neq}(z_1,z_2) \wedge \mn{Val}_b(z_2)
		\end{split} \label{cq:next_correct_additional_bit} \\
		\begin{split}
			\exists x,y,z_1,z_2 \, & \mn{next}_{i-1,b}(x,y) \wedge \mn{hBit}_j(x,z_1) \\
			& \wedge \mn{hBit}_j(x,z_2)  \wedge \mn{neq}(z_1,z_2)
		\end{split} \label{cq:next_same_bits}
	\end{align}
	for all $i \in \{1, \cdots, 2n\}$, $j \in \{1, \cdots, i\}$ and $b \in \{\mn{t}, \mn{f}\}$.
	Observe that the above indeed enforces a tree.

	We go on to construct CQs (\ref{cq:v_color_consistent}) and (\ref{cq:v_u_color_consistent}), which prohibit any two encoded pairs of vertices $(v,u)$ and $(v,u')$ or $(v,u)$ and $(u,u')$ to assign different colors to $v$ or $u$, respectively:
	\begin{align}
		\begin{split}
			\exists & x,y,c,d,z_1, \cdots, z_n \, \mn{hCol}(x,c) \wedge \mn{hCol}(y,d) \\
			& \wedge \mn{neq}(c,d) \wedge \bigwedge_{1 \leq j \leq n} \big(\mn{hBit}_j(y, z_j) \wedge \mn{hBit}_j(x,z_j) \big)
		\end{split} \label{cq:v_color_consistent} \\
		\begin{split}
			\exists & x,y,c,d,z_1, \cdots, z_n \, \mn{hCol}(x,c) \wedge \mn{hCol}'(y,d) \\
			& \wedge \mn{neq}(c,d) \wedge \bigwedge_{1 \leq j \leq n} \big(\mn{hBit}_j(y, z_j) \wedge \mn{hBit}'_{j+n}(x,z_j) \big)
		\end{split} \label{cq:v_u_color_consistent}
	\end{align}

	To ensure that the computation of the boolean circuit is consistent, we construct CQs restricting $\mn{gate}_g$ to follow the logical operator of $g$.
	For this, we assume w.l.o.g.\ that $C$ only contains unary NOT-gates, binary AND- and OR-gates, and $2n$ nullary INPUT-gates (each encoding a bit in $\bar k \cdot \bar l$).
	Given an INPUT-gate $g$ from $C$, we denote the index of the encoded bit from $\bar k \cdot \bar l$ with $i_g$.
	Construct, for each INPUT-gate $g$ from $C$, the CQ as given next:
	\begin{align}
		\begin{split}
			\exists x,y,z \, \mn{gate}_g(x,y) \wedge \mn{hBit}_{i_g}(x,z) \wedge \mn{neq}(y,z) \label{cq:input_gates}
		\end{split}
	\end{align}
	For all NOT-gates $g$ with their parent $g'$, construct
	\begin{align}
		\begin{split}
			\exists x,y \, \mn{gate}_g(x,y) \wedge \mn{gate}_{g'}(x,y) \label{cq:not_gate}
		\end{split}
	\end{align}
	For all AND-gates $g$ with parents $g_1,g_2$, construct
	\begin{align}
		\begin{split}
			\exists x,y,z \, & \mn{gate}_g(x,y) \wedge \mn{Val}_\mn{t}(y) \wedge \mn{gate}_{g_1}(x,z) \\
			& \wedge \mn{Val}_\mn{f}(z)
		\end{split} \\
		\begin{split}
			\exists x,y,z \, & \mn{gate}_g(x,y) \wedge \mn{Val}_\mn{t}(y) \wedge \mn{gate}_{g_2}(x,z) \\
			& \wedge \mn{Val}_\mn{f}(z)
		\end{split} \\
		\begin{split}
			\exists x,y,z \, & \mn{gate}_g(x,y) \wedge \mn{Val}_\mn{f}(y) \wedge \mn{gate}_{g_1}(x,z)  \\
			& \wedge \mn{Val}_\mn{t}(z) \wedge \mn{gate}_{g_2}(x,z)
		\end{split}
	\end{align}
	For all OR-gates $g$ with parents $g_1,g_2$, construct
	\begin{align}
		\begin{split}
			\exists x,y,z \, & \mn{gate}_g(x,y) \wedge \mn{Val}_\mn{f}(y) \wedge \mn{gate}_{g_1}(x,z) \\
			& \wedge \mn{Val}_\mn{t}(z)
		\end{split} \\
		\begin{split}
			\exists x,y,z \, & \mn{gate}_g(x,y) \wedge \mn{Val}_\mn{f}(y) \wedge \mn{gate}_{g_2}(x,z) \\
			& \wedge \mn{Val}_\mn{t}(z)
		\end{split} \\
		\begin{split}
			\exists x,y,z \, & \mn{gate}_g(x,y) \wedge \mn{Val}_\mn{t}(y) \wedge \mn{gate}_{g_1}(x,z)  \\
			& \wedge \mn{Val}_\mn{f}(z) \wedge \mn{gate}_{g_2}(x,z)
		\end{split} \label{cq:or_true_despite_both_false}
	\end{align}

	Finally, we rule out the existence of monochromatic edges in countermodels via CQ (\ref{cq:monochromatic_edge}):
	\begin{align}
		\exists x,y,z \, \mn{hCol}(x,y) \wedge \mn{hCol}'(x,y) \wedge \mn{gate}_{\dot g}(x,z)  \wedge \mn{Val}_\mn{t}(z) \label{cq:monochromatic_edge}
	\end{align}
	where we here and in what follows denote by $\dot g$ the output gate of $C$.

	%	Reduction from coSuccinct3COL: ABox encodes 2 Booleans + 3 colors as instances of the minimized predicate $M$. ABox also encode the root of a tree. TBox encodes a tree generating all couples of vertices $(u, v)$. Binary encoding is achieved by having roles pointing to instances of $M$. Picking colors of $u$ and $v$ at each end node is done similarly. Computing the Boolean circuit for each $(u, v)$ is done by having one role per gate of the circuit pointing to an instance of $M$.

	%The query matches if one of the following holds: a color is used as a Boolean or vice-versa; binary encoding is inconsistent with the branchings of the tree; end nodes define a inconsistent 3-coloring (ie there are two end nodes assigning two different colors to a same $u$); the computation of the Boolean circuit is inconsistent; or finally if there is a monochromatic edge.

	\begin{lemma}
		$G$ is 3-colorable iff $\Circ(\Kmc) \not \models q$.
	\end{lemma}
	``$\Rightarrow$''.
	Let $G$ be 3-colorable.
	Then there exists a 3-coloring $\pi : V \rightarrow \{\mn{r},\mn{g},\mn{b}\}$ such that $\pi(v) \neq \pi(u)$ for all $(v,u) \in V$.
	To show that $\Circ(\Kmc) \not \models q$, we construct a countermodel \Imc of $\Circ(\Kmc)$ as follows.
	Let $X \coloneqq \bigcup_{j = 1, \cdots, 2n} \{a_{j,1}, \cdots, a_{j,2^j}\}$; then set

	\begin{align*}
		\Delta^\Imc \coloneqq          & \Ind(\Amc) \cup X                                             \\
		A^\Imc \coloneqq          & \{ a \mid A(a) \in \Amc\}                                     \\
		\mn{neq}^\Imc \coloneqq        & \{ (a,b) \mid \mn{neq}(a,b) \in \Amc\}                        \\
		\mn{Index}^\Imc_i \coloneqq    & \{a_{i,1}, \cdots, a_{i,2^i}\}                                \\
		\mn{next}^\Imc_{i,\mn{t}} \coloneqq & \bigcup_{j = 1, \cdots, 2^{i-1}} \{(a_{i-1,j}, a_{i,2j})\}     \\
		\mn{next}^\Imc_{i,\mn{f}} \coloneqq & \bigcup_{j = 1, \cdots, 2^{i-1}} \{(a_{i-1,j}, a_{i,2j - 1})\} \\
		\begin{split}
			\mn{hBit}^\Imc_i \coloneqq &  \bigcup_{j = 1, \cdots, 2^{i-1}} \big( \{(a,\mn{val}_\mn{t}) \mid a \in  R(a_{i,2j})\} \\
			& \phantom{\bigcup_{1 \leq j \leq 2^{i-1}}\big(} \cup \{(a,\mn{val}_\mn{f}) \mid a \in  R(a_{i,2j-1})\} \big)
		\end{split}
	\end{align*}
	for all concept names $A \in \{\mn{Col}, \mn{Val}_\mn{t},\mn{Val}_\mn{f},\mn{Min},\mn{Index}_0\}$ and $i\in \{1, \cdots, 2n\}$, where we use
	\begin{itemize}
		\item $a_{0,1}$ to denote $a_\mn{tree}$, and
		\item $R(a_{k,l})$ to denote the set of instances that are reachable in $\Imc$ from $a_{k,l} \in X$ via the family of role names $\mn{next}_{i,\mn{t}}$ and $\mn{next}_{i,\mn{f}}$ (including $a_{k,l}$ itself).
	\end{itemize}
	We furthermore set  $\mn{hCol}^\Imc, {\mn{hCol}'}^\Imc$ as follows.
	Given some $a_{2n,i} \in X$ with $i \in \{1, \cdots 2^{2n}\}$, we denote by $\vartheta(a_{2n,i})$ the encoded pair $(v_k,u_l) \in V^2$, i.e., such that for all $j \in \{1, \cdots, 2n\}$, we have $(a_{2n,i}, \mn{val}_b) \in \mn{hBit}_j^\Imc$ iff the $j$-th bit in $\bar k \cdot \bar l$ is $b$ with $b \in \{\mn{t},\mn{f}\}$.
	\begin{align*}
		\mn{hCol}^\Imc \coloneqq    & \left\{ \big(a_{2n,i}, \pi(v)\big) \mid \vartheta(a_{2n,i}) = (v,u) \right\} \\
		{\mn{hCol}'}^\Imc \coloneqq & \left\{ \big(a_{2n,i}, \pi(u)\big) \mid \vartheta(a_{2n,i}) = (v,u) \right\}
	\end{align*}
	Finally, we set $\mn{gate}_g$ for all gates $g$ in $G_C$.
	We denote the sub-circuit of $G_C$ that contains exactly $g$ and all its ancestors with $G_C^g$.
	Note that the output gate of $G_C^g$ is $g$, i.e., $G_C^g(\bar k, \bar l)$ computes the value of $g$ in $G_C$ given the input $(\bar k, \bar l)$.
	Then, for all gates $g$, set:
	\begin{align*}
		\begin{split}
			\mn{gate}_g^\Imc \coloneqq & \{(a_{2n,i}, \mn{val}_b) \mid \vartheta(a_{2n,i}) = (v_k,u_l)  \\
			&\phantom{\{(a_{2n,i}, \mn{val}_\mn{t}) \mid} \text{ and } G_C^g(\bar k, \bar l) = b \} \\
		\end{split}
	\end{align*}

	It is obvious that \Imc is a model of \Kmc.
	As $a \in \mn{Min}^\Imc$ iff $\mn{Min}(a)$ for all $a \in \Delta^\Imc$, and $\mn{Min}$ is the only minimized concept, \Imc must furthermore be minimal.

	To see that $\Imc \not \models q$, it is readily checked that
	\begin{itemize}
		\item \Imc by definition has no answer to CQs (\ref{cq:hasBit_not_to_color})--(\ref{cq:v_u_color_consistent}),
		\item additionally, \Imc has no answer to CQs (\ref{cq:input_gates})--(\ref{cq:or_true_despite_both_false}), as otherwise, the computation of $G_C$ would be inconsistent, and
		\item finally, \Imc has no answer to CQ (\ref{cq:monochromatic_edge}), as otherwise, $\pi$ would not be a 3-coloring of $G$.
	\end{itemize}

%	\textcolor{red}{Robin: Not sure whether the above suffices or if I need to dig into all the details}

	\smallskip

	``$\Leftarrow$''.
	Let $\Circ(\Kmc)\not \models q$.
	Then there is a model \Imc of $\Circ(\Kmc)$ such that $\Imc \not \models q$.
	We aim to extract a function $\pi : V \rightarrow \{\mn{r},\mn{g},\mn{b}\}$ and to show that $\pi$ is indeed a 3-coloring of $G$.
	This is rather laborious, as we have to prepare the final argument in five steps. In Claim (\ref{claim:relation_ranges})--(\ref{claim:output_gate_edge}), respectively, we
	\begin{enumerate}
		\item briefly argue that $\mn{hBit}$ and $\mn{gate}$ have the range $\{\mn{val}_\mn{t}, \mn{val}_\mn{f}\}$ and that $\mn{hCol}$ and $\mn{hCol}'$ have the range $\{\mn{r},\mn{g},\mn{b}\}$, which will be convenient later on,
		\item identify within \Imc the intended tree-structure,
		\item show that each leaf indeed encodes a pair $(v_k,v_l) \in V^2$, setting precisely the bits from $\bar k \cdot \bar l$,
		\item extract $\pi$ from \Imc and show that it is sound in the sense that any two leaves that encode the same vertex also assign it the same color, and
		\item proof that the leaves correctly compute all gates.
	\end{enumerate}
	We start with the ranges of $\mn{hBit}, \mn{gate}$ and $\mn{hCol}$:
	\begin{claim} \label{claim:relation_ranges}
		The following properties hold.
		\begin{itemize}
			\item both $(x,y) \in \mn{hBit}^\Imc_i$ and $(x,y) \in \mn{gate}^\Imc_g$ entail $y \in \{\mn{val}_\mn{t}, \mn{val}_\mn{f}\}$ for all $i \in \{1, \cdots, 2n\}$ and gates $g$ in $C$, and
			\item both $(x,y) \in \mn{hCol}^\Imc$ and $(x,y) \in {\mn{hCol}'}^\Imc$ entail $y \in \{\mn{r},\mn{g},\mn{b}\}$.
		\end{itemize}
	\end{claim}
	\noindent The proof is simple: As \Imc is a model of \Amc, axioms (\ref{ax:min_value_col}) imply $\{\mn{r},\mn{g},\mn{b},\mn{val}_\mn{t},\mn{val}_\mn{f}\} \subseteq \mn{Min}^\Imc$.
	Furthermore, it is obvious that there cannot be any $a \in \mn{Min}^\Imc$ with $\mn{Min}(a) \notin \Amc$, since \Imc would otherwise not be $<_\CP$ minimal (it would then be straightforward to construct a smaller model).
	Ergo, $\mn{Min}^\Imc = \{\mn{r},\mn{g},\mn{b},\mn{val}_\mn{t},\mn{val}_\mn{f}\}$.

	The rest of the claim follows from axioms (\ref{ax:colors_def}), (\ref{ax:values_def}), (\ref{ax:hBit_min}), (\ref{ax:hCol_min}), (\ref{ax:gate_min}), CQs (\ref{cq:hasBit_not_to_color})--(\ref{cq:hasCol2_not_to_val}), and $\Imc \not \models q$:
	For example, in the case of $\mn{hCol}$, consider some $(x,y) \in \mn{hCol}^\Imc$.
	By axiom (\ref{ax:hCol_min}), we have that $y \in\mn{Min}^\Imc$.
	CQ (\ref{cq:hasCol_not_to_val}) and the fact that $\Imc \not \models q$ together yield $y \in\mn{Min}^\Imc \setminus (\mn{Val}_\mn{t} \cup \mn{Val}_\mn{f})$.
	As $\{\mn{val}_\mn{t}, \mn{val}_\mn{f}\} \subseteq \mn{Val}_\mn{t} \cup \mn{Val}_\mn{f}$ by axioms (\ref{ax:values_def}), we thus have that $y \in \{\mn{r},\mn{g},\mn{b}\}$.
	The other cases are analogous.

	This finishes the proof of Claim (\ref{claim:relation_ranges}).

	\smallskip

	We go on by identifying within \Imc the intended tree structure:
	\begin{claim}
		For all $i \in \{1, \cdots, 2n\}$ there is a set $Y_i \subseteq \mn{Index}^\Imc_i$ that satisfies the following properties:

		\begin{enumerate} \label{claim:tree_induction}
			\item for all $y \in Y_i$, there is exactly one \emph{parent $p \in Y_{i-1}$ of $y$} with $(p,y) \in \mn{next}_{i-1,b}^\Imc$ for some $b \in \{\mn{t}, \mn{f}\}$ (we set $Y_0 = \{a_\mn{tree}\}$),
			\item for all $y \in Y_i$ and $j \in \{1, \cdots, i \}$, there is exactly one $b \in \{\mn{t}, \mn{f}\}$ such that $(y, \mn{val}_n) \in \mn{hBit}_j$,
			\item for all $x, y \in Y_i$ with $x \neq y$, there is some $j \in \{1, \cdots, i\}$ such that $(x, \mn{val}_\mn{t}) \in \mn{hBit}_j$ iff $(y, \mn{val}_\mn{f}) \in \mn{hBit}_j$, and
			\item $|Y_i| = 2^i$.
		\end{enumerate}
	\end{claim}
	\noindent The proof of Claim (\ref{claim:tree_induction}) goes via induction over $i$:
	\begin{description}
		\item[Base case ($i=1)$.]
			Axioms (\ref{ax:tree_root})--(\ref{ax:next_index}) require the existence of some $x,y \in \mn{Index}_1^\Imc$ such that $(a_\mn{tree},x)\in\mn{next}_{1,\mn{t}}^\Imc$ and $(a_\mn{tree},y)\in\mn{next}_{1,\mn{f}}^\Imc$.
			Set $Y_1 = \{x,y\}$.
			Property 1.\ of Claim (\ref{claim:tree_induction}) obviously holds as $a_\mn{tree}$ is, on the one hand, the only element in $Y_0$, and, on the other hand, the parent of both $x$ and $y$.
			Together with Claim (\ref{claim:relation_ranges}), axioms (\ref{ax:neq_values}), and (\ref{ax:index_hBit}), and CQs (\ref{cq:next_correct_additional_bit}) (and the fact that $\Imc \not \models q$), we have that $(x, \mn{val}_\mn{t}) \in \mn{hBit}_1^\Imc$ and $(y, \mn{val}_\mn{f}) \in \mn{hBit}_1^\Imc$, while $(x, \mn{val}_\mn{f}) \notin \mn{hBit}_1^\Imc$ and $(y, \mn{val}_\mn{t}) \notin \mn{hBit}_1^\Imc$, i.e., also properties 2.\ and 3.\ hold.
			The above furthermore entails $x \neq y$, which is why also property 4.\ must hold.
		\item[Induction step ($i > 1$).]
			By the induction hypothesis, there is a set $Y_{i-1}$ with the claimed properties.
			For all $y \in Y_{i-1}$, axioms (\ref{ax:tree_root})--(\ref{ax:next_index}) entail the existence of elements $a_y,a_y' \in \mn{Index}_i^\Imc$ such that $(y,a_y)\in\mn{next}_{i,\mn{t}}^\Imc$ and $(y,a'_y)\in\mn{next}_{i,\mn{f}}^\Imc$.
			Similar as in the base case, we deduct that $(a_y, \mn{val}_\mn{t}) \in \mn{hBit}_i^\Imc$ and $(a'_y, \mn{val}_\mn{f}) \in \mn{hBit}_i^\Imc$, while $(a_y, \mn{val}_\mn{f}) \notin \mn{hBit}_i^\Imc$ and $(a'_y, \mn{val}_\mn{t}) \notin \mn{hBit}_i^\Imc$ $(\dag)$ via Claim (\ref{claim:relation_ranges}), axioms (\ref{ax:neq_values}) and (\ref{ax:index_hBit}), and CQs (\ref{cq:next_correct_additional_bit}) (and the fact that $\Imc \not \models q$).
			Set $Y_i = \bigcup_{y \in Y_{i-1}} \{a_y,a_y'\}$.

			To see that $Y_i$ satisfies property 1., assume to the contrary that there is some $a \in Y_i$ with two parents from $Y_{i-1}$, i.e., that there are two elements $y,y' \in Y_{i-1}$ such that $(y,a) \in \mn{next}_{i-1,b}^\Imc$ and $(y',a) \in \mn{next}_{i-1,b'}^\Imc$ for some $b,b' \in \{\mn{t},\mn{f}\}$.
			By property 3.\ of the induction hypothesis, there must be some $j \in \{1,\cdots,i-1\}$ such that $(x, \mn{val}_\mn{t}) \in \mn{hBit}_j^\Imc$ iff $(x', \mn{val}_\mn{f}) \in \mn{hBit}_j^\Imc$.
			Furthermore observe that Claim (\ref{claim:relation_ranges}) and axioms (\ref{ax:index_hBit}) require $a$ to assign the $j$-th bit, i.e., we have $(a, \mn{val}_\mn{t}) \in \mn{hBit}_j^\Imc$ or $(a, \mn{val}_\mn{f}) \in \mn{hBit}_j^\Imc$.
			In either case, due to axioms (\ref{ax:neq_values}), we can find a homomorphism from CQ (\ref{cq:next_same_bits}) to \Imc, which contradicts the fact that \Imc is a countermodel to $q$.
			Ergo, $Y_i$ must satisfy property 1.

			Property 2.\ follows, in case of $j = i$, from $(\dag)$, and, if otherwise $j \in \{1,\cdots,i-1\}$, from $Y_{i-1}$ satisfying property 2.\ and the fact that Claim (\ref{claim:relation_ranges}), axioms (\ref{ax:neq_values}) and (\ref{ax:index_hBit}), and CQs (\ref{cq:next_same_bits}) require all $a \in Y_i$ to assign the bits $1, \cdots, i-1$ exactly as their parents.

			For property 3, consider some $a, a' \in Y_i$ with $a \neq a'$.
			If $a$ and $a'$ have the same parent $x$, property 3.\ follows from $(\dag)$ and property 1.
			Otherwise, if $a$ has a parent $x$ and $a'$ has a parent $y$ such that $x \neq y$, observe that property 3.\ of the induction hypothesis implies the existence of some $j \in \{1,\cdots,i-1\}$ such that $(x, \mn{val}_\mn{t}) \in \mn{hBit}_j$ iff $(y, \mn{val}_\mn{f}) \in \mn{hBit}_j$.
			Property 3.\ then follows from the fact that Claim (\ref{claim:relation_ranges}), axioms (\ref{ax:neq_values}) and (\ref{ax:index_hBit}), and CQs (\ref{cq:next_same_bits}) require $a$ and $a'$ to assign the bits $1, \cdots, i-1$ exactly as their parents.

			Regarding property 4., observe that by $(\dag)$, $Y_i$ contains two elements $a_y,a_y'$ with $a_y \neq a_y'$ for each $y \in Y_{i-1}$.
			Given any two elements $x,y \in Y_{i-1}$, it is furthermore easy to see that $\{a_x,a_x'\}$ and $\{a_y,a_y'\}$ are disjoint, as by property 2.\ and 3.\ of the induction hypothesis, there must be some bit $j \in \{1,\cdots,i-1\}$ that $x$ and $y$ assign differently, which subsequently must then also be assigned differently by $\{a_x,a_x'\}$ and $\{a_y,a_y'\}$ due to Claim (\ref{claim:relation_ranges}), axioms (\ref{ax:neq_values}) and (\ref{ax:index_hBit}), and CQs (\ref{cq:next_same_bits}).
			As, thus, $|Y_i| = 2 |Y_{i-1}|$, property 4.\ of the induction hypothesis implies $|Y_i| = 2^i$.
	\end{description}
	This finishes the proof of Claim (\ref{claim:tree_induction}).

	\smallskip

	We go on to identify the instances in \Imc that encode pairs of vertices:
	\begin{claim} \label{claim:identify_encoding_pairs}
		We can identify a set $Y \subseteq \mn{Index}_{2n}^\Imc$ and a bijective function $\vartheta : Y \rightarrow V^2$ such that $\vartheta(x) = (v_k,u_l)$ implies $(x, \mn{val}_b) \in \mn{hBit}_i^\Imc$ iff the $i$-th bit in $\bar k \cdot \bar l$ is $b$ for all $b \in \{\mn{t},\mn{f}\}$ and $i \in \{1, \cdots, 2n\}$.
	\end{claim}

	\noindent Claim (\ref{claim:identify_encoding_pairs}) builds upon Claim (\ref{claim:tree_induction}); set $Y = Y_{2n}$.
	By property 2.\ of Claim (\ref{claim:tree_induction}), each $y \in Y$ assigns a unique $b \in \{\mn{t},\mn{f}\}$ to every $i$-th bit with  $i \in \{1, \cdots, 2n\}$, encoded via $(y, \mn{val}_b) \in \mn{hBit}_i^\Imc$.
	Ergo, we can find a function $\vartheta : Y \rightarrow V^2$ such that $\vartheta(y) = (v_k,u_l)$ implies $(y, \mn{val}_b) \in \mn{hBit}_i^\Imc$ iff the $i$-th bit in $\bar k \cdot \bar l$ is $b$ for all $b \in \{\mn{t},\mn{f}\}$ and $i \in \{1, \cdots, 2n\}$.

	Note that $\vartheta$ must be surjective, as by $|Y| = 2^{2n}$ (property 4\ of Claim (\ref{claim:tree_induction})) and the fact that all $x,y \in Y$ pairwise assign at least one bit differently (property 3.\ of Claim (\ref{claim:tree_induction})).

	To see that $\vartheta$ is injective, consider some $x,y \in Y$ with $\vartheta(x) = (v_k,u_l) = \vartheta(y)$.
	By definition of $\vartheta$, we have that $(x, \mn{val}_b) \in \mn{hBit}_i^\Imc$ iff $(y, \mn{val}_b) \in \mn{hBit}_i^\Imc$ for all with $b \in \{\mn{t},\mn{f}\}$ and $i \in \{1, \cdots, 2n\}$, and, together with property 2 \ of Claim (\ref{claim:tree_induction}), even that $(x, \mn{val}_\mn{t}) \in \mn{hBit}_i^\Imc$ iff $(y, \mn{val}_\mn{f}) \notin \mn{hBit}_i^\Imc$.
	Property 3.\ of Claim (\ref{claim:tree_induction}) then entails $x = y$.

	This finishes the proof of Claim (\ref{claim:identify_encoding_pairs}).

	\smallskip

	We go on to extract $\pi$ from \Imc and show that \Imc is sound in the sense that any two elements $x,y \in Y$ that encode the same vertex also assign it the same color as defined by $\pi$.

	\begin{claim} \label{claim:sound_colors}
		The relation $\pi : V \rightarrow \{\mn{r},\mn{g},\mn{b}\}$ with
		\begin{align*}
			\begin{split}
				\pi(v) \coloneqq \{c \in \{\mn{r},\mn{g},\mn{b}\} \mid & \exists y \in Y \text{ such that } \vartheta(y) = (v,u) \\
				& \text{ and } (y, c) \in \mn{hCol}^\Imc \}.
			\end{split}
		\end{align*}
		is a function such that $(y,c_1) \in \mn{hCol}^\Imc$ and $(y,c_2) \in {\mn{hCol}'}^\Imc$ hold for all $y \in Y$ with $\vartheta(y) = (v,u)$, $\pi(v) = c_1$ and $\pi(u) = c_2$.
	\end{claim}
	\noindent Indeed, $\pi$ is a function:
	On one hand, Claim (\ref{claim:relation_ranges}) and axioms (\ref{ax:hCol_index}) ensure the existence of some $c,d \in \{\mn{r},\mn{g},\mn{b}\}$ such that $(y, c) \in \mn{hCol}^\Imc$ and $(y, d) \in \mn{hCol}'^\Imc$ for all $y \in Y$.
	On the other hand, $\pi(y)$ is unique for all $y \in Y$:
	Assume to the contrary that there are two elements $y,y' \in Y$ such that $\vartheta(y) = (v,u)$ with $(y, c) \in \mn{hCol}^\Imc$ and $\vartheta(y') = (v,u')$ with $(y', c') \in \mn{hCol}^\Imc$ and $c' \neq c$.
	By definition of $\vartheta$, $y$ and $y'$ assign the bits with $1,\cdots,n$ the same, i.e., $(y,z) \in \mn{hBit}_i^\Imc$ iff $(y',z) \in \mn{hBit}_i^\Imc$.
	Furthermore, $c' \neq c$ yields $(c',c) \in \mn{neq}^\Imc$ via axioms (\ref{ax:neq_colors}).
	Then, however, there must be a homomorphism from CQ (\ref{cq:v_color_consistent}) to \Imc, which contradicts the fact that $\Imc \not \models q$.
	
	Now, consider some $y \in Y$ with $\vartheta(y) = (v,u)$, $\pi(v) = c_1$ and $\pi(u) = c_2$.
	We first show that $(y,c_1) \in \mn{hCol}^\Imc$.
	The definition of $\pi$ requires the existence of some $y' \in Y$ such that $\vartheta(y') = (v,u')$ and $(y',c_1) \in \mn{hCol}^\Imc$, while there must also be some $c \in \{\mn{r},\mn{g},\mn{b}\}$ such that $(y,c) \in \mn{hCol}^\Imc$ via Claim (\ref{claim:relation_ranges}) and axioms (\ref{ax:hCol_index}).
	By $\vartheta(y) = (v,u)$ and $\vartheta(y') = (v,u')$, Claim (\ref{claim:identify_encoding_pairs}) implies that $(y, \mn{val}_b) \in \mn{hBit}_i^\Imc$ iff $(y', \mn{val}_b) \in \mn{hBit}_i^\Imc$ for all $i \in \{1, \cdots, n\}$ and $b \in \{\mn{t},\mn{f}\}$.
	Then, we have that $(c_1,c) \notin \mn{neq}^\Imc$ via CQs (\ref{cq:v_color_consistent}) and the fact that $\Imc \not \models q$.
	Ergo, by Claim (\ref{claim:relation_ranges}), and axioms (\ref{ax:neq_colors}) and (\ref{ax:hCol_index}), we have that $c = c_1$, i.e., $(y,c_1) \in \mn{hCol}^\Imc$.

	We go on to show that $(y,c_2) \in {\mn{hCol}'}^\Imc$.
	Again, the definition of $\pi$ requires the existence of some $y' \in Y$ such that $\vartheta(y') = (u,u')$ and $(y',c_2) \in \mn{hCol}^\Imc$, while there must also be some $c \in \{\mn{r},\mn{g},\mn{b}\}$ such that $(y,c) \in {\mn{hCol}'}^\Imc$ via Claim (\ref{claim:relation_ranges}) and axioms (\ref{ax:hCol_index}).
	By $\vartheta(y) = (v,u)$ and $\vartheta(y') = (v,u')$, Claim (\ref{claim:identify_encoding_pairs}) implies that $(y, \mn{val}_b) \in \mn{hBit}_{i+n}^\Imc$ iff $(y', \mn{val}_b) \in \mn{hBit}_i^\Imc$ for all $i \in \{1, \cdots, n\}$ and $b \in \{\mn{t},\mn{f}\}$.
	Then, we have that $(c_2,c) \notin \mn{neq}^\Imc$ via CQs (\ref{cq:v_u_color_consistent}) and the fact that $\Imc \not \models q$.
	Ergo, by Claim (\ref{claim:relation_ranges}), and axioms (\ref{ax:neq_colors}) and (\ref{ax:hCol_index}), we have that $c = c_1$, i.e., $(y,c_1) \in {\mn{hCol}'}^\Imc$.

	This finishes the proof of Claim (\ref{claim:sound_colors}).

	\smallskip

	As a last step before proving that $\pi$ indeed is a 3-coloring, we need to argue that the computation of the logical gates within \Imc is sound.

	\begin{claim} \label{claim:output_gate_edge}
		For all $y \in Y$, we have that $\vartheta(y) \in E$ implies $(y, \mn{var}_\mn{t}) \in \mn{gate}_{\dot g}^\Imc$, where $\dot g$ is the output gate of $C$.
	\end{claim}
	\noindent As $\vartheta(y) \in E$ implies $C^{\dot g}(\bar k,\bar l) =  \mn{t}$, it suffices to show that $C^g(\bar k,\bar l) =  b$ implies $(y, \mn{var}_b) \in \mn{gate}_g^\Imc$ for all $y \in Y$ with $\vartheta(y) = (u_k,v_l)$, gates $g$ in $C$ and $b \in \{\mn{t}, \mn{f}\}$.
	We do this per induction over the structure of $C^g$:
	\begin{description}
		\item[$g$ is an INPUT gate.]
			Let $C^g(\bar k,\bar l) =  b$.
			Then, as $g$ is an INPUT gate, the $i_g$-th bit in $\bar k \cdot \bar l$ must be $b$.
			Thus, $(y, \mn{var}_b) \in \mn{hBit}_{i_g}^\Imc$ by definition of $\vartheta$.
			Claim (\ref{claim:relation_ranges}) and axioms (\ref{ax:index_gate}) entail $(y, \mn{var}_{b'}) \in \mn{gate}_g^\Imc$ for some $b' \in \{\mn{t}, \mn{f}\}$.
			Finally, $(y, \mn{var}_b) \in \mn{hBit}_{i_g}^\Imc$, axioms (\ref{ax:neq_values}), CQs (\ref{cq:input_gates}), and the fact that $\Imc \not \models q$ entail $b' = b$, i.e., $(y, \mn{var}_b) \in \mn{gate}_g^\Imc$.
		\item[$g$ is a NOT gate with parent $g'$.]
			Let $C^g(\bar k,\bar l) =  b$.
			As $g$ is a NOT gate with parent $g'$, we have that $C^{g'}(\bar k,\bar l) =  b'$ for some $b' \in \{\mn{t}, \mn{f}\}$ such that $b' \neq b$.
			By the induction hypothesis, we then have that $(y,\mn{var}_{b'}) \in \mn{gate}_{g'}^\Imc$.
			Claim (\ref{claim:relation_ranges}) and axioms (\ref{ax:index_gate}) entail $(y, \mn{var}_{b''}) \in \mn{gate}_g^\Imc$ for some $b'' \in \{\mn{t}, \mn{f}\}$.
			Due to $b' \neq b$, CQs (\ref{cq:not_gate}) and the fact that $\Imc \not \models q$, it must be so that $b'' = b$, i.e., $(y, \mn{var}_b) \in \mn{gate}_g^\Imc$.
		\item[$g$ is a AND or OR gate.]
			We omit the details, as these cases are very similar to the NOT case, except that the respective semantics of the logical operators need to be applied.
	\end{description}

	We are now in the position to show that $\pi$ indeed is a 3-coloring.
	Assume to the contrary that there is an edge $(v,u) \in E$ with $\pi(v) = \pi(u) \coloneqq c$.
	Since $\theta$ is a bijection as of Claim (\ref{claim:identify_encoding_pairs}), there exists a unique $y \in Y$ such that $\vartheta(y) = (v,u)$.
	We have $(y,\pi(v)) \in \mn{hCol}^\Imc$ and $(y,\pi(u)) \in {\mn{hCol}'}^\Imc$ by Claim (\ref{claim:sound_colors}), i.e., $(y,c) \in \mn{hCol}^\Imc$ and $(y,c) \in {\mn{hCol}'}^\Imc$.
	Furthermore, by Claim (\ref{claim:output_gate_edge}), $(v,u) \in E$ entails $(y, \mn{var}_\mn{t}) \in \mn{gate}_{\dot g}^\Imc$.
	Together with axioms (\ref{ax:values_def}), there must be a homomorphism from CQ (\ref{cq:monochromatic_edge}) to $\Delta^\Imc$.
	However, this contradicts the fact that \Imc is a countermodel to $q$.
	Ergo, $\pi$ must indeed be a 3-coloring, i.e., $G$ is 3-colorable.
\end{proof}

\section{Proofs for Section~\ref{subsection-dllite-data}}

\lemmacriteriadata*
\begin{proof}
	Before proving the lemma, we recall the set $E$ gathers elements $e_{t_1, t_2}$ which will serve as references for others with
	 same types.
	 To lighten notation, we introduce the mapping $\refmap : e \mapsto e_{\atypeinof{\abox}{e}, \typeinof{\I}{e}}$ defined on $\domain{\I}$.
	 
	``$1 \Rightarrow 2$''. 
	Assume $\Imc \models \circkb$.
	Consider $\Pmc \subseteq \domain{\I}$ s.t.\ $\sizeof{\Pmc} \leq 2\sizeof{\tbox} +1$.
	We first verify that $\I_\Pmc$ models $\kb_\Pmc$:
	\begin{itemize}
		\item $\I_\Pmc$ models $\abox_\Pmc$ as it inherits interpretations of concepts on $\indsof{\abox'}$ from $\I$, which is a model of $\abox$.
		\item Axioms in $\tbox$ with shape $\axtop$, $\axand$, $\axnotright$ or $\axnotleft$ are satisfied since $\I_\Pmc$ inherits interpretations of concept names from $\I$, which is a model of $\tbox$.
		\item Axioms in $\tbox$ with shape $A \incl \exists r$ are witnessed with an $r$-edge pointing to $w_r$.
		\item Axioms in $\tbox$ with shape $\exists r \incl A$ are satisfied since every element in $\I_\Pmc$ receiving some $r$-edge already received some in $\I$ (and interpretations of concept names are preserved).
		\item Role inclusions $r \incl s$ are satisfied directly from the definition of $s^{\Imc_\Pmc}$.
	\end{itemize}
	It remains to prove that $\I_\Pmc$ also complies with $\CP$.
	Assume to the contrary that there exists a model $\J'$ of $\kb_\Pmc$ with $\J' <_\CP \I_\Pmc$.
	Notice that, for each role $r$ s.t.\ $r^{\J'} \neq \emptyset$, there must be an element $w_r' \in (\exists r^-)^{\J'}$.
	We can chose such an element $w_r'$ for each such role $r$, and build the following interpretation $\J$:
	\begin{align*}
		\domain{\J} = \; & \domain{\I}
		\\
		\cstyle{A}^{\J} = \; & \cstyle{A}^{\J'} \cup \{ e \in \domain{\I} \setminus \domain{\J'} \mid \refof{e} \in A^{\J'} \}
		\\
		\rstyle{r}^{\J} = \; & \{ (a, b) \mid \kb \models r(a, b) \} \\
		&
		\cup \{ (e, w_s') \mid \refof{e} \in (\exists s)^{\J'}, \tbox \models s \incl r \}
		\\
		& \cup \{ (w_s', e) \mid \refof{e} \in (\exists s)^{\J'}, \tbox \models s \incl r^- \}
	\end{align*}
	It is easily verified that $\J$ is a model of $\kb$, the most interesting cases being axioms in $\tbox$ with shape either $A \sqsubseteq \exists r$ or $\exists r \sqsubseteq A$.
	The former are satisfied using the witness $w_r$.
	The latter, when triggered on $a \in \domain{\I} \setminus \domain{\J'}$ due to a pair $(a, b)$ s.t.\ $\kb \models r(a, b)$, hold thanks to $\refof{a}$ having same ABox-type as $a$.
%	{\color{red}(Quentin: Maybe I should elaborate? This is where we rely on $\abox_\Pmc$ and ABox-types.)}, 
%	\textcolor{blue}{Robin: I think maybe for axioms of the form $A \sqsubseteq \exists r$ and $\exists r \sqsubseteq A$; the others are obvious.}
	We now prove $\J <_\CP \I$, which will contradict $\I \models \circkb$.
	It suffices to prove that for each concept name $A$ and $\odot \in \{\subseteq, \supseteq\}$, we have $A^{\J} \odot A^\Imc$ iff $A^{\Jmc'} \odot A^{\I_\Pmc}$.
	Let $A$ be a concept name.
	We prove the claim for $\odot =\; \subseteq$ only; for $\odot =\; \supseteq$, the arguments are similar.
	
	``$\Rightarrow$''.
	Let $A^{\J} \subseteq A^\I$ and $d \in A^{\J'}$.
	In particular, $d \in A^{\J}$ by definition of $A^{\J}$.
	Thus, by hypothesis, $d \in A^{\I}$, and since $d \in \domain{\J'} = \domain{\I_\Pmc}$ we obtain $d \in A^{\I_\Pmc}$ by definition of $A^{\I_\Pmc}$.
	
	``$\Leftarrow$''.
	Let $A^{\J'} \subseteq A^{\I_\Pmc}$ and $d \in A^{\J}$; we need to show $d \in A^{\I}$.
	It is straightforward if $d \in \domain{\Jmc'}$.
	Otherwise, we know that $\refof{d} \in A^{\J'}$ by definition of $A^{\J}$.
	Therefore $\refof{d} \in A^{\I_\Pmc}$ by hypothesis, that is $A \in \typeinof{\I}{\refof{d}}$.
	Since $d$ and $\refof{d}$ have same type, it yields $A \in \typeinof{\I}{d}$, that is $d \in A^{\I}$.

	``$2 \Rightarrow 1$''. 
%	{\color{red} (Quentin: Spoiler alert, this is the very same proof as in Lemma~\ref{lemma-criteria-combined}.)}
	Assume $\I_\Pmc \models \Circ(\kb_\Pmc)$ for all $\Pmc \subseteq \domain{\I}$ s.t.\ $\sizeof{\Pmc} \leq 2\sizeof{\tbox} +1$.
	By hypothesis, we already have $\I \models \kb$.
	By contradiction, assume now there exists $\J < \I$.
	Based on $\J$, we build a subset $\Pmc \subseteq \domain{\J}$ containing:
	\begin{itemize}
		\item for each role $r$ s.t.\ $r^\J \neq \emptyset$, an element $w_r' \in (\exists r^-)^\J$;
		\item for each $A \in \Msf$ s.t.\ $A^\J \not\subseteq A^\I$, an element $e_A \in B^\J \setminus B^\I$ for some $B \prec A$ (Condition~3 in the definition of $\J <_\CP \I$ ensures existence of such $B$ and $e_A$);
		\item an element $e_\Msf \in A^\J \setminus A^\I$ for some $A \in \Msf$ s.t.\ $A^\J \subsetneq A^\I$ and for all $B \prec A$, $B^\J = B^\I$
		(Condition~4 in the definition of $<_\CP$ ensures the existence of such $A$ and $e_\Msf$).
	\end{itemize}
	Notice $\Pmc$ has size at most $2\sizeof{\tbox} +1$.
	We now build $\J'$ as:
	\begin{align*}
		\domain{\J'} = \; & \domain{\I_\Pmc}
		\\
		\cstyle{A}^{\J'} = \; & \cstyle{A}^{\J} \cap \domain{\J'}
		\\
		\rstyle{r}^{\J'} = \; & \{ (e, w_s') \mid e \in (\exists s)^\J  \cap \domain{\I_\Pmc}, \tbox \models s \incl r \}
		\\
		& \cup \{ (w_s', e) \mid e \in (\exists s)^\J  \cap \domain{\I_\Pmc}, \tbox \models s \incl r^- \}
	\end{align*}
%	It remains to verify $\J_\Pmc <_\CP \Imc_\Pmc$.
	It is easily verified that $\J'$ is a model of $\kb_\Pmc$, and we now prove $\J' <_\CP \I_\Pmc$, which will contradict $\I_\Pmc \models \Circ(\kb_\Pmc)$.
	%	We first notice a useful property: for all concept name $A$, we have $A^\J \cap (\domain{\I} \setminus \domain{\I_\Pmc}) \subseteq  A^\I \cap (\domain{\I} \setminus \domain{\I_\Pmc})$ ($\star$).
	%	Indeed, if $e \in A^\J \cap (\domain{\I} \setminus \domain{\I_\Pmc})$, then $A \in \ftypeinof{\I}{e}$, and therefore $e \in A^\I$.
	%	The converse does not holds in general.
	We now check that all four conditions from the definition of $<_\CP$ are satisfied:
	\begin{enumerate}
		\item 
		By definition, we have $\domain{\J'} = \domain{\I_\Pmc}$.
		\item 
		Let $A \in \Fsf$. Definitions of $\I_\Pmc$ and $\J'$ ensure $A^\I \cap {\domain{\I_\Pmc}} = A^{\I_\Pmc}$ and $A^\J \cap {\domain{\I_\Pmc}} = A^{\J'}$.
		From $\J <_\CP \I$, we get $A^{\I} = A^{\J}$, which thus yields $A^{\I_\Pmc} = A^{\J'}$.
		\item 
		Let $A \in \Msf$ such that $A^{\J'} \not\subseteq A^{\I_\Pmc}$.
		Therefore $A^{\J} \not\subseteq A^{\I}$, and recall we kept in $\Pmc$ an element $e_A \in B^\J \setminus B^\I$ for some $B \prec A$ to belong to $\Pmc$.
		Joint with $B^{\J'} \subseteq B^{\I_\Pmc}$ being trivial, $e_A$ additionally witnesses that $B^{\J'} \subsetneq B^{\I_\Pmc}$.
		\item
		Recall we kept in $\Pmc$ an element $e_\Msf \in A^\J \setminus A^\I$ for some $A \in \Msf$ s.t.\ $A^\J \subsetneq A^\I$ and for all $B \prec A$, $B^\J = B^\I$.
		It gives immediately that $A^{\J'} \subsetneq A^{\I_\Pmc}$ and for all $B \prec A$, $B^{\J'} = B^{\I_\Pmc}$.
	\end{enumerate}
	This proves $\J' <_\CP \I_\Pmc$, contradicting $\I_\Pmc \models \Circ(\kb_\Pmc)$ as desired.
      \end{proof}

\thmdataupperhornh*
\begin{proof}
	We exhibit an $\NPclass$ procedure to decide the complement of our problem, that is existence of a countermodel for UCQ $q$ over $\dlliteboolh$ cKB $\circkb$.
	Our procedure starts by guessing an interpretation $\I$ whose domain has size at most $|\Amc|+(2^{|\Tmc|+2}+1)^{3|q|}$.
	This can be done in linearly many non-deterministic steps (w.r.t.\ data complexity)
	It further checks whether $\I$ is a model of $\kb$ that does not entail $q$ and rejects otherwise.
	This can essentially be done naively in $\sizeof{\domain{\I}}^{\sizeof{\tbox}\sizeof{q}}$ deterministic steps, that is still polynomial
	% \textcolor{blue}{Really? Isn't it just polynomial?} 
	w.r.t.\ data complexity.
	The procedure finally checks whether $\I$ complies with $\CP$ by
	iterating over each $\Pmc$ with $\sizeof{\Pmc} \leq 2 \sizeof{\tbox} + 1$ and checking whether there exists a model $\J_\Pmc$ of $\kb$ s.t.\ $\J_\Pmc < \I_\Pmc$.
	If, for a choice of $\Pmc$ and we can find such a $\J_{\Pmc}$, then our procedure rejects.
	Notice that iterating over such $\Pmc$ can be done in $\sizeof{\domain{\I}}^{2 \sizeof{\tbox} + 1}$ iterations since we require $\sizeof{\Pmc} \leq 2 \sizeof{\tbox} + 1$.
	Computing $\I_\Pmc$ follows directly from the choice of $\Pmc$.
	Since each $\I_\Pmc$ has constant size w.r.t.\ data complexity, iterating over each possible $\J_\Pmc$ can be done naively with constantly many steps.
	Overall, the procedure uses a linear number of non-deterministic steps at the beginning and further performs several checks using a polynomial number of 
	%\textcolor{blue}{what about the deterministic steps that are linear/polynomial w.r.t.\ data complexity, e.g., the check whether \Imc is a model of \Kmc that does not entail $q$?} 
	additional deterministic steps.
	
	It remains to prove that an accepting run exists if there is a countermodel for $q$ over $\circkb$.
	If there exists an accepting run, then the corresponding guessed interpretation $\I$ is a model of $\kb$ that does not entail $q$, and the ``$2 \Rightarrow 1$'' direction from Lemma~\ref{lemma-criteria-data} ensures it also comply+ies with $\CP$.
	Conversely, if there exists a countermodel, then Lemma~\ref{lem-quotient} ensures existence of a countermodel $\I$ whose domain has size at most $|\Amc|+(2^{|\Tmc|+2}+1)^{3|q|}$.
	The procedure can guess this $\I$, and as \Imc is indeed a model of $\kb$ not entailing $q$, it will not be rejected.
	The ``$1 \Rightarrow 2$'' direction from Lemma~\ref{lemma-criteria-combined} further ensures $\I$ also passes the remaining checks performed by the procedure.
      \end{proof}

      \thmdatalowerdllitepos*

\begin{proof}
	\newcommand{\redge}{\mathsf{edge}}
	\newcommand{\cvertex}{\mathsf{Vertex}}
	\newcommand{\rhascol}{\mathsf{hasCol}}
	\newcommand{\ccolor}{\mathsf{Color}}
	We reduce the complement of the graph 3-colorability problem (3Col) to evaluating the Boolean CQ:
	\[
	q = \exists y_1 \, \exists y_2 \, \exists y ~ \redge(y_1, y_2) \land \rhascol(y_1, y) \land \rhascol(y_2, y)
	\]
	over the \dllitepos TBox:
	\[
	\tbox = \{ \cvertex \incl \exists \rhascol, \exists \rhascol^- \incl \ccolor \},
	\]
	where $\ccolor$ is minimized while all other predicates vary.
	Let $\CP$ be the resulting circumscription pattern.
	Given an instance $\graph = (\vertices, \edges)$ of 3Col, we build an ABox $\abox$ containing the following assertions:
	\begin{align}
		\cvertex(v) & \text{ for all } v \in \vertices
		\\
		\redge(v_1, v_2) & \text{ for all } \{v_1, v_2\} \in \edges
		\\
		\ccolor(c) & \text{ for all } c \in \{ r, g, b \}
	\end{align}
	We now prove the following claim:
	\[
	\graph \notin \text{3Col} \iff \circkb \models q
	\]
	First notice that every model $\I$ of $\circkb$ verifies $\ccolor^\I = \{ r, g, b \}$.
	Indeed, by contradiction, if $\I$ contains $e \in \ccolor^\I \setminus \{ r, g, b \}$, then we can build $\Jmc$ a model of $\kb$ with $\Jmc <_\CP \I$ by modifying $\I$ as follows:
	\begin{itemize}
		\item remove $e$ from $\ccolor^\I$, that is $\ccolor^\Jmc = \ccolor^\Imc \setminus \{ e \}$;
		\item reroute $\rhascol$ as: $\rhascol^\Jmc = \{ (v, r) \mid v \in (\exists \rhascol)^\I \}$.
	\end{itemize}
	It is then straightforward that $\Jmc$ satisfies the desired properties, contradicting $\I$ being a model of $\circkb$.
		
	``$\Rightarrow$''. Assume $\graph \notin \text{3Col}$ and consider a model $\I$ of $\Jmc$.
	By the above remark, we have $\ccolor^\I = \{ r, g, b \}$ and from $\I$ being a model of $\kb$, we can find a mapping $\tau : \vertices \rightarrow \{ r, g, b\}$ of $\graph$ such that for all $v \in \vertices$, if $\tau(v) = c$ then $(v, c) \in \rhascol^\I$.
	Since, by assumption, $\graph \notin \text{3Col}$, there exists an edge $\{ v_1, v_2 \} \in \edges$ such that $\tau(v_1) = \tau(v_2) = c$ for some $c \in \{ r, g, b \}$, which ensures $y_1 \mapsto v_1, y_2 \mapsto v_2, y \mapsto c$ is an homomorphism of $q$ in $\I$.
	
	``$\Leftarrow$''. Assume $\graph \in \text{3Col}$ and consider a 3-coloring $\tau : \vertices \rightarrow \{ r, g, b\}$.
	We build a model $\I_\tau$ of $\circkb$ by interpreting all concepts and roles as in $\abox$ except for $\rhascol$, which is interpreted as:
	\[
	\rhascol^{\I_\tau} = \{ (v, c) \mid v \in \vertices, \tau(v) = c \}.
	\]
	It is straightforward that $\I$ models $\circkb$ and does not embed $q$ (since $\tau$ is a 3-coloring).
      \end{proof}

\section{Proofs for Section~\ref{subsection-instance-alchi}}

We briefly discuss the variation of Proposition~\ref{prop:nonom} mentioned in the main part of the paper. 
Assume given a circumscribed $\mathcal{ALCHIO}$ KB $\circkb$ with $\kb = (\tbox, \abox)$, an AQ $A_0(x)$ and an individual $a_0 \in \mathsf{ind}(\mathcal{A})$.
We again replace all occurrences of a nominal $a$ with fresh concept $A_a$, add $A_a(a), B_a(a)$ to $\abox$, minimize $B_a$ and set $B_a \prec A$ for all $A \in \Msf$. 
However, in contrast with Proposition~\ref{prop:nonom}, we also add axioms $A_a \sqcap \neg B_a \sqsubseteq \exists r.(X \sqcap A_0)$ and $X \sqsubseteq Y$ to $\tbox$ for some fresh concept names $X$ and $Y$ and fresh role name $r$, and $Y(a_0)$ to $\abox$.
Finally, we also minimize $Y$ with higher preference than concepts from $\Msf$: We set $Y \prec A$ for all $A \in \Msf$.
Denoting $\mn{Circ}_{\CP'}(\kb')$ the resulting circumscribed \ALCHI KB, it can then be verified that 
	$\Circ(\Kmc) \models A_0(a_0)$ iff 
	$\mn{Circ}_{\mn{CP}'}(\Kmc') \models A_0(a_0)$.

We now move to a proof of Theorem~\ref{thm-combined-lower-el-aq}.

\thmcombinedlowerelaq*
\begin{proof}
Let $\mn{Circ}_\CP(\Kmc)$ be a circumscribed \ALC KB, with $\Kmc=(\Tmc,\Amc)$, $A_0$ an AQ, and $a_0 \in \Ind(\Amc)$.  We construct a
        circumscribed $\EL$ KB $\mn{Circ}_\CP(\Kmc')$, with
        $\Kmc'=(\Tmc',\Amc')$, such that
        $\mn{Circ}_\CP(\Kmc) \models A_0(a_0)$ iff $\mn{Circ}_\CP(\Kmc') \models A_0(a_0)$.

        With $\ELU_\bot$, we mean the extension of \EL with disjunction and $\bot$.
        It is well-known that every \ALC TBox $\Tmc$ can be rewritten in polynomial time into an $\ELU_\bot$ TBox $\Tmc^\ast$ that is a conservative extension of $\Tmc$ in the sense that every
        model of $\Tmc^\ast$ is a model of $\Tmc$ and every model of $\Tmc$ can be extended to a model of $\Tmc^\ast$ by interpreting the fresh concept and role names in $\Tmc^\ast$ \cite{DBLP:conf/ijcai/BaaderBL05}. It follows that $\mn{Circ}_\CP(\Kmc)
        \models A_0(a_0)$ iff $\mn{Circ}_\CP(\Tmc^\ast,\Amc) \models A_0(a_0)$, assuming that all the fresh concept names in $\Tmc^\ast$ vary in \CP.
        In the following, we recall the rewriting, which proceeds in three steps:
        \begin{enumerate}

        \item \emph{Remove value restrictions} by replacing every subconcept
          $\forall r . C$ with $\neg \exists r . \neg C$.

        \item \emph{Remove negation of compound concepts} by replacing
          every subconcept $\neg C$, with $C$ compound, by $\neg X$
          where $X$ is a fresh concept name, and adding the CIs
          $$
             C \sqsubseteq X \qquad X \sqsubseteq C.
          $$
          
        \item \emph{Remove negation entirely} by replacing every subconcept
          $\neg A$ with the fresh concept name $\overline A$, and adding
          the CIs
          $$
             \top  \sqsubseteq A \sqcup \overline{A} \qquad
             A \sqcap \overline{A} \sqsubseteq \bot.
          $$

        \end{enumerate}
        We may thus assume w.l.o.g.\ that the TBox \Tmc in the given circumscribed KB
        \Kmc is
        an $\ELU_\bot$ TBox. We may further assume that disjunction occurs in \Tmc
        only in CIs of the form
        $$
           B \sqsubseteq B_1 \sqcup B_2
        $$
        where $B,B_1,B_2$ are concept names, by replacing every disjunction
        $C_1 \sqcup C_2$ with a fresh concept name $X$ and adding the CIs
        $$
        \begin{array}{r@{\;}c@{\;}lcr@{\;}c@{\;}lcr@{\;}c@{\;}l}
          X &\sqsubseteq& Y_1 \sqcup Y_2 && Y_1 &\sqsubseteq& X &&
                                                                   Y_2 &\sqsubseteq& X \\[1mm]
          C_i & \sqsubseteq & Y_i && Y_i &\sqsubseteq& C_i && \text{for } i \in \{1,2\}
        \end{array}
        $$
        where also $Y_1,Y_2$ are fresh concept names. Finally, we may assume
        that \Tmc contains only a single CI $B \sqsubseteq B_1 \sqcup B_2$
        by replacing every such CI with
        $$
        B \sqsubseteq \exists r_{B_1,B_2} . D \quad
        \exists r_{B_1,B_2} . D_1 \sqsubseteq B_1 \quad 
        \exists r_{B_1,B_2} . D_2 \sqsubseteq B_2 
        $$
        where $r_{B_1,B_2}$ is a fresh role name and $D,D_1,D_2$ are fresh concept names,
        and adding the CI
        $$
            D \sqsubseteq D_1 \sqcup D_2.
        $$
        We may clearly also assume that $\bot$ occurs in \Tmc only in the form
        $C \sqsubseteq \bot$ with $C$ an \EL-concept.
        Note that the TBoxes resulting from these transformations are conservative
        extensions of the original ones. In \CP, all of the freshly introduced
        concept names vary.

        \smallskip
        We are now ready for the actual reduction, which combines ideas from
        the proofs of Theorems~\ref{thm:combined-lower-el} and~\ref{thm-data-lower-el}. To construct the TBox $\Tmc'$,
        We start with relativized versions of the \EL-CIs in \Tmc. 
        For an \EL
        concept $C$,
        inductively define the concept $C_\X$ as follows:
        \begin{align*}
                A_\X    & \coloneqq \X \sqcap A & (\exists r.D)_\X & \coloneqq \X \sqcap \exists r.D_\X \\
                \top_\X & \coloneqq \X          & (D \sqcap D')_\X & \coloneqq D_\X \sqcap D'_\X
        \end{align*}
        We then include in $\Tmc'$ all CIs 
        \begin{align}
                C_\X \sqsubseteq D_\X 
        \end{align}
        such that $C \sqsubseteq D \in \Tmc$ is neither the unique disjunctive
        CI $B \sqsubseteq B_1 \sqcup B_2$
        nor of the form $C \sqsubseteq \bot$. To construct the ABox $\Amc'$,
        we start with the extension of \Amc by
        \begin{align}
          X(a) \quad \text{ for all } a \in \Ind(\Amc).
          \label{Xmarking}
        \end{align}

        Of course, we need to compensate for removing the mentioned CIs.
        To simulate the disjunctive CI $B \sqsubseteq B_1 \sqcup B_2$, we
        extend $\Tmc'$ with
        \begin{align}
        B &\sqsubseteq \exists r_D . (D \sqcap \mn{Pos}) \qquad
            \exists r_D . D_1 \sqsubseteq B_1
            \label{blablaone}
          \\
                                                             B &\sqsubseteq \exists r_D . (D \sqcap \mn{Neg}) 
                                                          \qquad
                                                                 \exists r_D . D_2 \sqsubseteq B_2
                                                                 \label{blablatwo}
        \end{align}
        % \begin{array}{rclcrcl}
        % B &\sqsubseteq& \exists r_D . (D \sqcap \mn{Pos}) &&
        % \exists r_D . D_1 &\sqsubseteq& B_1 
        %   \\[1mm]
        %                                                      B &\sqsubseteq& \exists r_D . (D \sqcap \mn{Neg}) 
        %                                                   &&
        %                                                      \exists r_D . D_2 &\sqsubseteq& B_2
        % \end{array}
%        $$
        %
        where $D,D_1,D_2,\mn{Pos}$, and $\mn{Neg}$ are fresh concept names and $r_D$ is a fresh role name.
        We update \CP so that $D$ is minimized. We further extend \Amc with the
        assertions
\begin{align}
	D(d_1^+) 	& & D(d_1^-) 	& &D(d_2^+) 	& & D(d_2^-) \\
	D_1(d_1^+) 	& & D_1(d_1^-) 	& &
                                                            D_2(d_2^+)
                                                                                & & D_2(d_2^-)  	 \\
	\mn{Pos}(d_1^+) 	& & \mn{Neg}(d_1^-) 	& & \mn{Pos}(d_2^+) 	& &\mn{Neg}(d_2^-).
\end{align}
where $d^+_1,d^-_1,d^+_2,d^-_2$ are fresh individuals. Note that these individuals are \emph{not} marked with $X$, exempting them from $\Tmc$ is why the CIs from \Tmc are relativized in $\Tmc'$. Note that the way we simulate disjunction is similar to how we choose truth values in the proof of Theorem~\ref{thm-data-lower-el}, and also the reason for using a positive and a negative witness is the same.
We need to make sure that the positive and negative witnesses are distinct, which is achieved by otherwise making the query true.
%
% Further introduce fresh role names $\mn{freeze}$ %, $\mn{freeze}_{D_2}$,
% and \mn{checks} and for every $a \in \Ind(\Amc)$, fresh individuals $a_{D_1}$ and $a_{D_2}$.  Then extend $\Amc'$ with
% %
% $$
% \begin{array}{rcl}
%   \exists \mn{freeze}. D_1 \sqsubseteq D
% \end{array}
% $$
To this end, we introduce a fresh role name $u$ and fresh concept
names $G, A_0'$. We update \CP so that $G$ is minimized and extend $\Tmc'$ with:%
\begin{align}
	\mn{Pos} \sqcap \mn{Neg} & \sqsubseteq \exists u.(G \sqcap A'_0)
	\label{barlabel} \\
	A_0 &\sqsubseteq A'_0
	\label{barbarlabel}
\end{align}
We add
$
G(a_0)
$
to $\Amc'$ and the new query is $A'_0$.

To compensate for removing the CIs \mbox{$C \sqsubseteq \bot$}, we consider another fresh concept name $M$ and update \CP so that $M$ is minimized. We further extend $\Tmc'$ with
%
%$$
\begin{align}
	C \sqsubseteq M \sqcap \exists u . (G \sqcap A'_0) \quad \text{ for all } C \sqsubseteq \bot \in \Tmc.
	\label{lastone}
\end{align}
So if a concept $C$ with $C \sqsubseteq \bot \in \Tmc$ is satisfied, then we force the minimized concept name $M$ to be non-empty and make the (new) query true.

%\iffalse
%We introduce fresh a role name \mn{check} and extend $\Amc'$ with
%%
%\begin{align}
%  \mn{check}(a_0,a)  \qquad \text{for all } a \in \Ind(\Amc)
%  \label{foolabel}
%\end{align}
%%
%and $\Tmc'$ with
%%
%\begin{align}
%\exists \mn{check} . \exists r_D . (\mn{Pos} \sqcap \mn{Neg}) &\sqsubseteq A'_0
%  \label{barlabel} \\
%  A_0 &\sqsubseteq A'_0
%        \label{barbarlabel}
%\end{align}
%%
%where $A'_0$ is a fresh concept name that is the new query.
%
%
%Now for the compensation of the removal of the CIs \mbox{$C \sqsubseteq \bot$}. Let $u$ be a fresh role name and $G,M$ fresh concept names. We update \CP so that $G,M$ are both minimized and extend $\Tmc'$ with
%%
%%$$
%\begin{align}
%  C \sqsubseteq M \sqcap \exists u . (G \sqcap A'_0) \quad \text{ for all } C \sqsubseteq \bot \in \Tmc.
%  \label{lastone}
%\end{align}
%%$$
%%
%and add 
%%
%$
%G(a_0)
%$
%to $\Amc'$. So if a concept $C$ with $C \sqsubseteq \bot \in \Tmc$ is
%satisfied, then we force the minimized concept name $M$ to be non-empty
%and make the (new) query true.
%\fi
Let $\CP'$ be the extended circumscription pattern.
It remains to establish the correctness of the reduction.
        \\[2mm]
        {\bf Claim.} 
                $\Circ(\Kmc) \models A_0(a_0)$ iff $\Circ(\Kmc') \models A'_0(a_0)$.
                \\[2mm]
                To prepare for the proof of the claim, we first observe that every
                model \Imc of \Kmc gives rise to a model $\Imc'$ of $\Kmc'$
                in a natural way. More precisely, we set $\Delta^{\Imc'} = \Delta^\Imc \uplus \{ d^+_1,d^-_1,d^+_2,d^-_2\}$,
                define the extension of all concept and role names that occur in \Kmc
                exactly as in \Imc, and interpret the fresh concept and role names as
                follows:
                $$
                \begin{array}{rcl}
                  X^{\Imc'} &=& \Delta^\Imc \\[1mm]
                  D^{\Imc'} &=& \{ d^+_1,d^-_1,d^+_2,d^-_2\} \\[1mm]
                  D_i^{\Imc'}&=& \{d^+_i, d^-_i \} \text{ for } i \in \{1,2\} \\[1mm]
                  \mn{Pos}^{\Imc'} &=& \{ d^+_1,d^+_2 \}\\[1mm]
                  \mn{Neg}^{\Imc'} &=& \{ d^-_1,d^-_2 \}\\[1mm]
                  r_D^{\Imc'} &=& \{ (d,d^+_1),(d,d^-_1) \mid d \in (B \sqcap B_1)^\Imc \} \, \cup \\[1mm]
                         && \{ (d,d^+_2),(d,d^-_2) \mid d \in (B \sqcap B_2)^\Imc \} \\[0.5mm]
                  \mn{check}^{\Imc'} &=& \{ (a_0,a) \mid a \in \mn{ind}(\Amc) \\[1mm]
                  {A'_0}^{\Imc'} &=& A_0^\Imc \\[1mm]
                  u^{\Imc'} &=& \emptyset \\[1mm]
                  M^{\Imc'} &=& \emptyset \\[1mm]
                  G^{\Imc'} &=& \{ a_0 \}\\[1mm]
                \end{array}
                $$
                It is easily checked that ${\Imc'}$ is indeed a model of $\Kmc'$.
        Now for the actual proof of the claim
        \smallskip
                
        ``$\Leftarrow$''.  Assume that $\Circ(\Kmc) \not\models A_0(a_0)$. Then there is a model \Imc of \Kmc that is minimal w.r.t.\ \CP and satisfies $\Imc\not\models A_0(a_0)$. Let ${\Imc'}$ be the corresponding model of $\Kmc'$ defined above. We
                clearly have
            ${\Imc'} \not\models A'_0(a_0)$. To show that $\Circ(\Kmc') \not\models A'_0(a_0)$, it thus remains to show that $\Imc'$ is minimal w.r.t.\ $\CP'$.

            Assume to the contrary that there is a model $\Jmc' <_{\CP'} \Imc'$ of~$\Kmc'$.
            As $\Imc'$ interprets $D,M,$ and $G$ minimally among all models of $\Kmc'$,
            we must have $D^{\Jmc'} = D^{\Imc'} = \{ d^+_1,d^-_1,d^+_2,d^-_2\}$, $M^{\Jmc'} = \emptyset$, and
            $G^{\Jmc'} = G^{\Imc'} = \{ a_0 \}$. We show that the restriction $\Jmc$
            of $\Jmc'$ to domain $X^{\Jmc'}$ is a model
            of $\Kmc$. Moreover, $\Jmc' <_{\CP'} \Imc'$, $D^{\Jmc'} = D^{\Imc'}$, $M^{\Jmc'} = M^{\Imc'}$, and
            $G^{\Jmc'} = G^{\Imc'}$ imply $\Jmc <_\CP \Imc$, which then yields a contradiction against the minimality of \Imc.

            Based on the facts that $\Jmc'$ is a model of $\Amc'$, $\Ind(\Amc) \subseteq X^{\Jmc'}$ due to (\ref{Xmarking}), and $\Amc \subseteq \Amc'$, it is clear that $\Jmc$ is a model of \Amc. Moreover, since $\Jmc'$ is a model of $\Tmc'$, by
            construction of $\Jmc$ it is easy to see that $\Jmc$ satisfies all CIs in \Tmc
            with the possible
            exceptions of the disjunctive CI $B \sqsubseteq B_1 \sqcup B_2$ and the
            CIs of the form $C \sqsubseteq \bot$. The former, however, is satisfied due to
            CIs~(\ref{blablaone}) and~(\ref{blablatwo}) and since
            $D^{\Jmc'} = \{ d^+_1,d^-_1,d^+_2,d^-_2\}$. And the latter is satisfied
            due to the CIs~(\ref{lastone}) and since $M^{\Jmc'}=\emptyset$.
            
            %
            % Call an element $d \in \Delta^{\Jmc'}$ \emph{reachable} if there is a sequence
            % $d_0,r_0,d_1,r_1,\dots,r_{n-1},d_n$ such that $d_0 \in \Ind(\Amc)$, $(d_i,d_{i+1}) \in r^{\Jmc'}$ for $0 \leq i < n$, and $d_n=d$. We may assume w.l.o.g.\ that domain
            % elements in $\Jmc'$ that are not reachable do not occur in the extension of
            % concept and role names. NOT TRUE!!!!

\smallskip
            
``$\Rightarrow$''.  Assume that $\Circ(\Kmc') \not\models A'_0(a_0)$. Then there is a model $\Imc'$ of $\Kmc'$ that is minimal w.r.t.\ $\CP'$ and satisfies $\Imc'\not\models A'_0(a_0)$. 
We first argue that $G^{\Imc'}=\{ a_0 \}$ as, otherwise, we can find a model $\Jmc' <_{\CP'} \Imc'$ of~$\Kmc'$, contradicting the minimality of $\Imc'$.
We have $G^{\Imc'} \subseteq \{ a_0 \}$ since $\Imc'$ is a model of $\Amc'$. Assume to the contrary of what we want to show that the converse fails.  Then we construct $\Jmc'$ by modifying $\Imc'$ as follows:
\begin{itemize}
	
	\item set $G^{\Jmc'} = \{ a_0 \}$;
	
	\item add $a_0$ to ${A'_0}^{\Jmc'}$;
	
	\item reroute $u$ as $u^{\Jmc'} = \{ (e, a_0) \mid e \in (\exists u)^{\Imc'} \}$.
	
\end{itemize}
It is easy to see that, indeed, $\Jmc'$ is still a model of $\Kmc'$ and $\Jmc' <_{\CP'} \Imc'$.

Since $\I'$ satisfies CIs~(\ref{blablaone}) and~(\ref{blablatwo}), for every $e \in B^{\I'}$ we can choose two elements $e^+ \in (D \sqcap \mn{Pos})^{\Imc'}$ and $e^- \in (D \sqcap \mn{Neg})^{\Imc'}$ such that $(e,e^+), (e, e^-) \in r_D^{\I'}$. If $e^+ = e^-$ for some $e$, then by~(\ref{barlabel}) and $G^{\Imc'} = \{ a_0\}$, we have $a_0 \in A_0^{\Imc'}$,
which is impossible since $\Imc'\not\models A'_0(a_0)$. Thus  $e^+ \neq e^-$ for
all $e$.

We next argue that the following conditions are satisfied:
\begin{enumerate}

\item for all $e \in B^{\Imc'}$:
$\{ e^+, e^- \} \cap \{ d^+_1, d^-_1,d^+_2, d^-_2\}
\neq \emptyset$;

%\item $G^{\Imc'}=\{ a_0 \}$;

\item $M^{\Imc'}=\emptyset$.

\end{enumerate}
If, in fact, any of the above conditions are violated, then we can again find a model $\Jmc' <_{\CP'} \Imc'$ of~$\Kmc'$, contradicting the minimality of $\Imc'$.
We start with Condition~1.

Assume to the contrary that for some $e \in B^{\Imc'}$, $e^+, e^- \notin \{ d^+_1, d^-_1,d^+_2, d^-_2\}$.  Then we construct
$\Jmc'$ by modifying \Jmc as follows:
\begin{itemize}

\item remove $e^-$ from $D^{\Jmc'}$;

\item add $e^+$ to $\mn{Neg}^{\Jmc'}$;
  
\item add $a_0$ to ${A'_0}^{\Jmc'}$;

\item add $(e^+, a_0)$ to $u^{\Jmc'}$.

\end{itemize}
It is easy to see that, indeed, $\Jmc'$ is still a model of $\Kmc'$ and $\Jmc' <_{\CP'} \Imc'$.  

%Next for Condition~2. We have $G^{\Imc'} \subseteq \{ a_0 \}$ since $\Imc'$ is a model of $\Amc'$. Assume to the contrary of what we want to show that the converse fails.  Then we construct $\Jmc'$ by modifying \Jmc as follows:
%%
%\begin{itemize}
%
%\item set $G^{\Jmc'} = \{ a_0 \}$;
%
%\item add $a_0$ to ${A'_0}^{\Jmc'}$. 
%
%\end{itemize}
%%
%It is easy to see that, indeed, $\Jmc'$ is still a model of $\Kmc'$ and $\Jmc' <_{\CP'} \Imc'$.  

In the case of Condition~2, we can construct the model $\Jmc'$ simply as \Jmc modified by setting $M^{\Jmc'}=\emptyset$. The resulting $\Jmc'$ is a model of $\Kmc'$.  The CIs~(\ref{lastone}) are the only potentially problematic items. But since $\Imc'\not\models A'_0(a_0)$ and $G^{\Imc'}=\{a_0\}$, we can infer from~(\ref{lastone}) that $C^{\Imc'} = \emptyset$ for all $C \sqsubseteq \bot \in \Tmc$, and thus the same holds for $\Jmc'$. Consequently, the CIs~(\ref{lastone}) are never triggered in $\Jmc'$ and it is safe to set $M^{\Jmc'}=\emptyset$.

Let $\Imc$ be the restriction of $\Imc'$ to $X^{\Imc'}$. It can be verified that $\Imc'$ is a model of \Amc and that it satisfies all CIs in \Tmc
with the possible
            exceptions of the disjunctive CI $B \sqsubseteq B_1 \sqcup B_2$ and the
            CIs of the form $C \sqsubseteq \bot$. The former, however, is satisfied by
            Condition~1 and due to
            CIs~(\ref{blablaone}) and~(\ref{blablatwo}). And the latter is satisfied
            by Condition~2 and 
            due to CI~(\ref{lastone}).

            Since $\Imc' \not\models A'_0(a_0)$ and by (\ref{barbarlabel}), we have $\Imc \not\models A_0(a_0)$. To show that $\Kmc \not\models A_0(a_0)$, it thus remains
            to show that $\Imc$ is minimal w.r.t.\ $<_\CP$.
            Assume to the contrary that there is a model $\Jmc <_\CP \Imc$ of $\Kmc$
            and let $\Jmc'$ be the corresponding model of $\Kmc'$ constructed at
            the beginning of the correctness proof. Since $\Jmc'$ interprets
            the minimized concept names $D$, $M$, and $G$ in a minimal way among
            the models of $\Kmc'$, it follows from $\Jmc <_\CP \Imc$ that
            $\Jmc' <_{\CP'} \Imc'$, in contradiction to $\Imc'$ being minimal.
\end{proof}

\section{Proofs for Section~\ref{subsection-instance-dllite-combined}}

We now move to a proof of Theorem~\ref{thm-combined-lower-bool-instance}, which strongly combines \dllitebool expressiveness with fixed concept names.
Interestingly, fixed concept names are actually not needed.
Indeed, given a circumscribed $\dllitebool$ KB \circkb, each $A \in \Fsf$ can be replaced by the two minimized predicates $A$ and $\overline{A}$, where $\overline{A}$ is a fresh concept name set to be the complement of $A$ via the \dllitebool axioms $\overline{A} \incl \lnot A$ and $ \lnot A \incl \overline{A}$ that can be added in the TBox.
Concept names $A$ and $\overline{A}$ are then given higher preference than any other concept name from the original set of minimized concept names $\Msf$.
It is then straightforward to verify that the resulting circumscribed \dllitebool KB $\mn{Circ}_{\CP'}(\kb')$ has the same models as $\circkb$ (up to the interpretation of $\overline{A}$, which always equals the interpretation of $\lnot A$).

\thmcombinedlowerboolinstance*
\begin{proof}
	\newcommand{\ccenter}{\mathsf{Center}}
	\newcommand{\cbit}{\mathsf{Bit}}
	\newcommand{\cgoal}{\mathsf{Goal}}
	\newcommand{\callpairs}{\mathsf{AllPairs}}
	\newcommand{\cgoodcol}{\mathsf{GoodCol}}
	
	\newcommand{\cred}{\mathsf{R}}
	\newcommand{\cgreen}{\mathsf{G}}
	\newcommand{\cblue}{\mathsf{B}}
	\newcommand{\cgate}{G}
	\newcommand{\ctest}{\mathsf{T}}
	\newcommand{\istested}{\mathsf{Test}}

	The proof proceeds by reduction from the complement of the $\NExpTime$-complete \succinct\tcol\ problem. %, known to be $\NEXP$-complete due to \cite{papadimitriou-succinct}.
	An instance of \succinct\tcol\ consists of a Boolean circuit $\circuit$ with $2n$ input gates.
	The graph $\graph_\circuit$ encoded by $\circuit$ has $2^n$ vertices, identified by binary encodings on $n$ bits.
	Two vertices $u$ and $v$, with respective binary encodings $u_1 \dots u_n$ and $v_1 \dots v_n$, are adjacent in $\graph_\circuit$ iff $\circuit$ returns True when given as input $u_1 \dots u_n$ on its first $n$ gates and  $v_1 \dots v_n$ on the second half.
	The problem of deciding if $\graph_\circuit$ is 3-colorable has been proven to be $\NExpTime$-complete in \cite{Papadimitriou1986}.
	
	Let $\circuit$ be a Boolean circuit with $2n$ input gates.
	We build a \dllitebool cKB $\circkb$ with $\kb = (\tbox, \abox)$ s.t.\ the AQ $\cgoal(x)$ admits the individual $a$ as a certain answer iff $\circuit$ does not belong to \succinct\tcol.
	Let us already clarify that $\CP$ uses three minimized concept names, namely $\ccenter$, $\callpairs$ and $\cgoodcol$, with the following preference relation $\prec$:
	\begin{align}
		\ccenter \prec \callpairs \prec \cgoodcol
	\end{align}
	It also uses fixed concept names: each $\cbit_i$ for $1 \leq i \leq 2n$ and the six concept names $\cred_1$, $\cgreen_1$, $\cblue_1$, $\cred_2$, $\cgreen_2$ and $\cblue_2$, which will be useful to represent binary encodings and color assignments respectively.
	All other predicates vary.
	
	Models of $\kb$ contain a central element $a$, that we enforce via the ABox $\abox = \{ \ccenter(a) \}$ and which will be unique
%	, and we add the following axiom in $\tbox$:
%	\begin{align}
%		\ccenter \equiv \; & \lnot \cpair
%	\end{align}
	by virtue of the preference relation.
	This central element will further be used to detect undesired behaviors of the models via the AQ.
%	To this end, we ask $\ccenter$ to be a minimized concept.
%	Let us already clarify that our AQ consists of the concept $\cgoal$ and that we will check whether $\cgoal$ holds on $a$.	
	In a model, each element represents a pair $(v_1, v_2)$ of vertices by its combination of fixed concepts $\cbit_i$ with $1 \leq i \leq 2n$ that corresponds to the binary encodings of $v_1$ and $v_2$.
	To detect models that do not represent all possible pairs, we require each element representing a pair $(v_1, v_2)$ to ``send'' at the center a binary sequence of $2n$ bits that must be different from the encoding of $(v_1, v_2)$.
	This is achieved by the following axioms in $\tbox$:
	\begin{align}
		\top \incl \; & \exists r_i \sqcup \exists \overline{r_i}
		\quad \text{ for each } 1 \leq i \leq 2n
		\\
		\exists r_i^- \incl \; & \ccenter
		\qquad \text{ for each } 1 \leq i \leq 2n
		\\
		\exists \overline{r_i}^- \incl \; & \ccenter
		\qquad \text{ for each } 1 \leq i \leq 2n
		\\
		\top \incl \; & \bigsqcup_{0 \leq i \leq 2n} (\exists r_i \sqcap \lnot \cbit_i) \sqcup (\exists \overline{r_i} \sqcap \cbit_i)
		\label{eq:send-bits}
	\end{align}
	We now require the number of sent sequences to be unique, if possible, via the minimized concept name $\callpairs$, triggered by the following axioms in $\tbox$:
	\begin{align}
		\exists r_i^- \sqcap \exists \overline{r_i}^- \incl \; & \callpairs \quad \text{ for each } 1 \leq i \leq 2n
	\end{align}
	Therefore, if (at least) a pair is not represented in a model, then \emph{all} elements can send the binary encoding of a same missing pair to avoid instantiating $\callpairs$.
	If, on the other hand, each pair is represented (at least once), then the number of sent sequences cannot be unique, and $\callpairs$ must be satisfied on the central element $a$.
	To detect this with the AQ, we add the following axiom to $\tbox$:
	\begin{align}
		 \lnot\callpairs \incl \; & \cgoal
	\end{align}
	Now that we can detect whether all pairs are represented, we move to the encoding of colors.
	The respective color of $v_1$ and $v_2$ is chosen locally via the following axioms in $\tbox$:
	\begin{align}
		\top \incl \; & \cred_1 \sqcup \cgreen_1 \sqcup \cblue_1
		\label{eq:exists-color-1}
		\\
		\top \incl \; & \cred_2 \sqcup \cgreen_2 \sqcup \cblue_2
		\label{eq:exists-color-2}
	\end{align}
%	and each $v_1$, $v_2$ can only be assigned a single color via the following disjointness axioms in $\tbox$ (defined for $i = 1, 2$):
%	\begin{align}
%		\cred_i \sqcap \cgreen_i \incl \; & \bot 
%		&
%		\cgreen_i \sqcap \cblue_i \incl \; & \bot
%		&
%		\cblue_i \sqcap \cred_i \incl \; & \bot
%	\end{align}
	Recall concept names $\cred_1, \cgreen_1, \cblue_1$ and $\cred_2, \cgreen_2, \cblue_2$ are fixed.
	We additionally enforce that if an element represents a pair $(v_1, v_2)$ corresponding to an edge $\{ v_1, v_2 \}$ in $\graph_\circuit$, then it must assign different colors to $v_1$ and $v_2$.
	This is achieved by computing the output of $\circuit$ on input $v_1$ and $v_2$ via a fresh concept $\cgate$ for each gate $\cgate$ of $\circuit$ and adding the following axioms in $\tbox$:
	\begin{align}
		\cgate \equiv \; & \cbit_i \quad\qquad \text{ if } \cgate \text{ is the } i^{\text{th}} \text{ input gate of } \circuit
		\label{eq:consistent-circuits}
		\\
		\cgate \equiv \; & \cgate_1 \sqcap \cgate_2 \quad \text{ if } \cgate \text{ is a $\land$-gate with inputs } \cgate_1, \cgate_2
		\\
		\cgate \equiv \; & \cgate_1 \sqcup \cgate_2 \quad \text{ if } \cgate \text{ is a $\lor$-gate with inputs } \cgate_1, \cgate_2
		\\
		\cgate \equiv \; & \lnot \cgate' \quad\qquad \text{if } \cgate \text{ is a $\lnot$-gate with input } \cgate'
	\end{align}
	Assuming the output gate of $\circuit$ is $\cgate_{o}$, it now suffices to add the following axioms in $\tbox$:
	\begin{align}
		\cgate_{o} \sqcap \cred_1 \sqcap \cred_2 \incl \; & \bot
		\label{eq:consistent-edges-red}
		\\
		\cgate_{o} \sqcap \cgreen_1 \sqcap \cgreen_2 \incl \; & \bot
		\label{eq:consistent-edges-green}
		\\
		\cgate_{o} \sqcap \cblue_1 \sqcap \cblue_2 \incl \; & \bot
		\label{eq:consistent-edges-blue}
	\end{align}
	While the above allows ensuring that each element $e$ representing an edge $\{ v_1, v_2 \}$ assigns different colors to $v_1$ and $v_2$, there might still be inconsistent colorings in the sense that $v_1$ might have been assigned another color by some other element $e'$ representing an edge $\{ v_1, v_3 \}$.
	To detect such inconsistent colorings, the central element ``scans'' all colors assigned to a tested vertex, whose encoding corresponds to a binary sequence of $n$ bits represented by dedicated concepts $\ctest_i$.
	To do so, the interpretation of each $\ctest_i$ on the center element is first copied by all elements via the following axioms in $\tbox$, defined for each $1 \leq i \leq n$:
	\begin{align}
		\top \incl \; & \exists t_i \sqcup \exists \overline{t_i}
		\\
		\exists t_i^- \incl \; & \ccenter \sqcap \ctest_i
		&
		\exists \overline{t_i}^- \incl \; & \ccenter \sqcap \lnot \ctest_i
		\\
		\exists t_i \incl \; & \ctest_i
		&
		\exists \overline{t_i} \incl \; & \lnot\ctest_i
	\end{align}
	Each element representing a pair $(v_1, v_2)$ then compares whether the encoding of either $v_1$ or $v_2$ matches the sequence $\ctest_i$, via the following axioms:
	\begin{align}
		\bigsqcap_{1 \leq i \leq n} \left( (\cbit_i \sqcap \ctest_i) \sqcup (\lnot \cbit_i \sqcap \lnot \ctest_i) \right) \equiv \; & \istested_1
		\label{eq:test-1}
		\\
		\bigsqcap_{1 \leq i \leq n} \left( (\cbit_{n + i} \sqcap \ctest_i) \sqcup (\lnot \cbit_{n + i} \sqcap \lnot \ctest_i) \right) \equiv \; & \istested_2
	\end{align}
	It then sends the corresponding assigned color back to the central element via the following axioms in $\tbox$, defined for each $C \in \{ \cred, \cgreen, \cblue \}$:
	\begin{align}
	 	\istested_1 \sqcap C_1 \equiv \; & \exists s_C
	 	\\
	 	\istested_2 \sqcap C_2 \equiv \; & \exists s_C
	 	\\
	 	\exists s_C^- \incl \, & \ccenter
 	\end{align}
 	The center now detects whether it receives two different colors for the tested vertex:
 	\begin{align}
 		\bigsqcup_{\substack{ C, C' \in \{ \cred, \cgreen, \cblue \} \\ C \neq C'}} (\exists s_C^- \sqcap \exists s_{C'}^-) \equiv \; & \lnot \cgoodcol
% 		(\exists s_\cred^- \sqcap \exists s_\cblue^-) \sqcup (\exists s_\cblue^- \sqcap \exists s_\cgreen^-) \sqcup (\exists s_\cgreen^- \sqcap \exists s_\cred^-) \incl  \equiv \, & \lnot \cgoodcol
	\label{eq:inconsistent-coloring}
 	\end{align}
	where $\cgoodcol$ is a minimized concept name, which forces the center element to detect an inconsistent coloring if it exists. 
	This is further translated in terms of the AQ with:
	 	\begin{align}
		\lnot \cgoodcol \incl \; & \cgoal
		\label{eq:bad-color-gives-goal}
	\end{align}
 	
 	We are now done with the construction of $\circkb$.
	It remains to prove that:
	\[
	\circkb \models \cgoal(a) \iff \circuit \notin \succinct\tcol.
	\]
	
	``$\Rightarrow$''.
	Assume $\circuit \in \succinct\tcol$ and let $\rho : \{ 0, \dots, 2^n - 1 \} \rightarrow \{ \cred, \cgreen, \cblue \}$ be a (legal) 3-coloring of the encoded graph $\graph_\circuit$.
	We build a model $\I$ of $\circkb$ based on $\rho$, whose domain $\domain{\I}$ contains $a$ and one fresh element $e_{v_1, v_2}$ per $(v_1, v_2) \in \{ 0, \dots, 2^n - 1\} \times \{ 0, \dots, 2^n -1 \}$.
	Model $\I$ further interprets concept and role names as follows:
	\begin{align*}
		{\ccenter}^\I & = \cgoodcol^\I = \callpairs^\I = \{ a \}
		\\
		\cbit_i^\I & = \{ e_{v_1, v_2} \mid i^\text{th} \text{ bit in } (v_1, v_2) \text{ encoding is } 1 \}
		\\
		C_i^\I & = \{ e_{v_1, v_2} \mid \rho(v_i) = C \}
		\\
		G & = \{ e_{v_1, v_2 } \mid G \in \circuit \text{ evaluates to } 1 \text{ on input } (v_1, v_2) \}
		\\
		\istested_i & = \{ e_{v_1, v_2} \mid v_i = 0 \}
		\\	
		\cgoal^\I & = \ctest_i^\I = \emptyset
		\\	
		r_i^\I & = \{ (e_{v_1, v_2}, a) \mid i^\text{th} \text{ bit in } (v_1, v_2) \text{ encoding is } 0 \}
		\\	
		\overline{r_i}^\I & = \{ (e_{v_1, v_2}, a) \mid i^\text{th} \text{ bit in } (v_1, v_2) \text{ encoding is } 1 \}
		\\
		t_i^\I & = \emptyset
		\\
		\overline{t_i}^\I & = \{ (e_{v_1, v_2}, a) \mid 0 \leq v_1, v_2 \leq 2^n -1 \}
		\\
		\begin{split}
		s_C & = \{ (e_{v_1, v_2}, a) \mid \rho(0) = C \\
		&\phantom{= \{ (e_{v_1, v_2}, a) \mid }\text{ and either } v_1 = 0 \text{ or } v_2 = 0 \}
		\end{split}
	\end{align*}
	Notice that we have arbitrarily chosen each element representing a pair to send back to the center it's own encoding in which all bits have been flipped (see interpretations of roles $r_i$ and $\overline{r_i}$), and the tested vertex to be $0$ (interpretations of each $\ctest_i$ being empty and $t_i$, $\overline{t_i}$ and $\ctest_i$ being set accordingly).
	With the two above remarks, it is easily verified $\I$ models $\kb$, and, by definition $a \notin \cgoal^{\I}$.
	It remains to verify $\I$ complies with $\CP$.
	By contradiction, assume there exists $\J <_\CP \I$.
	Notice that from the fixed predicates, $\J$ still encodes one instance of each possible pair and the very same coloring $\rho$.
	From $\J$ being a model of $\abox$ , we have $a \in \ccenter^\J$.
	From $\ccenter^\I = \{ a \}$ and $\ccenter$ being the most preferred minimized predicate, it follows that $\ccenter^\J = \{ a\}$ as otherwise we would have $\I <_\CP \J$.
	Therefore, since each possible pair is represented at least once, the $r_i$ and $\overline{r_i}$ mechanism ensures $a \in \callpairs^\J$.
	Together with $\callpairs^\I = \{ a\}$ and $\callpairs$ being second most preferred minimized predicates, we obtain $\callpairs^\J = \{ a \}$ (as otherwise, again, we would have $\I <_\CP \J$).
	Finally, since the coloring encoded in $\J$ must be exactly $\rho$, whatever the interpretations of concepts $\ctest_i$, the concept $\exists s_{C}^- \sqcap \exists s_{C'}^-$ will always be empty for all $C, C' \in \{ \cred, \cgreen, \cblue \}$ s.t.\ $C \neq C'$.
	Therefore, $a \in \cgoodcol^\J$.
	Now, from $\cgoodcol$ being also minimized and $\cgoodcol^\I = \{ a \}$, we obtain $\cgoodcol^\J = \{ a\}$.
	Overall $\J$ interprets the minimized predicates as $\I$ does, hence the desired contradiction of $\J <_\CP \I$.
		
	``$\Leftarrow$''.
	Assume $\circuit \notin \succinct\tcol$.
	Consider a model $\I$ of $\circkb$.
	First notice that $\ccenter^\I = \{ a \}$.
	Indeed, $\I$ models $\abox$ hence $a \in \ccenter^\I$, and, if there were $b \in \ccenter^\I$ with $b \neq a$, then we could find a model $\J$ of $\kb$ with $\J <_\CP \I$ by:
	\begin{enumerate}
		\item take $\domain{\J} = \domain{\I}$ and preserve all interpretations of fixed concept names;
		\item setting $\ccenter^\J = \{ a \}$;
		\item replace every $(e, e') \in r_i^\I$ by $(e, a) \in r_i^\J$ and same for $\overline{r_i}$;
		\item define accordingly $\callpairs^\J$;
		\item set for all $e \in \domain{\J}$: $e\in \ctest_i^\J$ iff $a \in \ctest_i^\I$;
		\item set $t_i^\J = \{ (e, a) \mid e \in \ctest_i^\J \}$ and $\overline{t_i}^\J = \{ (e, a) \mid e \notin \ctest_i^\J \}$;
		\item define accordingly interpretations of concepts evaluating the circuit and $\istested_1^\J$, $\istested_2^\J$;
		\item set $s_C^\J = \{ (e, a) \mid e \in ((\istested_1 \sqcap C_1) \sqcup (\istested_2 \sqcap C_2))^\J \}$;
		\item define accordingly $\cgoodcol^\J$ and $\cgoal^\J$.
	\end{enumerate}
	In particular, notice Step~1 removes $b$ from the interpretation of $\ccenter$.
	
	We now want to prove that if a pair $(v_1, v_2)$ is not represented in $\I$, that is:
	\[
	\bigcap_{i \in \text{Ones}(v_1, v_2)} \cbit_i^\J \cap \bigcap_{i \in \text{Zeros}(v_1, v_2)} (\lnot \cbit_i)^\J = \emptyset,
	\]
	where $\text{Ones}(v_1, v_2)$ is the set of $0 \leq i \leq 2n -1$ s.t.\ the $i^\text{th}$ bit in the binary encoding of $(v_1, v_2)$ is $1$ and $\text{Zeros}(v_1, v_2)$ is its complement, then the query must be satisfied.
	Indeed, if such a $(v_1, v_2)$ exists, then we must have $\callpairs^\J = \emptyset$, thus $a \in \cgoal^\J$, as otherwise we can obtain a model $\J$ of $\kb$ s.t.\ $\J <_\CP \I$ by:
		\begin{enumerate}
		\item take $\domain{\J} = \domain{\I}$ and preserve all interpretations of fixed concept names and $\ccenter$;
		\item set $r_i^\J = \domain{\I} \times \{ a \}$ if $i \in \text{Ones}(v_1, v_2)$ and $r_i^\J = \emptyset$ otherwise; set $\overline{r_i}^\J = \domain{\I} \times \{ a \}$ if $i \in \text{Zeros}(v_1, v_2)$ and $\overline{r_i}^\J = \emptyset$ otherwise;
		\item follow steps 3 to 8 from the previous construction of $\J$.
	\end{enumerate}
	In particular, Step~2 of the above complies with Equation~\ref{eq:send-bits} as $(v_1, v_2)$ is not represented in $\I$.
	It further implies that $\callpairs^\J = \emptyset$, which ensures the desired contradiction $\J <_\CP \I$.
	
	We are thus left with the case in which each possible pair $(v_1, v_2)$ is represented at least once in $\I$.
	From Equations~\ref{eq:exists-color-1} and \ref{eq:exists-color-2}, we know each element representing a pair assigns colors to its $v_1$ and $v_2$.
	From Equations~\ref{eq:consistent-circuits} to \ref{eq:consistent-edges-blue}, these colors cannot be the same if there is an edge $\{ v_1, v_2 \}$ in the graph $\graph_\circuit$.
	Thus, since we assume $\circuit \notin \succinct\tcol$, the overall choices of colors cannot be consistent: there must exist a vertex $v_0$ which is assigned a color $C_1$ by an element $e_1$ representing a pair $p_1$ and a different color $C_2$ by an element $e_2$ representing a pair $p_2$.
	Let us assume $p_1$ has shape $(v_0, v_1)$ and $p_2$ has shape $(v_0, v_2)$ (other cases works similarly).
	We can now prove that $\cgoodcol^\I = \emptyset$, thus $a \in \cgoal$, as otherwise we could find a model $\J$ of $\kb$ with $\J <_\CP \I$ by:
	\begin{enumerate}
		\item take $\domain{\J} = \domain{\I}$ and preserve all interpretations of fixed concept names, of $\ccenter$ and $\callpairs$, and of roles $r_i$ and $\overline{r_i}$;
		\item set for all $e \in \domain{\J}$: $e \in \ctest_i^\J$ iff $i \in \text{Ones}(v_0)$;
		\item set $t_i^\J = \{ (e, a) \mid e \in \ctest_i^\J \}$ and $\overline{t_i}^\J = \{ (e, a) \mid e \notin \ctest_i^\J \}$;
		\item define accordingly interpretations of concepts evaluating the circuit and $\istested_1^\J$, $\istested_2^\J$;
		\item set $s_C^\J = \{ (e, a) \mid e \in ((\istested_1 \sqcap C_1) \sqcup (\istested_2 \sqcap C_2))^\J \}$;
		\item define accordingly $\cgoodcol^\J$ and $\cgoal^\J$.
	\end{enumerate}
	In particular, Equation~\ref{eq:test-1} and Step~4 in the above ensure $e_1, e_2 \in \istested_1^\J$.
	Therefore Step~5 above yields $(e_1, a) \in s_{C_1}^\J$ and $(e_2, a) \in s_{C_2}^\J$, which triggers Equation~\ref{eq:inconsistent-coloring} in Step~6 and ensures $\cgoodcol^\J = \emptyset$.
	This yields the desired contradiction $\J <_\CP \I$.
	Thus, $\cgoodcol^\I = \emptyset$, in particular Equation~\ref{eq:bad-color-gives-goal} yields $a \in \cgoal^\I$.

      \end{proof}

We work towards a proof of Theorem~\ref{thm-combined-upper-hornh-instance}.
Assume given a model $\I$ of a $\dllitehornh$ cKB $\circkb$.
We ``forget'' about some parts of $\I$, only retaining which roles may be needed due to a combination of fixed predicates in the forgotten part.
To  this end, we define the fixed-type $\ftypeinof{\I}{e}$ of an element $e \in \domain{\I}$ as the set of \dllite concepts $C$ such that $\tbox \models ( \bigsqcap_{e \in F^\I, \ F \in \Fsf} F ) \incl C$.
Given a role $r \in \posroles$, we say that $r$ is \emph{forced} in $\I$ if there exists an element $f_r \in \domain{\I}$ such that $\exists r \in \ftypeinof{\I}{f_r}$.
For each forced role in $\I$, we assume chosen such an element $f_r$.
Similarly, for each role $r \in \posroles$, we assume chosen an element $w_r \in (\exists r^-)^\I$ if $(\exists r^-)^\I \neq \emptyset$.
We now construct an interpretation ${\I_0}$ whose domain $\domain{\I_0}$ consists in $\indsof{\abox}$, all chosen $f_r$ and all chosen $w_r$.
The interpretation $\I_0$ is now defined as:
\begin{align*}
	\cstyle{A}^{\I_0} = \; & \cstyle{A}^{\I} \cap \domain{\I_0}
	\\
	\rstyle{r}^{\I_0} = \; & \rstyle{r}^{\I} \cap (\indsof{\abox} \times \indsof{\abox}) 
	\\
	& \cup \{ (e, w_s) \mid e \in (\exists s)^\I \cap \domain{\I_0}, \tbox \models s \incl r \}
	\\
	& \cup \{ (w_s, e) \mid e \in (\exists s)^\I \cap \domain{\I_0}, \tbox \models s \incl r^- \}
\end{align*}

\begin{remark}
	Notice $\I_0$ is a special case of the models $\I_\Pmc$ considered in Section~\ref{subsection-dllite-combined}, and that $\sizeof{\I_0} \leq \sizeof{\abox} + 2\sizeof{\tbox}$.
\end{remark}

The key result is now the following:

\begin{lemma}
	\label{lemma-linear-countermodel}
	Let $q$ be an AQ.
	If $\I$ is a countermodel for $q$ over $\circkb$, then so is $\I_0$.
\end{lemma}

\begin{proof}
	Assume $\I$ is a countermodel for $q$ over $\circkb$.
	Setting $\Pmc = \{ f_r \mid r \text{ is forced in } \I \}$, we have $\I_\Pmc = \I_0$ (see Section~\ref{subsection-dllite-combined}) and thus Lemma~\ref{lemma-portion-are-models} ensures $\I_0 \models \kb$.
	Since concept interpretations in $\I_0$ are inherited from $\I$, it is clear $\I_0$ does not entail $q$.
	It remains to prove $\I_0$ also complies with $\CP$.
	By contradiction assume there exists $\J_0$ a model of $\kb$ with $\J_0 <_\CP \I_0$.
	Notice that, for each forced role $r$ in $\I$, there must exists an element $w_r' \in (\exists r^-)^{\J_0}$ as we kept element $f_r \in \domain{\I_0}$ and $r$ is a consequence of the fixed predicates on $f_r$ that must have been preserved in $\J_0$ (see Condition~2 from the definition of $<_\CP$).
	We assume chosen such an element $w_r'$ per forced role and build an interpretation $\Jmc$:
	\begin{align*}
			\domain{\J} = \; & \domain{\I}
			\\
			\cstyle{A}^{\J} = \; & \cstyle{A}^{\J_0} \cup \{ e \in \domain{\I} \setminus \domain{\J_0} \mid A \in \ftypeinof{\I}{e} \}
			\\
			\rstyle{r}^{\J} = \; & \rstyle{r}^{\J_0} 
			\cup \left\{ (e, w_s') \; \middle| \begin{array}{l} e \in \domain{\I} \setminus \domain{\J_0} \\ \exists s \in \ftypeinof{\I}{e}, \tbox \models s \incl r \end{array} \right\}
			\\
			\; & \phantom{\rstyle{r}^{\J_0} } \cup \left\{ (w_s', e) \; \middle| \begin{array}{l} e \in \domain{\I} \setminus \domain{\J_0} \\ \exists s \in \ftypeinof{\I}{e}, \tbox \models s \incl r^- \end{array} \right\}
		\end{align*}
	It is easily verified that $\J$ is a model of $\kb$, and we now prove $\J <_\CP \I$, which will contradict $\I \models \circkb$.
	We first notice a useful property: for all concept name $A$, we have $A^\J \cap (\domain{\I} \setminus \domain{\I_0}) \subseteq  A^\I \cap (\domain{\I} \setminus \domain{\I_0})$ ($\star$).
	Indeed, if $e \in A^\J \cap (\domain{\I} \setminus \domain{\I_0})$, then $A \in \ftypeinof{\I}{e}$, and therefore $e \in A^\I$.
	The converse does not hold in general.
	We now check that all four conditions from the definition of $<_\CP$ are satisfied:
	\begin{enumerate}
			\item 
			By definition, we have $\domain{\J} = \domain{\I}$.
			\item 
			Let $A \in \Fsf$. Definitions of $\I_0$ and $\J$ ensure $A^\I \cap {\domain{\I_0}} = A^{\I_0}$ and $A^\J \cap {\domain{\I_0}} = A^{\J_0}$.
			From $\J_0 <_\CP \I_0$, we get $A^{\I_0} = A^{\J_0}$, which yields $A^\I \cap {\domain{\I_0}} = A^\J \cap {\domain{\I_0}}$.
			For an element $e \in \domain{\I} \setminus \domain{\I_0}$, we remark: $e \in A^\I$ iff $A \in \ftypeinof{\I}{e}$ iff $e \in A^\J$.
			Altogether, we obtain $A^\I = A^\J$.
			\item 
			Let $A \in \Msf$ such that $A^\J \not\subseteq A^\I$.
			Let thus $e \in A^\J \setminus A^\I$.
			Notice $e$ must belong to $\domain{\I_0}$, as otherwise $\star$ yields $e \in A^\I$.
			It follows that $e \in A^{\J_0} \not\subseteq A^{\I_0}$.
			Since $\J_0 <_\CP \I_0$, there exists $B \prec A$ s.t.\ $B^{\J_0} \subsetneq B^{\I_0}$.
			By $\star$, this extends into $B^{\J} \subsetneq B^{\I}$ and we found $B$ as desired.
			\item
			From $\J_0 <_\CP \I_0$, there exists $A \in \Msf$ s.t.\ $A^{\J_0} \subsetneq A^{\I_0}$ and for all $B \prec A$, $B^{\J_0} = B^{\I_0}$.
			Joint with $\star$, it follows that $A^{\J} \subsetneq A^{\I}$ and for all $B \prec A$, $B^{\J} \subseteq B^{\I}$.
			If ever there exists such a $B \prec A$, such that additionally $B^{\J} \subsetneq B^{\I}$, then we select a minimal such $B$ w.r.t.\ $\prec$, which provides the desired minimized concept.
			Otherwise, $A$ fits.
		\end{enumerate}
	It $\J <_\CP \I$, contradicting $\I \models \circkb$ as desired.
\end{proof}

\thmcombinedupperhornhinstance*
\begin{proof}
	Guess a candidate interpretation $\I$ with size $\sizeof{\abox} + 2\sizeof{\tbox}$.
	Check whether it is a model of $\kb$ and if the AQ of interest is \emph{not} satisfied in $\I$. 
	Using a $\NPclass$ oracle, check whether $\I$ is a model of $\circkb$.
	If all the above tests succeed, then accept; otherwise, reject.
	From Lemma~\ref{lemma-linear-countermodel}, it is immediate that there exists an accepting run if there exists a countermodel for the AQ over $\circkb$.
	Conversely, if a run accepts, then the guessed model $\I$ is a countermodel.
\end{proof}

%Before properly proving Lemma~\ref{lemma-data-indep}, we first highlight a useful property that allows to swap elements with same ABox types in a given interpretation.
% relies on the intuition that having kept (up to) $4^\sizeof{\tbox} +1$ witnesses for each ABox type is sufficient to faithfully capture every combinations any possible behavior (that is a realized type) of elements 

\lemmadataindep*

\begin{proof}
	\newcommand{\typeref}{\mathsf{ref}}
	``$\Rightarrow$''.
	Assume $\circkb \models A_0(a_0)$ and let $\I'$ be a model of $\Circ(\kb')$.
	
	We extend $\I'$ into an interpretation $\I$ whose domain is $\domain{\I} = \domain{\I'} \uplus (\indsof{\abox} \setminus \indsof{\abox'})$.
	To define a suitable interpretation of concepts on an individual $a$ from $\Delta = \indsof{\abox} \setminus \indsof{\abox'}$, we consider its ABox-type $t = \atypeinof{\abox}{a}$.
	Notice $m_{t} = 4^\sizeof{\tbox}$ as otherwise we would
        have $a \in  \indsof{\abox'}$.
	Consider now the types in $\I$ of elements $a_{t, 1}, \dots a_{t, 4^\sizeof{\tbox}}$.
	Since there are $4^\sizeof{\tbox}$ such elements for only $2^{\sizeof{\tbox}}$ possible types, there exists a type $t'$ realized in $\I$ at least $2^\sizeof{\tbox}$ times.
	We now chose an element $\typeref(t) \in \domain{\I'}$ s.t.\ $\atypeinof{\abox}{\typeref(t)} = t$ and $\typeinof{\I'}{\typeref(t)} = t'$.
	Such an element $\typeref(t)$ serves as a reference to interpret concepts and roles on individuals $a \in \Delta$ with ABox type $t$, as the following construction shows:
	\[
	\begin{array}{r@{\;}c@{\;}l}
		A^\I & = & A^{\I'} \; \cup \; \{ a \mid a \in \Delta, \typeref(\atypeinof{\abox}{a}) \in A^{\I'} \} 
		\smallskip \\
		p^\I & = & p^{\I'} \; \cup \; \{ (a, b) \mid \kb \models p(a, b) \}
		\smallskip \\
		& &  
		\cup \; \{ (a, e) \mid a \in \Delta, (\typeref(\atypeinof{\abox}{a}, e) \in p^{\I'} \}
		\smallskip \\
		& &
		\cup \; \{ (e, a) \mid a \in \Delta, (e, \typeref(\atypeinof{\abox}{a}) \in p^{\I'} \}.
	\end{array}
	\]
	It is easily verified that $\I$ is a model of $\kb$,
        particularly that it satisfies all role assertions from $\abox$. 
%	Furthermore, 
	We now prove $\I \models \circkb$, which, by hypothesis, gives $\I \models A_0(a_0)$, and thus $\I' \models A_0(a_0)$ by definition of $A_0^\I$.
	Assume by contradiction one can find a model $\J$ of $\kb$ s.t.\ $\J <_\CP \I$.
	We construct $\J' <_\CP \I'$ which will contradict $\I'$ being a model of $\Circ(\kb')$.
	Intuitively, we proceed as in Lemma~\ref{lem-lemma5} and simulate $\J$ in $\J'$.
	For each ABox type $t$ s.t.\ there exists $a \in \Delta$ with $\atypeinof{\abox}{a} = t$, we set:
	\begin{align*}
	D_t = & \; \{ d \in \domain{\I'} \mid \atypeinof{\abox}{d} = t, \atypeinof{\I'}{d} = \typeinof{\I'}{\typeref(t)} \}
	\smallskip \\
	S_t = & \; \{ \typeinof{\J}{d} \mid \atypeinof{\abox}{d} = t, \atypeinof{\I'}{d} = \typeinof{\I'}{\typeref(t)} \}
	\end{align*}
	From the definition of $\typeref(t)$, we have $\sizeof{D_t} \geq 2^\sizeof{\tbox}$, while, clearly, $\sizeof{S_t} \leq 2^\sizeof{\tbox}$.
	Since $S_t \neq \emptyset$ (it contains e.g.\ $\typeinof{\J}{\typeref(t)}$), we can find a surjective function $\pi_t : D_t \rightarrow S_t$.
	We consider $\pi$ the union of all such $\pi_t$, that is with $t$ s.t.\ there exists $a \in \Delta$ with $\atypeinof{\abox}{a} = t$.
	We further extend the domain of definition of $\pi$ to $\domain{\I'}$ by setting $\pi(d) = \typeinof{\J}{d}$ for the remaining elements of $\domain{\I'}$.
	We now define the interpretation $\J'$ as:
	\[
	\begin{array}{r@{\;}c@{\;}l}
		\domain{\J'} & = & \domain{\I'}
		\smallskip \\
		A^{\J'} & = & \{ d \in \domain{\I'} \mid A \in \pi(d) \} 
		\smallskip \\
		\rstyle{r}^{\J'}      & =	& \{ (d,e) \in \Delta^{\Imc'}\times \Delta^{\Imc'} \mid \pi(d) \rightsquigarrow_\rstyle{r} \pi(e) \}.
	\end{array}
	\]
	It can now be verified that $\J'$ is a model of $\kb'$ such that $\J' <_\CP \I'$.
%	In particular, for the latter, any minimization making $\J <_\CP \I$ that involve elements from $\Delta$ is now witnessed on some element from a corresponding $D_t$.
	
	 ``$\Leftarrow$''.
	 Assume $\Circ(\kb') \models A_0(a_0)$ and let $\I$ be a model of $\circkb$.
	 Here again, we denote $\Delta = \indsof{\abox} \setminus \indsof{\abox'}$.
	 By definition of $W$, all elements from $\Delta$ have an ABox type $t$ that is already realized at least $4^\sizeof{\tbox}$ times in $W$.
	 Therefore, we can define a permutation $\sigma$ on $\domain{\I}$ such that for all $d \in \domain{\I}$, the following conditions are respected:
	 \begin{enumerate}
	 	\item 
	 	$\sigma(a_0) = a_0$;
	 	\item 
	 	$\atypeinof{\abox}{\sigma(d)} = \atypeinof{\abox}{d}$;
	 	\item 
	 	If $d \in \Delta$, then there exists an element $\typeref(d) \in W$ with $\atypeinof{\abox}{\typeref(d)} = \atypeinof{\abox}{d}$ and $\typeinof{\I}{\typeref(d)} = \typeinof{\I}{d}$.
	 \end{enumerate} 
	 We can then define an interpretation $\I_\sigma$ as follows:
	 \[
	 \begin{array}{r@{\;}c@{\;}l}
	 	\domain{\I_\sigma} & = & \domain{\I}
	 	\smallskip \\
	 	A^{\I_\sigma} & = & \sigma(A^\I)
	 	\smallskip \\
	 	\rstyle{r}^{\I_\sigma}     & =	& \{ (d,e) \mid \kb \models r(d, e) \} \; \cup \; (\sigma \times \sigma)(r^\I).
	 \end{array}
	 \]
	 It is straightforward that $\I_\sigma$ models $\kb$ (notably relying on Condition~2), that preserves interpretation of concepts on the individual $a_0$ of interest (from Condition~1).
	 % TODO (from Robin): I do not understand the above sentence grammatically
	 Additionally, $\I_\sigma$ models $\circkb$ as otherwise a model $\J$ of $\kb$ with $\J <_\CP \I_\sigma$ immediately yields a model $\J_{\sigma^{-1}}$ of $\kb$ with $\J_{\sigma^{-1}} <_\CP \I$, contradicting $\I$ being a model of $\circkb$.
	 
	 We extend the mapping $\typeref$ from Condition~3 to the identity for elements from $\domain{\I} \setminus \Delta$, and define an interpretation $\I'$ as follows:
	\[
	\begin{array}{r@{\;}c@{\;}l}
		\domain{\I'} & = & \domain{\I} \setminus \Delta
		\smallskip \\
		A^{\I'} & = & A^{\I_\sigma} \cap \domain{\I'}
		\smallskip \\
		\rstyle{r}^{\I'}    & = & (\typeref \times \typeref)(r^{\I_\sigma} \cap (\domain{\I'} \times \domain{\I'})).
	\end{array}
	\]
	 It can be verified that $\I'$ is a model of $\kb'$.
	 We now prove it is also a model of $\Circ(\kb')$, which, by hypothesis, gives $\I' \models A_0(a_0)$, and thus $\I \models A_0(a_0)$ as unfolding definitions gives $a_0 \in A_0^\I$ iff $a_0 \in A_0^{\I_\sigma}$ iff $a_0 \in A_0^{\I'}$ (notably via Condition~1 on $\sigma$).
	 Assume by contradiction one can find a model $\J'$ of $\kb'$ with $\J' <_\CP \I'$.
	 We now construct $\J <_\CP \I$ which will contradict $\I$ being a model of $\circkb$.
	 Relying on the mapping $\typeref$, we set:
	 \[
	 \begin{array}{r@{\;}c@{\;}l}
	 	\domain{\J} & = & \domain{\I}
	 	\smallskip \\
	 	A^{\J} & = & \typeref^{-1}(A^{\J'})
	 	\smallskip \\
	 	\rstyle{r}^{\J}    & = & \{ (d,e) \mid \kb \models r(d, e) \} \; \cup \; (\typeref^{-1} \times \typeref^{-1})(r^{\J'}).
	 \end{array}
	 \]
	 It is easily checked that $\J$ models $\kb$.
	 From Condition~3 on $\sigma$, it then follows $\J <_\CP \I$, ie the desired contradiction.
\end{proof}

\section{Proofs for Section~\ref{subsection-negative-ri}}

\thmdatalowercoreh*
\begin{proof}
	
	\renewcommand{\cstyle}[1]{{\mathsf{#1}}}
	\renewcommand{\rstyle}[1]{{\mathsf{#1}}}
	\newcommand{\ixvar}{{x}} % individual x-variable
	\newcommand{\iyvar}{{y}} % individual y-variable
	\newcommand{\itrue}{t} % individual true
	\newcommand{\itrueof}[1]{\itrue_{#1}} % individual true of some variable
	\newcommand{\ifalse}{f}% individual false
	\newcommand{\ifalseof}[1]{\ifalse_{#1}} % individual false of some variable
	\newcommand{\iclause}{c} % individual clause
	
	\newcommand{\cxvar}{\cstyle{XVar}} % concept x variable
	\newcommand{\cyvar}{\cstyle{YVar}} % concept y variable
	\newcommand{\cclause}{\cstyle{Clause}} % concept clause
	\newcommand{\cformula}{\cstyle{Formula}} % concept formula
	
	\newcommand{\rxeval}{\rstyle{eval}_{\cstyle{X}}}
	\newcommand{\ryeval}{\rstyle{eval}_{\cstyle{Y}}}
	\newcommand{\rceval}{\rstyle{eval}_{\cstyle{C}}}
	\newcommand{\reval}{\rstyle{eval}}
	\newcommand{\rnegeval}{\overline{\reval}}
	
	\newcommand{\cxval}{\cstyle{XVal}}
	
	\newcommand{\ccval}{\cstyle{CVal}}
	
	\newcommand{\cvval}{\cstyle{VVal}}
	\newcommand{\cfval}{\cstyle{FVal}}
	
	\newcommand{\iformula}{f}
	\newcommand{\rfeval}{\rstyle{eval}_{\cstyle{F}}}
	
	\newcommand{\cgoal}{\cstyle{Goal}}

	We give a polynomial time reduction from
        $\forall\exists\mn{3SAT}$, c.f.\ the proof
        of Theorem~\ref{thm-data-lower-el}. Let a
        $\forall\exists$-3CNF sentence
        $\forall \bar x \exists \bar y \, \vp$ be given where
        $\bar x=x_1 \cdots x_m$, $\bar y = y_1 \cdots y_n$, and
        $\varphi=\bigwedge^\ell_{i=1} \bigvee_{j=1}^3 L_{ij}$ with
        $L_{ij} = v$ or $L_{ij} = \lnot{v}$ for some
        $v \in \{ x_1, \dots x_m, y_1, \dots, y_n \}$.  We construct a
        circumscribed \dllitecoreh KB $\circkb$ and an
        atomic query $\query$ such that $\circkb \models \query$ iff
        $\forall \bar x \exists \bar y \, \varphi$ is true.

        The circumscription pattern \CP involves four minimized
        concept names with the preference
        $$\cvval \prec \cxval \prec \ccval \prec \cfval,$$ and no
        fixed concept names. %  The
        % instance query is $$\query = \cgoal(\iformula).$$  
        We now
        describe the construction of the KB $\kb=(\Tmc,\Amc)$, not
        strictly
        separating \Tmc from \Amc. We first introduce an ABox
        individual for each variable, marking the existential
        variables
        with the concept name $\cxvar$ and the universal ones with
        $\cyvar$:
	\begin{align}
		\cxvar(\ixvar)
		& \quad \text{for all } x \in \bar x
		\label{eq:xvars} \\
		\cyvar(\iyvar)
		& \quad \text{for all } y \in \bar y.
		\label{eq:yvars}
	\end{align}
        To choose truth values for variables, we use the minimized concept name $\cvval$.
		We introduce two instances of $\cvval$ for each variable, one representing true and the other false:
        	\begin{align}
		\cvval(\itrueof{v})
		& \quad \text{for all } v \in \bar x \cup \bar y
		\label{eq:vvalstrue} \\
		\cvval(\ifalseof{v})
		& \quad \text{for all } v \in \bar x \cup \bar y.
		\label{eq:vvalsfalse}
	\end{align}
        Each variable must choose an instance of $\cvval$ via the role
        names $\rxeval$ an $\ryeval$, depending on whether it is
        existential
        or universal:
	\begin{align}
		\cxvar & \sqsubseteq \, \exists \rxeval
		\label{eq:xvariables_have_value} \\
		\cyvar & \sqsubseteq \, \exists \ryeval
		\label{eq:yvariables_have_value}\\
		\exists {\rxeval}^- & \sqsubseteq \, \cvval
		\label{eq:xvalues_are_vvalues} \\
		\exists {\ryeval}^- & \sqsubseteq \, \cvval.
		\label{eq:yvalues_are_vvalues}
	\end{align}
        There is no guarantee yet, however, that a variable $v$ chooses one of the instances $\itrueof{v}$ and $\ifalseof{v}$ of $\cvval$ reserved for it.
		To ensure this, we first install
        the following role inclusions:
		\begin{align}
		\rxeval  & \sqsubseteq \, \reval
		\label{eq:xeval_is_eval} \\
		\ryeval  & \sqsubseteq \, \reval
		\label{eq:yeval_is_eval} \\
		\reval & \sqsubseteq \, \lnot \rnegeval.
		\label{eq:eval_is_not_negeval}
	\end{align}
	The negative role inclusion allows us to flexibly control the targets for the existential restrictions in CIs~(\ref{eq:xvariables_have_value}) and~(\ref{eq:yvariables_have_value}), as follows:
	\begin{align}
		\rnegeval(v, \itrueof{v'})
		& \quad \text{for all } v, v' \in \bar x \cup \bar y
           \text{ with }  v \neq v'
		\label{eq:varblock} \\
		\rnegeval(v, \ifalseof{v'})
		& \quad \text{for all } v, v' \in \bar x \cup \bar y \text{ with }  v \neq v'.
		\label{eq:varblocktwo}
	\end{align}
	To force the truth values of the variables in $\bar x$ to be
        identical in all models that are smaller w.r.t.\
        `$<_\CP$,' we mark those truth values with the minimized
        concept name
        $\cxval$:
	\begin{align}
          \exists {\rxeval}^- & \sqsubseteq \, \cxval.
                                \label{eq:implxval}
	\end{align}
	We next introduce an individual for each clause:
	\begin{align}
		\cclause(\iclause_i)
		& \quad \text{for } 1 \leq i \leq \ell.
		\label{eq:clauses}
	\end{align}
	We also assign a truth value to every clause via the role name $\rceval$, another subrole of $\reval$.
	Every element with an incoming $\rceval$-edge must make the concept name $\ccval$ true, which is minimized, but with lower priority than $\cvval$ and $\cxval$.
	This reflects the fact that the truth values of variables determine the truth values of clauses. We put:
	\begin{align}
		\cclause & \sqsubseteq \, \exists \rceval
		\label{eq:clauses_have_value'} \\
		\rceval  & \sqsubseteq \, \reval
		\label{eq:ceval_is_eval} \\
		\exists {\rceval}^- & \sqsubseteq \, \ccval
		\label{eq:rceval_is_ccval}
	\end{align}
	The truth values of clauses are represented by the same
        individuals
        as the truth values of variables:
	\begin{align}
	\ccval(\itrueof{v})
	& \quad \text{for all } v \in \bar x \cup \bar y
	\label{eq:cvalstrue} \\
	\ccval(\ifalseof{v})
	& \quad \text{for all } v \in \bar x \cup \bar y
	\label{eq:vvalsfalse'} 
	\end{align}
	We again use the role $\rnegeval$ to control which instance of
        $\cclause$ can be used as truth values for which clause. This
        is based on the literals that occur in the clause.  If a
        variable $v$ occurs positively in the $i^{th}$ clause, then
        $\iclause_i$ has access to $\ifalseof{v}$, while if $v$ occurs
        negatively, then $\iclause_i$ has access to $\itrueof{v}$. And
        those are the only instances of $\cvval$ to which $\iclause_i$
        has access: for $1 \leq i \leq \ell$ and all $v \in \bar x
        \cup \bar y$,
        put
	\begin{align}
		\rnegeval(\iclause_i, \itrueof{v})
		& \quad \text{if } \lnot v \notin \{ L_{i, 1}, L_{i, 2}, L_{i, 3} \}
		\label{eq:clause_block_but_positive} \\
		\rnegeval(\iclause_i, \ifalseof{v})
		& \quad \text{if }  v \notin \{ L_{i, 1}, L_{i, 2}, L_{i, 3} \}.
		\label{eq:clause_block_but_negative}
	\end{align}
        Note that clause individual %$\itrueof{v}$, $\ifalseof{v}$
        % represents not only a truth value of variable $v$, but also a
        % literal for variable $v$. From this perspective, every
        $\iclause_i$ has access via $\rceval$ to $\itrueof{v}$ if
        making $v$ \emph{false} leads to satisfaction of the $i^{th}$
        clause, and likewise for $\ifalseof{v}$ and making $v$
        \emph{true}. Moreover, $v$ being made true is represented by
        an $\rxeval$- or $\ryeval$-edge from $v$ to $\itrueof{v}$ and
        likewise for $v$ being made false and $\ifalseof{v}$. Also
        recall that $\itrueof{v}$ and $\ifalseof{v}$ cannot have such
        incoming edges from elsewhere. Consequently, the $i^{th}$
        clause evaluates to true if we can find a target for the
        $\rceval$-edge that does \emph{not} have an incoming
        $\rxeval$- or $\ryeval$-edge:
	\begin{align}
		\exists {\rxeval}^- & \sqsubseteq \, \lnot \exists {\rceval}^-
		\label{eq:disjone} \\	
		\exists {\ryeval}^- & \sqsubseteq \, \lnot \exists {\rceval}^-.
		\label{eq:disjtwo}
	\end{align}
	In the case that a clause evaluates to false, it cannot reuse
        one of the admitted instances of $\ccval$. We introduce an
        extra instance $f$ of $\ccval$ that can be used instead:
		\begin{align}
		\ccval(\iformula).
		\label{eq:iformula_is_cval}
	\end{align}
	To ensure that $f$ is indeed used as an $\rceval$-target only if at least one clause is falsified, we use the fourth minimized concept name $\cfval$.
	Note that it is minimized with the least priority.
	We make sure that $f$ must have an
        outgoing $\rfeval$-edge leading to an instance of $\cfval$,
        that $f$ itself is an instance of $\cfval$, and that having an
        incoming $\rfeval$-edge precludes having an incoming
        $\rceval$-edge. If all clauses evaluate to true, then there is
        no need to use $f$ as a target for $\rceval$ and $f$ can use
        itself as the $\rfeval$-target. But if a clause evaluates to
        false, then we must use $f$ as a last resort $\rceval$-target
        and cannot use it as an $\rfeval$-target. Since $\cfval$ is
        minimized with least priority, the latter will simply lead to a fresh instance of $\rfeval$
       to be created. In summary, all clauses evaluate to true
        if and only of $f$ has an incoming $\rfeval$-edge.  We put:
	\begin{align}
		\cformula(\iformula)
%		\label{eq:iformula_is_formula}
%		\\
		& \qquad \cfval(\iformula)
		\label{eq:iformula_is_fval} \\
%	\end{align}
%	And axioms:
%	\begin{align}
		\cformula & \sqsubseteq \, \exists \rfeval
%		\label{eq:clauses_have_value'} 
		\\
		\exists {\rfeval}^- & \sqsubseteq \, \cfval
		\\
		\exists {\rceval}^- & \sqsubseteq \, \lnot \exists {\rfeval}^-.
		\label{eq:rcevalfcevaldisj}
	\end{align}
        By what was said above, to finish the reduction, it suffices to add
        \begin{align}
          \exists {\rfeval}^- & \sqsubseteq \, \cgoal.
	\end{align}
        to choose as the query $q=\cgoal(x)$, and to ask whether $f$ is an answer.

        To prove correctness, we thus have to show the following.
        \\[2mm]
        {\bf Claim.} $\circkb \models q(f)$ iff
        $\forall \bar x \exists \bar y \, \varphi$ is true.
        \\[2mm]
        To prepare for the proof of the claim, we first observe that
        every valuation $V$ for $\bar x \cup \bar y$ gives rise
        to a corresponding model $\Imc_V$ of \Kmc. We use domain 
        $$
          \Delta^{\Imc_V} = \Ind(\Amc) 
        $$
        and set
        $$
        A^{\Imc_V} = \{ a \mid A(a) \in \Amc \}
        $$
        for all concept names $$A \in \{ \cxvar, \cyvar, \cvval,
        \ccval, \cclause, \cformula \}.$$
        We interpret $\rxeval$ and $\ryeval$ according to $V$,
        that is
        $$
        \begin{array}{rcl}
          \rxeval^{\Imc_V} &=& \{ (x,\itrueof{v}) \mid x \in \bar x \text{
                           and }V(x)=1\} \,\cup\\[1mm]
                            && \{ (x,\ifalseof{v}) \mid x \in \bar x \text{
                           and }V(x)=0\} 
        \end{array}
        $$
        and analogously for $\ryeval$. Next we put
        $$
        \cxval^{\Imc_V} = \{ e \mid (e,d) \in \rxeval^{\Imc_V} \}.
        $$
        If $V$ makes the $i^{th}$ clause true, then there is a literal
        in it that is true. Choose such a literal $L$ and set
        $w_i = \itrueof{v}$ if $L=\neg v$ an $w_i = \ifalseof{v}$ if
        $L=v$. If $V$ makes the $i^{th}$ clause false, then set
        $w_i=f$. We proceed with the definition of $\Imc_V$:
        $$
        \begin{array}{rcl}
          \rceval^{\Imc_V} &=& \{ (c_i,w_i) \mid 1 \leq i \leq \ell \}
          \\[1mm]
          \reval^{\Imc_V} &=& \rxeval^{\Imc_V} \cup \ryeval^{\Imc_V} \cup
                          \rceval^{\Imc_V} \\[1mm]
          \rnegeval^{\Imc_V} &=& \{(a,b) \mid \rnegeval(a,b) \in \Amc \}
          \\[1mm]
          \cfval^{\Imc_V} &=& \{ f,c_1 \}  \\[1mm]
          \rfeval^{\Imc_V} &=& \{ (f,c_10) \} \\[1mm]
          \cgoal^{\Imc_V} &=& \{ c_1 \}.
        \end{array}
        $$
        The choice of $c_1$ is somewhat arbitrary in the last three
        statements, any other individual without an incoming
        $\rceval$-edge would also do.
        % $V$ also assigns a truth value
        % to each clause, let $V(c_i)$ denote the value of the $i^{th}$
        % clause.
        It is straightforward to verify that $\Imc_V$ is a model of
        \Kmc with $\Imc_V \not\models q(f)$.

        We can define a variation $\Imc'_V$ of $\Imc_V$ that is still
        a model of~\Kmc provided that all clauses are satisfied by $V$
        (which guarantees that $f$ has no incoming $\rceval$-edge), and
        that satisfies $\Imc'_V \models q(f)$. To achieve this, we
        replace the last three lines from the definition of $\Imc_V$
        with
        $$
        \begin{array}{rcl}
          \cfval^{\Imc_V} &=& \{ f \}  \\[1mm]
          \rfeval^{\Imc_V} &=& \{ (f,f) \} \\[1mm]
          \cgoal^{\Imc_V} &=& \{ f \}.
        \end{array}
        $$

        \medskip
        Now for the actual proof of the claim

        \smallskip
        
	``$\Rightarrow$''.  Assume that
        $\forall \bar x \exists \bar y \, \varphi$ is false, and thus
        $\exists \bar x \forall \bar y \, \lnot \varphi$ is true and
        there is a valuation $V_{\bar x}: \bar x \rightarrow \{0,1\}$
        such that $\forall \bar y \, \lnot \varphi'$ holds where
        $\varphi'$ is obtained from $\varphi$ by replacing every
        variable $x \in \bar x$ with the truth constant
        $V_{\bar x}(x)$. Consider any extension $V$ of $V_{\bar x}$ to
        the variables in $\bar y$ and the interpretation
        $\Imc_V$. Since $\Imc_V$ is a model of \Kmc with
        $\Imc_V \not\models q(f)$, to show that
        \mbox{$\circkb \not\models q(f)$} it remains to prove
        that there is no model $\Jmc <_\CP \I$ of \Kmc.

        Assume to the contrary that there is such a $\Jmc$. We first
        observe that $A^\Jmc=A^{\Imc_V}$ for all
        $A \in \{ \cvval, \cxval, \ccval \}$. This holds for $\cvval$
        since $\cvval^\Jmc \subsetneq \cvval^{\Imc_V}$ means that \Jmc
        does not satisfy \Amc, and likewise for $\ccval$. It also
        holds for $\cxval$ since every model of \Kmc must make
        $\cxval$ true at at least one of $\itrueof{x}$ and
        $\ifalseof{x}$ for all $x \in \bar x$. This is because of
        CIs~(\ref{eq:xvariables_have_value}),
        (\ref{eq:xvalues_are_vvalues}), (\ref{eq:xeval_is_eval}), and
        (\ref{eq:implxval}), the role
        disjointness~(\ref{eq:eval_is_not_negeval}), the
        assertions~(\ref{eq:varblock}) and~(\ref{eq:varblocktwo}), and
        the fact that minimization of $\cvval$ is preferred over
        minimization of $\cxval$.  But no subset of $\cxval^{\Imc_V}$
        satisfies this condition, so we must have  $\cxval^{\Imc_V}
        \subseteq \cxval^{\Jmc}$,
        consequently $\cxval^{\Jmc}=\cxval^{\Imc_V}$.

The above and $\Jmc <_\CP \I$ means that $\cfval^\Jmc \subsetneq
\cfval^{\Imc_V}$. Since \Jmc is a model of \Kmc, this implies $\cfval^\Jmc
= \{ f \}$.

Since $\cxval^\Jmc = \cxval^{\Imc_V}$ and \Jmc is a model of \Kmc,
$V(x)=1$ implies $(x,\itrueof{x}) \in \reval^\Jmc$ and $V(x)=0$
implies $(x,\ifalseof{x}) \in \reval^\Jmc$. Moreover, since
$\cvval^\Jmc = \cvval^{\Imc_V}$ and \Jmc is a model of \Kmc, for every
$y \in \bar y$ we have $(y,\itrueof{y}) \in \reval^\Jmc$ or
$(y,\ifalseof{y}) \in \reval^\Jmc$.  We thus find an extension $V'$ of
$V_{\bar x}$ to $\bar x \cup \bar y$ that is \emph{compatible with}
\Jmc in the sense that for all $v \in \bar x \cup \bar y$,
\begin{itemize}
\item 
$V'(v)=1$ implies $(v,\itrueof{v}) \in \reval^\Jmc$ and 
\item $V'(v)=0$ implies $(v,\ifalseof{v}) \in \reval^\Jmc$.
\end{itemize}
Choose some such $V'$. Since $\forall \bar y \, \lnot \varphi'$ holds,
at least one of the clauses must be made false by $V'$. As explained
alongside the construction of \Kmc, that clause can only have an
$\rceval$-edge to $f$. By~(\ref{eq:rcevalfcevaldisj}), the outgoing
$\rfeval$-edge from $f$ cannot end at $f$. But $\cfval^\Jmc = \{ f \}$
and thus~(\ref{eq:clauses_have_value'}) implies that $f$ is the only
point where that edge may end.  We have arrived at a contradiction.

\smallskip ``$\Leftarrow$''.  Assume that
$\forall \bar x \exists \bar y \, \varphi(\bar x, \bar y)$ is true and
let \Imc be a model of $\circkb$. We have to show that
$\Imc \models q(f)$.
To this end, we first observe that
\begin{equation*}
\cvval^\Imc = \{ a \mid \cvval(a) \in \Amc \}.
\tag{$*$}
\end{equation*}
If this is not the case, in fact, then we find a model
$\Jmc <_\CP \Imc$ of \Kmc, contradicting the minimality of \Jmc.
This model \Jmc is essentially $\Imc_V$, except that we might have to extend the domain with additional elements that do not occur in the extension of any concept or role name to make sure that the domains of \Imc and $\Imc_V$ are identical.

It follows from ($*$) and the fact that \Imc is a model of \Kmc that
for every $x \in \bar x$, we have $(x,\itrueof{x}) \in \reval^\Jmc$ or
$(x,\ifalseof{x}) \in \reval^\Jmc$.  Consequently, we find a valuation
$V_{\bar x}$ for $\bar x$ that is compatible with \Imc as defined in
the ``$\Rightarrow$'' direction of the proof. Since
$\forall \bar x \exists \bar y \, \varphi(\bar x, \bar y)$ is true, we
can extend $V_{\bar x}$ to a valuation $V$ for $\bar x \cup \bar y$
that satisfies $\varphi$. Consider the model $\Imc'_V$, extended to
domain $\Delta^\Imc$. By construction of $\Imc'_V$ and ($*$), we have
$\cvval^\Imc = \cvval^{\Imc'_V}$.
Using the facts that \Imc is a minimal model of \Kmc and the construction of $\Imc'_V$, it can now be observed that $\cxval^\Imc=\cxval^{\Imc'_V}$.
Moreover, by construction, $\Imc'_V$ interprets $\ccval$ and $\cfval$ in the minimal possible way among all models of \Kmc.
Since \Imc is a minimal
model, this implies $\ccval^\Imc=\ccval^{\Imc'_V}$ and
$\cfval^\Imc=\cfval^{\Imc'_V}$. In particular,
$\cfval^{\Imc}= \{ f \}$. But this implies $(f,f) \in \rfeval^\Imc$ as
all objects with an incoming $\rfeval$-edge must satisfy $\cfval$.  It
follows that $f \in \cgoal^\Imc$ and thus $\Imc \models q(f)$, as
desired.
\end{proof}
